# Supplementary material for: Flux: Liquid Types for Rust
Source: arXiv:2207.04034 source file (2022-11-14)
Supplement: Supplementary file 1 [file appendix.tex]

\section{Syntax of \corelan.}
\label{subsec:formalism:syntax}
\bpara{Syntax of Expressions}
{
\small
$$
\begin{array}{rrcll}
    \multicolumn{5}{c}{
        \aa,\lvar \in \mathit{RefineVar} \qquad \cloc \in \mathit{Loc} \qquad \xx, \ff \in \mathit{Var} \qquad t \in \mathit{Tag}
    }
    \\
    \syntaxcat{Expressions} &
    e & ::=
              & \blet{\xx}{e}{e}                                          & \textit{let-bind}       \\
      && \mid & \blet{\xx}{\new{\lvar}}{e}                                & \textit{let-alloc}       \\
      && \mid & \bif{\ee}{e}{e}                                           & \textit{if-then-else} \\
      && \mid & \eunpack{\xx}{\aa}{e}                                     & \textit{unpacking} \\
      && \mid & \fcall{e}{\overline{\typ}}{\overline{\expr}}{\overline{\aval}}  & \textit{function call} \\
      && \mid & \sassign{\place}{\ee}                                     & \textit{assignment} \\
      && \mid & \rvstrgref{\place} \mid \rvmutref{\place} \mid \rvshrref{\place} & \textit{(re)borrows} \\
      && \mid & \deref{\place}                                            & \textit{potinter dereference} \\
      && \mid & \xx                                                       & \textit{variables} \\
      && \mid & \val                                                      & \textit{values} \\

    \syntaxcat{Values} &
    \val & ::=
                    & \vrec{\ff}{\overline{\aa}}{\overline{\xx}}{{e}}   & \textit{(recursive) functions} \\
            && \mid & \ctrue \mid \cfalse               & \textit{booleans}  \\
            && \mid & 0, \pm 1, \dots                   & \textit{integers}  \\
            && \mid & \poison                           & \textit{uninitialized memory} \\
            && \mid & \vptr{\cloc}{\ptrtag}             & \textit{tagged pointers} \\
            && \mid & \vvec{n}{\val'}                   & \textit{vector values} \\
            && \mid & \vecnew                           & \textit{vector new}  \\
            && \mid & \vecpush                          & \textit{vector push} \\
            && \mid & \vecindexmut                      & \textit{vector mutable indexing} \\

      \syntaxcat{Logic} &
      \expr & ::= & \ctrue \mid \cfalse \mid 0, \pm 1, \dots & \textit{constants} \\
      && \mid & \aa \mid \expr = \expr & \textit{variables and equality} \\
      && \mid & \lnot \expr \mid \expr [\land,\vee] \expr \mid \expr [+, - , *] \expr  & \textit{bool and  arithmetic} \\
      && \mid & \cloc                                                             & \textit{locations} \\

    \syntaxcat{A-values} &
        \aval & ::=  & \val \mid \xx  \\

         \syntaxcat{Place} &
        \place & ::= & \xx \mid \vptr{\cloc}{\ptrtag} \\

    % \syntaxcat{Pointer Tag} &
    %     \ptrtag &  &
    \end{array}
$$
}

\bpara{Syntax of Types}
{
\small
\[
\begin{array}{rrcll}
    \syntaxcat{Types} &
        \typ & :=   & \rtyp{\tcon}{\expr}                      & \textit{indexed type} \\
            && \mid & \texists{\aa}{\rtyp{\tcon}{\aa}}{\expr}  & \textit{existential type} \\
            && \mid & \tptr{\loc}                              & \textit{pointer to location $\loc$}\\
            && \mid & \tbor{\lft}{\bormode}{\typ}              & \textit{borrowed reference (mutable or shared)}  \\
            && \mid & \uninit{n}                               & \textit{uninitialized memory of size $n$} \\
            && \mid & \polysig{\overline{\tvar}}
                              {\overline{\aa: \sort}}
                              {\expr}
                              {\loccx}
                              {\overline{\typ}}
                              {\typ}
                              {\loccx} \\
    \syntaxcat{Base Types} &
        \tcon & ::= & \tint  \mid \tbool \mid \tvec     & \textit{integers, booleans, and vectors} \\
    \syntaxcat{Modifier} &
        \bormode & ::=   & \mut \mid \shr  & \textit{mutable or shared} \\
    \syntaxcat{Locations} &
        \loc & := & \lvar \mid \cloc  & \textit{a concrete or abstract location}\\
    \syntaxcat{Sorts} &
        \sort  & := &  \sint \mid \sbool \mid \sloc \lftonly{\mid  \slft}\\

    \syntaxcat{Refinement contexts} &
        \varcx & :=   & \emptyset
                    \mid \varcx, \aa: \sort
                    \mid \varcx, \expr \\
    \syntaxcat{Location contexts} &
        \loccx & :=   & \emptyset \mid \loccx, \mapstoowned{\loc}{\typ} \\
    \syntaxcat{Value contexts} &
        \env & :=   & \emptyset \mid \env, \mapstoenv{\xx}{\typ} \\
    \syntaxcat{Dynamic Location contexts} &
        \dynenv & :=   & \emptyset \mid \dynenv, \mapstoowned{(\cloc,\ptrtag)}{\typ}
        %& \textit{Only references or pointer types.}\\
\end{array}
\]
}

\section{Auxiliary Definitions}

\subsection{Free Refinement Variables}
\[
\begin{array}{lcl}
    \text{\textbf{Expressions}} & & \\
     \fv{\blet{\xx}{e_1}{e_2}} & = & \fv{e_1} \cup \fv{e_2} \\
     \fv{\blet{\xx}{\new{\lvar}}{e}} & = & \fv{e} \setminus \{\lvar \}                                 \\
     \fv{\bif{\ee_1}{e_2}{e_3}} & = & \fv{e_1} \cup \fv{e_2} \cup \fv{e_3} \\
     \fv{\eunpack{\xx}{\aa}{e}} & = & \fv{e} \setminus \{\aa\} \\
     \fv{\fcall{e}{\overline{\typ}}{\overline{\expr}}{\overline{\aval}}} & = & \fv{e} \cup \bigcup_i \fv{\expr_i}\\
     \fv{\sassign{\place}{\ee}} & = & \fv{\ee} \\
     \fv{[\rvstrgref{\place}, \rvmutref{\place}, \rvshrref{\place}]} & = & \{\} \\
     \fv{\deref{\place}}  & = & \{\}\\
     \fv{\xx} & = & \{\} \\
     \fv{\vrec{\ff}{\overline{\aa}}{\overline{\xx}}{{e}}}  & =& \fv{e} \setminus \{\overline{\aa}\}\\
     \fv{[\ctrue, \cfalse]} & = & \{\} \\
     \fv{0, \pm 1, \dots}  & = & \{\} \\
     \fv{\poison} & = & \{\}\\
     \fv{\vptr{\cloc}{\ptrtag}} & = & \{\} \\
     \fv{\vvec{n}{\val}} & = & \fv{\val} \\[0.5em]

    \text{\textbf{Types}} & & \\
    \fv{\rtyp{\tcon}{\expr}} & = & \fv{\expr}\\
    \fv{\texists{\aa}{\rtyp{\tcon}{\aa}}{\expr}} & = & \fv{\expr} \setminus \{\aa\} \\
    \fv{\tptr{\loc}} & = & \fv{\loc}\\
    \fv{\tbor{\lft}{\bormode}{\typ}} & = & \fv{\typ}\\
    \fv{\uninit{n}} & = & \{\}\\
    \fv{\polysig{\overline{\tvar}}
    {{\overline{\aa: \sort}}}
    {{\expr}}
    {\loccx_i}
    {\overline{\typ}}
    {\typ_o}
    {\loccx_o}} & = & (\fv{\expr} \cup \fv{\loccx_i} \bigcup_i \fv{\typ_i} \cup \fv{\typ_o} \cup \fv{\loccx_o}) \setminus \{\overline{\aa}\}\\[0.5em]

    \text{\textbf{Refinements}} & & \\
    \fv{\aa}& = & \{\aa\} \\
    \fv{\expr_1 [=, \land, +, - , *] \expr_2}& = & \fv{\expr_1}\cup \fv{\expr_2} \\
    \fv{\lnot \expr}& = & \fv{\expr} \\
    \fv{[\ctrue,\cfalse,\cloc]}  &=& \{\} \\
    \fv{n}       &=& \{\} \quad n \in \mathbb{Z}\\[0.5em]

    \text{\textbf{Location Contexts}} & & \\
    \fv{\emptyset} & = & \emptyset \\
    \fv{\loccx, \mapstoowned{\loc}{\typ}} & = & \fv{\loccx} \cup \fv{\typ} \cup \fv{\loc} \\[0.5em]

    \text{\textbf{Value Contexts}} & & \\
    \fv{\emptyset} & = & \emptyset \\
    \fv{\env, \mapstoenv{\xx}{\typ}} & = & \fv{\env} \cup \fv{\typ} \\[0.5em]

    \text{\textbf{Dynamic Location Contexts}} & & \\
    \fv{\emptyset} & = & \emptyset \\
    \fv{\dynenv, \mapstoowned{(\cloc,\ptrtag)}{\typ}} & = & \fv{\dynenv} \cup \fv{\typ} \\
\end{array}
\]
\clearpage

\subsection{Type Substitution}
$$
\begin{array}{lcl}
    \text{\textbf{Types}} & & \\
    {\rtyp{\tcon}{\expr}}\subst{\aa}{\expr_\aa} & = & \rtyp{\tcon}{\expr\subst{\aa}{\expr_\aa}}\\
    {\texists{\bb}{\rtyp{\tcon}{\bb}}{\expr}}\subst{\aa}{\expr_\aa} & = & \left\{\begin{array}{ll}
        \texists{\bb}{\rtyp{\tcon}{\bb}}{\expr}, & \text{if } \bb = \aa\\
        \texists{\bb}{\rtyp{\tcon}{\bb}}{\expr\subst{\aa}{\expr_\aa}}, & \text{otherwise }
        \end{array}\right.\\
    {\tptr{\loc}}\subst{\aa}{\expr_\aa} & =  & \left\{\begin{array}{ll}
        \tptr{\expr_\aa}, & \text{if } \aa = \loc\\
        \tptr{\loc}, & \text{otherwise }
        \end{array}\right.\\
    ({\tbor{\lft}{\bormode}{\typ}})\subst{\aa}{\expr_\aa} & = & {\tbor{\lft}{\bormode}{\typ\subst{\aa}{\expr_\aa}}}\\
    {\uninit{n}}\subst{\aa}{\expr_\aa} & = & \uninit{n}\\
    ({\polysig{\overline{\tvar}}
    {{\overline{\aa: \sort}}}
    {{\expr}}
    {\loccx_i}
    {\overline{\typ}}
    {\typ_o}
    {\loccx_o}})\subst{\aa}{\expr_\aa} & = & \left\{\begin{array}{ll}
                \polysig{\overline{\tvar}}
            {{\overline{\aa: \sort}}}
            {{\expr}}
            {\loccx_i}
            {\overline{\typ}}
            {\typ_o}
            {\loccx_o} & \text{if } \aa \in \{\overline{\aa}\}\\

            \polysig{\overline{\tvar}}
            {{\overline{\aa: \sort}}}
            {{\expr\subst{\aa}{\expr_\aa}}}
            {\loccx_i\subst{\aa}{\expr_\aa}}
            {\overline{\typ\subst{\aa}{\expr_\aa}}}
            {\\ \quad\quad\quad\typ_o\subst{\aa}{\expr_\aa}}
            {\loccx_o\subst{\aa}{\expr_\aa}}, & \text{otherwise }
        \end{array}\right.\\[0.5em]

    \text{\textbf{Logical Expressions}} & & \\
    {\bb}\subst{\aa}{\expr_\aa}& = & \left\{\begin{array}{ll}
        \expr_\aa, & \text{if } \aa = \bb\\
        \bb, & \text{otherwise }
        \end{array}\right. \\
    {(\expr_1 [=, \land, +, - , *] \expr_2)}\subst{\aa}{\expr_\aa}& = & \expr_1\subst{\aa}{\expr_\aa} [=, \land, +, - , *] \expr_2\subst{\aa}{\expr_\aa} \\
    {(\lnot \expr)}\subst{\aa}{\expr_\aa}& = & \lnot \expr\subst{\aa}{\expr_\aa} \\
    {n}\subst{\aa}{\expr_\aa}& = & n \quad n \in \mathbb{Z} \\
    {\cloc}\subst{\aa}{\expr_\aa}& = & \cloc \\
    {\ctrue}\subst{\aa}{\expr_\aa}& = & \ctrue \\
    {\cfalse}\subst{\aa}{\expr_\aa}& = & \cfalse \\[0.5em]

    \text{\textbf{Location Contexts}} & & \\
    {\emptyset}\subst{\aa}{\expr_\aa} & = & \emptyset \\
    {(\loccx, \mapstoowned{\loc}{\typ})}\subst{\aa}{\expr_\aa} & = &
    \loccx\subst{\aa}{\expr_\aa}, \mapstoowned{\loc\subst{\aa}{\expr_\aa}}{\typ\subst{\aa}{\expr_\aa}} \\[0.5em]

    \text{\textbf{Value Contexts}} & & \\
    {\emptyset}\subst{\aa}{\expr_\aa} & = & \emptyset \\
    {(\env, \mapstoenv{\xx}{\typ})}\subst{\aa}{\expr_\aa} & = &
    \env\subst{\aa}{\expr_\aa}, \mapstoenv{\xx}{\typ\subst{\aa}{\expr_\aa}} \\[1em]

    \text{\textbf{Dynamic Location Contexts}} & & \\
    {\emptyset}\subst{\aa}{\expr_\aa} & = & \emptyset \\
    {(\dynenv, \mapstoowned{(\cloc,\ptrtag)}{\typ})}\subst{\aa}{\expr_\aa} & = &
    \dynenv\subst{\aa}{\expr_\aa}, \mapstoowned{(\cloc,\ptrtag)}{\typ\subst{\aa}{\expr_\aa}} \\[0.5em]

    \text{\textbf{Refinement Contexts}} & & \\
    {\emptyset}\subst{\aa}{\expr_\aa} & = & \emptyset \\
    {(\varcx, \aa': \sort)}\subst{\aa}{\expr_\aa} & = &
        \varcx\subst{\aa}{\expr_\aa}, \aa': \sort \text{, if } \aa \not= \aa' \\
    {(\varcx, \expr)}\subst{\aa}{\expr_\aa} & = & \varcx\subst{\aa}{\expr_\aa}, \expr\subst{\aa}{\expr_\aa} \\
\end{array}
$$
\clearpage

\subsection{Expression Substitution (values)}
$$
\begin{array}{lcl}
    (\eunpack{\xx}{\aa}{\ee})\subst{\yy}{\val_\yy} & = & \left\{\begin{array}{ll}
        \ee\subst{\yy}{\val_\yy}\subst{\aa}{\interp{\val_\yy}}, & \text{if } \xx = \yy\\
        \eunpack{\xx}{\aa}{\ee}\subst{\yy}{\val_\yy}, & \text{otherwise }
        \end{array}\right.\\
    (\blet{\xx}{\ee_\xx}{\ee})\subst{\yy}{\val_\yy} & = & \left\{\begin{array}{ll}
        \blet{\xx}{\ee_\xx\subst{\yy}{\val_\yy}}{\ee}, & \text{if } \xx = \yy\\
        \blet{\xx}{\ee_\xx\subst{\yy}{\val_\yy}}{\ee\subst{\yy}{\val_\yy}}, & \text{otherwise }
        \end{array}\right.\\
    (\blet{\xx}{\new{\lvar}}{\ee})\subst{\yy}{\val_\yy} & = & \left\{\begin{array}{ll}
        \blet{\xx}{\new{\lvar}}{\ee}, & \text{if } \xx = \yy\\
        \blet{\xx}{\new{\lvar}}{\ee\subst{\yy}{\val_\yy}}, & \text{otherwise }
        \end{array}\right.\\
        \xx\subst{\yy}{\val_\yy} & = & \left\{\begin{array}{ll}
            \val_\yy, & \text{if } \xx = \yy\\
            \xx, & \text{otherwise }
            \end{array}\right.\\
        (\bif{\ee}{\ee_1}{\ee_2})\subst{\yy}{\val_\yy} & = &
    \bif{\ee\subst{\yy}{\val_\yy}}{\ee_1\subst{\yy}{\val_\yy}}{\ee_2\subst{\yy}{\val_\yy}} \\
    (\bseq{\stmt}{\ee})\subst{\yy}{\val_\yy} & = &
    \bseq{\stmt\subst{\yy}{\val_\yy}}{\ee\subst{\yy}{\val_\yy}}\\
    (\fcall{e}{\overline{\typ}}{\overline{\expr}}{\overline{\aval}})\subst{\yy}{\val_\yy} & = &
    \fcall{e\subst{\yy}{\val_\yy}}{\overline{\typ}}{\overline{\expr}}{\overline{\aval\subst{\yy}{\val_\yy}}}\\

    % \text{\textbf{Value Substitution}} & & \\
    (\vrec{\ff}{\overline{\aa}}{\overline{\xx}}{{e}})\subst{\yy}{\val_\yy} & = & \left\{\begin{array}{ll}
        \vrec{\ff}{\overline{\aa}}{\overline{\xx}}{\ee\subst{\yy}{\val_\yy}}, & \text{if } \yy \not = \ff \text{ and } \yy \not = \xx_i\\
        \vrec{\ff}{\overline{\aa}}{\overline{\xx}}{\ee}, & \text{otherwise }
        \end{array}\right.
    \\
    \val\subst{\yy}{\val_\yy} & = & \val \\

    % \text{\textbf{Statement Substitution}} & & \\

    \sassign{\place}{\rval}\subst{\yy}{\val_\yy} & = &
    \sassign{\place\subst{\yy}{\val_\yy}}{\rval\subst{\yy}{\val_\yy}}
    \\
    % \sskip\subst{\yy}{\val_\yy} & = & \sskip \\

    % \text{\textbf{R-Value Substitution}} & & \\

    % \val\subst{\yy}{\val_\yy} & = & \val\subst{\yy}{\val_\yy}\\
    (\rvstrgref{\place}) \subst{\yy}{\val_\yy} & = & \rvstrgref{\place\subst{\yy}{\val_\yy}} \\

    (\rvmutref{\place}) \subst{\yy}{\val_\yy} & = & \rvmutref{\place\subst{\yy}{\val_\yy}} \\

    (\rvshrref{\place}) \subst{\yy}{\val_\yy} & = & \rvshrref{\place\subst{\yy}{\val_\yy}} \\

    (\deref{\place}) \subst{\yy}{\val_\yy} & = & \deref{\place\subst{\yy}{\val_\yy}} \\
\end{array}
$$

\subsection{Expressions Substitution (refinements)}
$$
\begin{array}{lcl}
    (\eunpack{\xx}{\bb}{\ee})\subst{\aa}{\expr_\aa} & = & \left\{\begin{array}{ll}
        \eunpack{\xx}{\bb}{\ee\subst{\aa}{\val_\aa}}, & \text{if } \aa \neq \bb \\
        \eunpack{\xx}{\bb}{\ee} & \text{otherwise }
        \end{array}\right.\\

    (\blet{\xx}{\ee_\xx}{\ee})\subst{\aa}{\expr_\aa} & = & \blet{\xx}{\ee_\xx\subst{\aa}{\expr_\aa}}{\ee\subst{\aa}{\expr_\aa}} \\

    (\blet{\xx}{\new{\lvar}}{\ee})\subst{\aa}{\expr_\aa} & = & \left\{\begin{array}{ll}
        \blet{\xx}{\new{\lvar}}{\ee\subst{\aa}{\expr_\aa}}, & \text{if } \aa \neq \lvar \\
        \blet{\xx}{\new{\lvar}}{\ee\subst{\aa}{\expr_\aa}}, & \text{otherwise} \\
        \end{array}\right.\\

    \xx\subst{\aa}{\expr_\aa} & = & \xx \\

    (\bif{\ee}{\ee_1}{\ee_2})\subst{\aa}{\expr_\aa} & = &
    \bif{\ee\subst{\aa}{\expr_\aa}}{\ee_1\subst{\aa}{\expr_\aa}}{\ee_2\subst{\aa}{\expr_\aa}} \\

    (\bseq{\stmt}{\ee})\subst{\aa}{\expr_\aa} & = &
    \bseq{\stmt\subst{\aa}{\expr_\aa}}{\ee\subst{\aa}{\expr_\aa}}\\

    (\fcall{e}{\overline{\typ}}{\overline{\expr}}{\overline{\aval}})\subst{\aa}{\expr_\aa} & = &
    \fcall{e\subst{\aa}{\expr_\aa}}{\overline{\typ}}{\overline{\expr\subst{\aa}{\expr_\aa}}}{\overline{\aval\subst{\aa}{\expr_\aa}}} \\

    % \multicolumn{3}{l}{\text{\textbf{Substitution of refinements in values}}}  \\

    (\vrec{\ff}{\overline{\bb}}{\overline{\xx}}{{e}})\subst{\aa}{\expr_\aa} & = & \left\{\begin{array}{ll}
        \vrec{\ff}{\overline{\bb}}{\overline{\xx}}{\ee\subst{\aa}{\expr_\aa}}, & \text{if } \aa \neq \bb_i \\
        \vrec{\ff}{\overline{\bb}}{\overline{\xx}}{\ee}, & \text{otherwise }
        \end{array}\right.
    \\

    \val\subst{\aa}{\expr_\aa} & = & \val \\

    % \multicolumn{3}{l}{\text{\textbf{Substitution of refinements in statements}}}  \\

    \sassign{\place}{\rval}\subst{\aa}{\expr_\aa} & = &
    \sassign{\place\subst{\aa}{\expr_\aa}}{\rval\subst{\aa}{\expr_\aa}} \\

    % \sskip\subst{\aa}{\expr_\aa} & = & \sskip \\

    % \multicolumn{3}{l}{\text{\textbf{Substitution of refinements in r-values}}}  \\

    % \val\subst{\aa}{\expr_\aa} & = & \val\subst{\aa}{\expr_\aa}\\

    (\rvstrgref{\place}) \subst{\aa}{\expr_\aa} & = & \rvstrgref{\place\subst{\aa}{\expr_\aa}} \\

    (\rvmutref{\place}) \subst{\aa}{\expr_\aa} & = & \rvmutref{\place\subst{\aa}{\expr_\aa}} \\

    (\rvshrref{\place}) \subst{\aa}{\expr_\aa} & = & \rvshrref{\place\subst{\aa}{\expr_\aa}} \\

    (\deref{\place}) \subst{\aa}{\expr_\aa} & = & \deref{\place\subst{\aa}{\expr_\aa}} \\
\end{array}
$$
\clearpage

\subsection{Type Sorts and Value Indices}

The following definitions connect values and types with
the refinement logic.
The function \getsort{\bty} associates a \emph{refinement sort} to
a base type \bty.
Values of type \bty must be indexed with refinements of that sort.
The function \interp{\cdot} maps values to a \emph{refinement index}.
This function is partial as only values of a base type can be refined.
Integers and booleans are mapped to the exact value in the logic.
Vectors are mapped to an index representing its length.

$$
\begin{array}{lcl}
    \getsort{\tint} & = & \sint\\
    \getsort{\tbool} & = & \sbool\\
    \getsort{\tvec} & = & \sint \\
    \interp{\ctrue}         & = & \ctrue \\
    \interp{\cfalse}        & = & \cfalse\\
    \interp{n}              & = & n, \text{ for } n \in \mathbb{Z} \\
    \interp{\vvec{n}{\val}} & = & n, \text{ for } n \in \mathbb{Z} \\
\end{array}
$$
\clearpage

\section{Declarative Judgements of \corelan.}
\label{subsec:formalism:typing}
\subsection{Well-typed Expressions}
\begin{judgment}{Well-typed Expressions}{\typing{\varcx}{\env}{\loccx}{\dynenv}{\rexpr}{\typ}{\loccx}{\dynenv}}

    \inferrule[\tlet]
    {
        \typing{\varcx}{\env}{\loccx_i}{\dynenv}{\ee_{\xx}}{\typ_{\xx}}{\loccx}{\dynenv}\\\\
        \typing{\varcx}{\env,\mapstoenv{\xx}{\typ_\xx}}{\loccx}{\dynenv}{\ee}{\typ}{\loccx_o}{\dynenv_o}
    }
    {\typing{\varcx}{\env}{\loccx_i}{\dynenv}{\blet{\xx}{\ee_{\xx}}{\ee}}{\typ}{\loccx_o}{\dynenv_o}}

    \inferrule[\tnew]
    {
     \wf{\typ} \\
     \wf{\loccx_o}\\\\
     \typing{\varcx, \lvar:\sloc}
            {\env, \mapstoenv{\xx}{\tptr{\lvar}}}
            {\loccx_i, \mapstoowned{\lvar}{\uninit{1}}}
            {\dynenv}{\ee}{\typ}{\loccx_o}{\dynenv} \\
    }
    {\typing{\varcx}
            {\env}{\loccx_i}{\dynenv}{\blet{\xx}{\new{\lvar}}{e}}{\typ}{\loccx_o}{\dynenv}
    }

    \inferrule[\tsub]
    {
        \typing{\varcx}{\env}{\loccx_i}{\dynenv}{\ee}
            {\typ_1}
            {\loccx}
            {\dynenv} \\\\
        \subtyping{\typ_1}{\typ} \\
        \loccxinc{\varcx}{\elftcx}{\llftcx}{\loccx}{\loccx_o}\\
    }
    {
        \typing{\varcx}{\env}{\loccx_i}{\dynenv}{\ee}
            {\typ}
            {\loccx_o}
            {\dynenv}
    }

    \inferrule[\tif]
    {
        \typing{\varcx}{\env}{\loccx_i}{\dynenv}{\ee}{\rtyp{\tbool}{\expr}}{\loccx_o}{\dynenv_o} \\\\
        \typing{\varcx, \expr}{\env}{\loccx_o}{\dynenv}{\ee_1}{\typ}{\loccx}{\dynenv} \\\\
        \typing{\varcx, \lnot \expr}{\env}{\loccx_o}{\dynenv}{\ee_2}{\typ}{\loccx}{\dynenv} \\
    }
    {\typing{\varcx}{\env}{\loccx_i}{\dynenv_i}{\bif{\ee}{\ee_1}{\ee_2}}{\typ}{\loccx}{\dynenv}}

    \inferrule[\tunpack]
    {
        \typing{\varcx, \aa : \getsort{\tcon}, \expr}{\env_1,\mapstoenv{\xx}{\rtyp{\tcon}{\aa}}, \env_2}
               {\loccx_i}{\dynenv}
               {\ee}{\typ}
               {\loccx_o}{\dynenv}
    }
    {
        \typing{\varcx}{\env_1,\mapstoenv{\xx}{\texists{\aa}{\rtyp{\tcon}{\aa}}{\expr}}, \env_2}
               {\loccx_i}{\dynenv}
               {\eunpack{\xx}{\aa}{e}}{\typ}
               {\loccx_o}{\dynenv}
    }

    \inferrule[\tcall]
    {
        \forall i. \typing{\varcx}{\env}{\loccx}{\dynenv}{\aval_i}{\applysubst{\substvar}{\typ_{i}}}{\loccx}{} \\
        \typing{\varcx}{\env}{\loccx}{\dynenv}{e}
               {\polysig{\overline{\tvar}}
                        {\overline{\aa: \sort}}
                        {\expr}
                        {\loccx_{i}}
                        {\overline{\typ}}
                        {\typ_o}
                        {\loccx_{o}}}
              {\loccx_1, \loccx_2 }{\dynenv} \\
        \substvar = \subst{\overline{\aa}}{\overline{\expr}} \\
        \loccxinc{\varcx}{}{}{\loccx_1}{\applysubst{\substvar}{\loccx_{i}}}\\
        \forall i.\sortck{\expr_i}{\sort_i} \\
        \lmodel{\varcx}{\applysubst{\substvar}{\expr}} \\
        \wf{\dynenv}\\
    }
    {
        \typing{\varcx}{\env}{\loccx}{\dynenv}
               {\fcall{\ee}{\overline{\typ}}{\overline{\expr}}{\overline{\aval}}}
               {\applysubst{\substvar}{\typ_o}}{\applysubst{\substvar}{\loccx_{o}}, \loccx_2}{}
    }
\end{judgment}

\begin{judgment}{Well-typed Expressions (assignment)}{\typing{\varcx}{\env}{\loccx}{\dynenv}{\rexpr}{\typ}{\loccx}{\dynenv}}
    \inferrule[\tassign]
    {
        \rvaltyping{\varcx}{\env}{\loccx_i}{\dynenv}{\ee}{\typ_v}{\loccx_o} \\\\
        \pltyping{\varcx}{\env}{\loccx_o}{\dynenv}{\place}{\tref{\mut}{\typ}}{\loccx_o} \\
        \subtyping{\typ_v}{\typ}
    }
    {\typing{\varcx}{\env}{\loccx_i}{\dynenv}{\sassign{\place}{\ee}}{\uninit{1}}{\loccx_o}{}}

    \inferrule[\tassignstrg]
    {
        \rvaltyping{\varcx}{\env}{\loccx_i}{\dynenv}{\ee}{\typ}{\loccx_o} \\\\
        \pltyping{\varcx}{\env}{\loccx_o}{\dynenv}{\place}{\tptr{\loc}}{\loccx_o}
    }
    {\typing{\varcx}{\env}{\loccx_i}{\dynenv}{\sassign{\place}{\ee}}{\uninit{1}}{\loccx_o[\loc \mapsto \typ]}{}}
\end{judgment}

\begin{judgment}{Well-typed Expressions (values)}{\typing{\varcx}{\env}{\loccx}{\dynenv}{\ee}{\typ}{\loccx}{}}

    \inferrule[\ttvar]
    {\mapstoenv{\xx}{\typ} \in \env}
    {\typing{\varcx}{\env}{\loccx}{\dynenv}{\xx}{\selfty{\typ}{\xx}}{\loccx}{}}

    \inferrule[\ttrue]
    {}
    {\typing{\varcx}{\env}{\loccx}{\dynenv}{\ctrue}{\rtyp{\tbool}{\ctrue}}{\loccx}{}}

    \inferrule[\tfalse]
    {}
    {\typing{\varcx}{\env}{\loccx}{\dynenv}{\cfalse}{\rtyp{\tbool}{\cfalse}}{\loccx}{}}

    \inferrule[\tconstint]
    {}
    {\typing{\varcx}{\env}{\loccx}{\dynenv}{i}{\rtyp{\tint}{i}}{\loccx}{}}

    \inferrule[\tfun]
    {   \typing{\varcx,\overline{\aa: \sort},\expr}
               {\env,
                \overline{\xx : \typ},
                \ff: \polysig{\overline{\tvar}}{{\overline{\aa: \sort}}}
                             {{\expr}}{\loccx_{i}}
                             {\overline{\typ}}
                             {{\typ}}
                             {\loccx_{o}}
                }
               {\loccx_i}{\dynenv}
               {\ee}
               {\typ}{\loccx_o}
               {}
    }
    {
        \typing{\varcx}{\env}{\loccx}{\dynenv}
               {\vrec{\ff}{\overline{\aa}}{\overline{\xx}}{{e}}}
               {\polysig{\overline{\tvar}}{{\overline{\aa: \sort}}}
                          {\expr}{\loccx_{i}}{\overline{\typ}}
                          {\typ}{\loccx_{o}}
               }
               {\loccx}{\dynenv}
    }

    \inferrule[\ttptr]
    {}
    {\typing{\varcx}{\env}{\loccx}{\dynenv}{\vptr{\cloc}{\ptrtag}}{\dynenv(\cloc, \ptrtag)}{\loccx}{\dynenv}}

    \inferrule[\tumem]
    {}
    {\typing{\varcx}{\env}{\loccx}{\dynenv}{\poison}{\uninit{1}}{\loccx}{\dynenv}}

    \inferrule[\tvecnew]
    {}
    {
        \typing{\varcx}{\env}{\loccx}{\dynenv}{\vecnew}{\loccx}
        {\kw{fn}() \rightarrow \tvec<0>}
        {}
    }

    \inferrule[\tvecpush]
    {}
    {
        \typing
        {\varcx}{\env}{\loccx}{\dynenv}{\vecpush}
        {\polysig{}
            {\lvar:\sloc}{\ctrue}
            {[\mapstoowned{\lvar}{\rtyp{\tvec}{n}}]}
            {\tptr{\lvar}}
            {\uninit{1}}{[\mapstoowned{\lvar}{\rtyp{\tvec}{n + 1}}]}
        }
        {\loccx}
        {}
    }

    \inferrule[\tvecindexmut]
    {}
    {
        \typing
        {\varcx}{\env}{\loccx}{\dynenv}{\vecindexmut}
        {
            \polysig
            {}
            {\aa:\sint,\bb:\sint}
            {0 \leq \bb < \aa}
            {\emptyset}
            {\tref{\mut}{\rtyp{\tvec}{\aa}}, \rtyp{\tint}{\bb}}
            {\tref{\mut}{\typ}}
            {\emptyset}
        }
        {\loccx}
        {}
    }

    \inferrule[\tvecvec]
    {
        n \geq 0 \\
        n > 0 \implies \val = \vptr{\cloc}{\ptrtag} \wedge \forall i \in [0, n).~\dynenv(\cloc + i, \ptrtag) = \tref{\mut}{\typ}
    }
    {
        \typing
        {\varcx}{\env}{\loccx}{\dynenv}{\vvec{n}{\val}}
        {
            \rtyp{\tvec}{n}
        }
        {\loccx}
        {}
    }

\end{judgment}

\begin{judgment}{Well-typed Expressions (borrows)}{\typing{\varcx}{\env}{\loccx}{\dynenv}{\ee}{\typ}{\loccx}{}}

\inferrule[\tstrgrebor]
{\pltyping{\varcx}{\env}{\loccx}{\dynenv}{\place}{\tptr{\loc}}{\loccx}}
{\rvaltyping{\varcx}{\env}{\loccx}{\dynenv}{\rvstrgref{\place}}{\tptr{\loc}}{\loccx}}

\inferrule[\tstrgmutrebor]
{
    \pltyping{\varcx}{\env}{\loccx}{\dynenv}{\place}{\tptr{\loc}}{\loccx} \\
    \subtyping{\loccx(\loc)}{\typ}
}
{\rvaltyping{\varcx}{\env}{\loccx}{\dynenv}{\rvmutref{\place}}{\tref{\mut}{\typ}}{\loccx[\loc\mapsto \typ]}}

\inferrule[\tmutmutrebor]
{\pltyping{\varcx}{\env}{\loccx}{\dynenv}{\place}{\tref{\mut}{\typ}}{\loccx}}
{\rvaltyping{\varcx}{\env}{\loccx}{\dynenv}{\rvmutref{\place}}{\tref{\mut}{\typ}}{\loccx}}

\inferrule[\tshrrebor]
{
    \pltyping{\varcx}{\env}{\loccx}{\dynenv}{\place}{\tref{\bormode}{\typ'}}{\loccx} \\
    \subtyping{\typ'}{\typ}
}
{\rvaltyping{\varcx}{\env}{\loccx}{\dynenv}{\rvshrref{\place}}{\tref{\shr}{\typ}}{\loccx}}

\end{judgment}

\begin{judgment}{Well-typed Expressions (dereference)}{\typing{\varcx}{\env}{\loccx}{\dynenv}{\ee}{\typ}{\loccx}{}}

\inferrule[\tderef]
{\pltyping{\varcx}{\env}{\loccx}{\dynenv}{\place}{\tref{\bormode}{\typ}}{\loccx}}
{\rvaltyping{\varcx}{\env}{\loccx}{\dynenv}{\deref{\place}}{\typ}{\loccx}}

\inferrule[\tderefstrg]
{\typing{\varcx}{\env}{\loccx}{\dynenv}{\place}{\tptr{\loc}}{\loccx}{}}
{\rvaltyping{\varcx}{\env}{\loccx}{\dynenv}{\deref{\place}}{\loccx(\loc)}{\loccx}}
\end{judgment}

\subsection{Location Context Inclusion and Subtyping}

\begin{judgment}{Context inclusion}{\loccxinc{\varcx}{\elftcx}{\llftcx}{\loccx}{\loccx}}
    \inferrule[\loccxinctrans]
        {\loccxinc
        {\varcx}
        {\elftcx}{\llftcx}
        {\loccx_1}
        {\loccx_2}\and
        \loccxinc
                {\varcx}
                {\elftcx}{\llftcx}
                {\loccx_2}
                {\loccx_3}}
        {
            \loccxinc
                {\varcx}
                {\elftcx}{\llftcx}
                {\loccx_1}
                {\loccx_3}
        }

    \inferrule[\loccxincperm]
        {\loccx' \text{ is a permutation of } \loccx}
        {
            \loccxinc
                {\varcx}
                {\elftcx}{\llftcx}
                {\loccx}
                {\loccx'}
        }

    \inferrule[\loccxincweaken]
        {}
        {
            \loccxinc
                {\varcx}
                {\elftcx}{\llftcx}
                {\loccx,\loccx'}
                {\loccx}
        }

    \inferrule[\loccxincframe]
        {
            \loccxinc
                {\varcx}
                {\elftcx}{\llftcx}
                {\loccx_1}{\loccx_2}
        }{
            \loccxinc
                {\varcx}
                {\elftcx}{\llftcx}
                {\loccx,\loccx_1}
                {\loccx, \loccx_2}
        }

    \inferrule[\loccxincsub]
        {
            \subtyping{\typ_1}{\typ_2}
        }
        {
            \loccxinc
                {\varcx}
                {\elftcx}{\llftcx}
                {\mapstoowned{\loc}{\typ_1}}
                {\mapstoowned{\loc}{\typ_2}}
        }
\end{judgment}

\begin{judgment}{Subtyping}{\subtyping[\varcx][\elftcx][\llftcx]{\typ}{\typ}}
    \inferrule[\subptr]
        {}
        {
            \subtyping{\tptr{\loc}}{\tptr{\loc}}
        }

\inferrule[\submem]
        {}
        {
            \subtyping{\uninit{n}}{\uninit{n}}
        }

\inferrule[\subfun]
        {
            \entailment{\varcx, \overline{\aa: \sort}}{\expr_2 \Rightarrow \expr_1} \and
            \loccxinc
                {\varcx, \overline{\aa: \sort}}
                {\elftcx}{\llftcx}
                {\loccx_{2i}}
                {\loccx_{1i}} \and
            \forall i. \subtyping[\varcx, \overline{\aa: \sort}]{\typ_{2i}}{\typ_{1i}} \\
        \loccxinc
            {\varcx, \overline{\aa: \sort}}
            {\elftcx}{\llftcx}
            {\loccx_{1o}}
            {\loccx_{2o}} \and
        \subtyping[\varcx, \overline{\aa: \sort}]{\typ_{1o}}{\typ_{2o}}
        }
        {
            \subtyping{
            \polysig{\overline{\tvar}}
            {\overline{\aa: \sort}}
            {\expr_1}
            {\loccx_{1i}}
            {\overline{\typ_1}}
            {\typ_{1o}}
            {\loccx_{1o}}
            }{
            \polysig{\overline{\tvar}}
            {\overline{\aa: \sort}}
            {\expr_2}
            {\loccx_{2i}}
            {\overline{\typ_2}}
            {\typ_{2o}}
            {\loccx_{2o}}
            }
        }

    \inferrule[\subrtyp]
        {
            \entailment{\varcx}{\expr_1 = \expr_2}
        }{
            \subtyping
                {\rtyp{\tcon}{\expr_1}}
                {\rtyp{\tcon}{\expr_2}}
        }

    \inferrule[\subunpack]
        {
          % \fresh{\aa}{\varcx} \and
           \subtyping
                [\varcx, \aa: \getsort{\tcon}, \expr]
                {\rtyp{\tcon}{\aa}}
                {\typ}
        }{
            \subtyping
                {\texists{\aa}{\rtyp{\tcon}{\aa}}{\expr}}
                {\typ}
        }

    \inferrule[\subexists]
        {
            \entailment{\varcx}{\expr_2[\expr_1/\aa]}
        }{
            \subtyping
                {\rtyp{\tcon}{\expr_1}}
                {\texists{\aa}{\rtyp{\tcon}{\aa}}{\expr_2}}
        }

    \inferrule[\subborshr]
        {
            \subtyping{\typ_1}{\typ_2}
        }{
            \subtyping
                {\tbor{\lft}{\shr}{\typ_1}}
                {\tbor{\lft}{\shr}{\typ_2}}
        }

    \inferrule[\subbormut]
        {
            \subtyping{\typ_1}{\typ_2}
            \and
            \subtyping{\typ_2}{\typ_1}
        }{
            \subtyping
                {\tbor{\lft}{\mut}{\typ_1}}
                {\tbor{\lft}{\mut}{\typ_2}}
        }
\end{judgment}

\subsection{Well-formedness}
The well-formedness judgments (\wfvdash) document the binding struct
of the grammar as well as well-sortedness of refinements.
In what follows, we assume well-formed implicitly in other judgments.

\begin{judgment}{Well-formed Types}{\wf[\varcx]{\typ}}
    \inferrule[\twfidx]
    {\sortck[\varcx]{\expr}{\getsort{\tcon}}}
    {\wf[\varcx]{\rtyp{\tcon}{\expr}}}

    \inferrule[\twfex]
    {\sortck[\varcx,\aa :\getsort{\tcon} ]{\expr}{\tbool{}}}
    {\wf[\varcx]{\texists{\aa}{\rtyp{\tcon}{\aa}}{\expr}}
    }

    \inferrule[\twfptr]
    {
        \sortck{\loc}{\sloc}
    }
    {
        \wf[\varcx]{\tptr{\loc}}
    }

    \inferrule[\twfref]
    {\wf[\varcx]{\typ}}
    {\wf[\varcx]{\tbor{\lft}{\bormode}{\typ}}
    }

    \inferrule[\twfmem]
    {}
    {\wf[\varcx]{\uninit{n}}
    }

    \inferrule[\twffun]
    {
        \sortck[\varcx,\overline{\aa: \sort}]{\expr}{\sbool}\\
        \dom{\loccx_o} \subseteq \dom{\loccx_i} \\
        % \varcx' = \varcx\setminus\{(\lvar:\sloc) \mid  (\lvar:\sloc) \in \varcx\}\\
        \wf[\varcx',\overline{\aa: \sort}]{\loccx_i}\\
        \forall i. \wf[\varcx',\overline{\aa: \sort}]{\typ_i}\\
        \wf[\varcx',\overline{\aa: \sort}]{\typ_o}\\
        \wf[\varcx',\overline{\aa: \sort}]{\loccx_o}
    }
    {\wf[\varcx]{\polysig{\overline{\tvar}}
    {{\overline{\aa: \sort}}}
    {{\expr}}
    {\loccx_i}
    {\overline{\typ}}
    {\typ_o}
    {\loccx_o}}
    }
\end{judgment}

\begin{judgment}{Well-formed Value Contexts}{\wf[\varcx]{\env}}

    \inferrule[\twfbind]
        {\wf[\varcx]{\typ}\\
        \wf[\varcx]{\env}
        }
        {\wf[\varcx]{\env, \mapstoenv{\xx}{\typ}}}

    \inferrule[\twfemp]{}{\wf[\varcx]{\emptyset}}
\end{judgment}

\begin{judgment}{Well-formed Dynamic Contexts}{\wf[\varcx]{\dynenv}}
    \inferrule[\twfbind]
        {\wf[\varcx]{\typ}\\
        \wf[\varcx]{\dynenv}
        }
        {\wf[\varcx]{\dynenv, \mapstoowned{(\cloc,\ptrtag)}{\typ}}}

    \inferrule[\twfemp]{}{\wf[\varcx]{\emptyset}}
\end{judgment}
\begin{judgment}{Well-formed Location contexts}{\wf[\varcx]{\loccx}}
    \inferrule[\twfbind]
        {
        \wf[\varcx]{\typ} \\
        \wf[\varcx]{\loccx} \\
        \sortck{\loc}{\sloc} \\
        \loc \notin \dom{\loccx}
        }
        {\wf[\varcx]{\loccx, \mapstoowned{\loc}{\typ}}}

    \inferrule[\twfemp]{}{\wf[\varcx]{\emptyset}}
\end{judgment}

\begin{judgment}{Well-formed Refinements Contexts}{\wfvarcx{\varcx}}
    \inferrule
        {}
        { \wfvarcx{\emptyset}}

    \inferrule
        { \wfvarcx{\varcx} \\ \sortck{\expr}{\sbool}}
        { \wfvarcx{\varcx,\expr} }

    \inferrule
        { \wfvarcx{\varcx} \\ \aa \notin \dom{\varcx}}
        { \wfvarcx{\varcx,\aa:\sort} }
\end{judgment}

\begin{judgment}{Well-sorted Refinements}{\sortck[\varcx]{\expr}{\sort}}
    \inferrule{\aa:\sort \in \varcx}{\sortck{\aa}{\sort}}

    \inferrule{\sortck{\expr_1}{\sort}\\\sortck{\expr_2}{\sort}}{\sortck{\expr_1=\expr_2}{\sbool}}

    \inferrule{}{\sortck{\cloc}{\sloc}}

    \inferrule
        {
            \oplus \in \{+, -, *\} \\\\
            \sortck{\expr}{\sint} \\ \sortck{\expr_2}{\sint}
        }
        {\sortck{\expr_1 \oplus \expr_2}{\sint}}

    \inferrule
        {
            \oplus \in \{\wedge, \vee\} \\\\
            \sortck{\expr}{\sbool} \\ \sortck{\expr_2}{\sbool}
        }
        {\sortck{\expr_1 \oplus \expr_2}{\sbool}}

    \inferrule
        {
            \sortck{\expr}{\sbool}
        }
        {\sortck{\neg\expr}{\sbool}}

    \inferrule
        {
            n \in \mathbb{Z}
        }
        {\sortck{n}{\sint}}
\end{judgment}

\subsection{Implication Checking}

Implication checking \lmodel{\varcx}{\expr} is implemented via SMT.
Here we axiomatize the properties we need for the proof.

\begin{assumption}[Weakening]\label{assumption:model:weakening}
    If \lmodel{\varcx_1,\varcx_2}{\expr} then \lmodel{\varcx_1, \varcx', \varcx_2}{\expr}.
\end{assumption}

% \begin{assumption}[Strengthening]\label{assumption:model:strengthening}
%     If \lmodel{\varcx_1}{\expr} and $\dom{\varcx_1} \cap \dom{\varcx_2} = \emptyset$,
%     then \lmodel{\varcx_1, \varcx_2}{\expr}.
% \end{assumption}

\begin{assumption}[Cut]\label{assumption:model:cut}
    If \lmodel{\varcx_1}{\expr_1} and
       \lmodel{\varcx_1, \expr_1, \varcx_2}{\expr_2},
    then \lmodel{\varcx_1, \varcx_2}{\expr_2}.
\end{assumption}

\begin{assumption}[Identity]\label{assumption:model:identity}
    Forall \varcx and \expr, \lmodel{\varcx, \expr}{\expr}.
\end{assumption}

\begin{assumption}[Substitution]\label{assumption:model:substitution}
    If \sortck[\varcx_1]{\expr_\aa}{\sort} and \entailment{\varcx_1, \aa:\sort, \varcx_2}{\expr},
    then \entailment{\varcx_1, \varcx_2[\expr_\aa/\aa]}{\expr[\expr_\aa/\aa]}.
\end{assumption}

\begin{assumption}[Transitive]\label{assumption:model:transitive}
    If \entailment{\varcx}{\expr_1 = \expr_2} and \entailment{\varcx}{\expr_2 = \expr_3},
    then \entailment{\varcx}{\expr_1 = \expr_3}.
\end{assumption}

\begin{assumption}[Transitivity of Implication]\label{assumption:model:transitive:implication}
    If \entailment{\varcx}{\expr_1 \Rightarrow \expr_2} and \entailment{\varcx}{\expr_2 \Rightarrow \expr_3},
    then \entailment{\varcx}{\expr_1 \Rightarrow \expr_3}.
\end{assumption}

\begin{assumption}[Congruence]\label{assumption:model:congruence}\label{assumption:model:equality}
    If \entailment{\varcx}{\expr_1 = \expr_2} and \entailment{\varcx}{\expr[\expr_2/\aa]},
    then \entailment{\varcx}{\expr[\expr_1/\aa]}.
\end{assumption}

\begin{assumption}[Reflexivity]\label{assumption:model:reflexive}
    \lmodel{\varcx}{\expr = \expr}.
\end{assumption}

\section{Operational Semantics of \corelan.}
\label{subsec:formalism:operational}
The operational semantics follows a sandard call-by-value evaluation.
Note that function arguments are A-values and thus they must not be
further evaluated.
We use the convention that a rule with a stacked borrow transition
as a premise does not get stuck if the transition does not hold but
instead evaluates to an error.
In \opvecindexmut{}, for example, evaluation will return an error
if either the \text{EAccess} or \text{ERetag} transition does not hold,
but it will get stuck if the index does not point to a valid location.

$$
\begin{array}{rrcll}
    \syntaxcat{Heap} &
        \hp  & ::= & \emptyset \mid \hp\hbind{\cloc}{\hval}  \\
    \syntaxcat{Contexts} &
        \CC  & ::= & \bullet \mid \blet{\xx}{\CC}{e}
              \mid \bif{\CC}{\ee}{\ee}
              \mid \fcall{\CC}{\overline{\typ}}{\overline{\expr}}{\overline{\aval}}
              \mid \sassign{\place}{\CC} \\
\end{array}
$$

\begin{judgment}{Operational Semantics}{\eval{\hp}{\sbstate}{\rexpr}{\hp}{\sbstate}{\rexpr} or \evalerr{\hp}{\sbstate}{\ee}}
  \inferrule[\opprop]
    { \eval{\hp_i}{\sbstate_i}{\ee}{\hp_o}{\sbstate_o}{\ee'}}
    {\eval{\hp_i}{\sbstate_i}{\CC[\ee]}
          {\hp_o}{\sbstate_o}{\CC[\ee']}}

  \inferrule[\opproperr]
    {\evalerr{\hp_i}{\sbstate_i}{\ee}}
    {\evalerr{\hp_i}{\sbstate_i}{\CC[\ee]}}

  \inferrule[\opnew]
    {\fresh{\cloc}{\hp} \\ \transnew{\sbstate}{\sbstate'} }
    {\eval{\hp}{\sbstate}{\blet{\xx}{\new{\lvar}}{\rexpr}}
          {\hp\hbind{\cloc}{\poison}}{\sbstate'}{\rexpr[\cloc/\lvar][\vptr{\cloc}{\ptrtag}/\xx]}}

  \inferrule[\oplet]
    {}
    {\eval{\hp}{\sbstate}{\blet{\xx}{\val}{\rexpr}}
          {\hp}{\sbstate}{\rexpr[\val/\xx]}}

  \inferrule[\opifTrue]
    {}
    {\eval{\hp}{\sbstate}{\bif{\ctrue}{\rexpr_1}{\rexpr_2}}
          {\hp}{\sbstate}{\rexpr_1}}

  \inferrule[\opifFalse]
    {}
    {\eval{\hp}{\sbstate}{\bif{\cfalse}{\rexpr_1}{\rexpr_2}}
          {\hp}{\sbstate}{\rexpr_2}}

  \inferrule[\opcall]
    {}
    {\eval{\hp}{\sbstate}{\fcall{(\vrec{\ff}{\overline{\aa}}{\overline{\xx}}{\rexpr})}{\overline{\typ}}{\overline{\expr}}{\overline{\val}}}
          {\hp}{\sbstate}{\rexpr[\vrec{\ff}{\overline{\aa}}{\overline{\xx}}{\rexpr}/\ff,\overline{\val}/\overline{\xx}, \overline{\expr}/\overline{\aa}]}}

  \inferrule[\opunpack]
    {}
    {\eval{\hp}{\sbstate}{\bunpack{\xx}{\aa}{\rexpr}}
          {\hp}{\sbstate}{\rexpr}}

    \inferrule[\opass]
    { \transwrite{\sbstate}{\cloc}{\ptrtag}{\sbstate'} }
    {\eval{\hp\hbind{\cloc}{\val}}{\sbstate}{\sassign{\vptr{\cloc}{\ptrtag}}{\val'}}
          {\hp\hbind{\cloc}{\val'}}{\sbstate'}{\poison}}

  \inferrule[\opstrgrebor]
    {\transreborrow{\sbstate}{\cloc}{\ptrtag}{\ptrtag'}{\SbRef{\mut}}{\sbstate'}}
    {
      \eval{\hp}{\sbstate}{\rvstrgref{\vptr{\cloc}{\ptrtag}}}
           {\hp}{\sbstate'}{\vptr{\cloc}{\ptrtag'}}
    }

  \inferrule[\opmutrebor]
    {\transreborrow{\sbstate}{\cloc}{\ptrtag}{\ptrtag'}{\SbRef{\mut}}{\sbstate'}}
    {
      \eval{\hp}{\sbstate}{\rvmutref{\vptr{\cloc}{\ptrtag}}}
           {\hp}{\sbstate'}{\vptr{\cloc}{\ptrtag'}}
    }

  \inferrule[\opshrrebor]
    {\transreborrow{\sbstate}{\cloc}{\ptrtag}{\ptrtag'}{\SbRef{\shr}}{\sbstate'}}
    {
      \eval{\hp}{\sbstate}{\rvshrref{\vptr{\cloc}{\ptrtag}}}
           {\hp}{\sbstate'}{\vptr{\cloc}{\ptrtag'}}
    }

  \inferrule[\opderef]
    {
      \transread{\sbstate}{\cloc}{\ptrtag}{\sbstate'}
    }
    {
      \eval{\hp}{\sbstate}{\deref{\vptr{\cloc}{\ptrtag}}}
           {\hp}{\sbstate'}{\hp(\cloc)}
    }
\end{judgment}

\begin{judgment}{Operational Semantics (vectors)}{\eval{\hp}{\sbstate}{\ee}{\hp}{\sbstate}{\rexpr}}
    \inferrule[\opvecnew]
    {}
    {
        \eval
          {\hp}{\sbstate}
          {\fcall{\vecnew}{}{}{}}
          {\hp}{\sbstate}
          {\vvec{0}{\poison}}
    }

    \inferrule[\opvecpush]
    {
        \transwrite{\sbstate_i}{\cloc}{\ptrtag}{\sbstate} \\\\
        \transdealloc{\sbstate}{\cloc'}{\ptrtag'}{n}{\sbstate'} \\\\
        \transalloc{\sbstate'}{\cloc''}{\ptrtag''}{n+1}{\sbstate_o} \\\\
        [\cloc'', \cloc'' + n] \mathrel{\#} \dom{\hp} \\\\
        \hp_i = \hp\hbind{\cloc}{\vvec{n}{\vptr{\cloc'}{\ptrtag'}}}\hbindn{n}{\cloc'}{\overline{\val}} \\\\
        \hp_o = \hp\hbind{\cloc}{\vvec{n+1}{\vptr{\cloc''}{\ptrtag''}}}\hbindn{n+1}{\cloc''}{\overline{\val} \append [\val]}
    }
    {
        \eval
          {\hp_i}{\sbstate_i}
          {\fcall{\vecpush}{}{\cloc}{\vptr{\cloc}{\ptrtag}, \val}}
          {\hp_o}{\sbstate_o}
          {\poison}
    }

    \inferrule[\opvecpushempty]
    {
        \transwrite{\sbstate_i}{\cloc}{\ptrtag}{\sbstate} \\\\
        \transalloc{\sbstate}{\cloc'}{\ptrtag'}{1}{\sbstate_o} \\\\
        \cloc' \notin \dom{\hp} \\\\
        \hp_i = \hp\hbind{\cloc}{\vvec{0}{\val'}} \\\\
        \hp_o = \hp\hbind{\cloc}{\vvec{1}{\vptr{\cloc'}{\ptrtag'}}}\hbind{\cloc'}{\val}
    }
    {
        \eval
          {\hp_i}{\sbstate_i}
          {\fcall{\vecpush}{}{\cloc}{\vptr{\cloc}{\ptrtag}, \val}}
          {\hp_o}{\sbstate_o}
          {\poison}
    }

    \inferrule[\opvecindexmut]
    {
        \cloc + i \in \dom{\hp} \\\\
        \transread{\sbstate_i}{\cloc}{\ptrtag}{\sbstate} \\\\
        \transreborrow{\sbstate}{\cloc' + i}{\ptrtag'}{\ptrtag''}{\mut}{\sbstate_o} \\\\
        \hp = \hp'\hbind{\cloc}{\vvec{n}{\vptr{\cloc'}{\ptrtag'}}}
    }
    {
        \eval
          {\hp}{\sbstate_i}
          {\fcall{\vecindexmut}{}{}{\vptr{\cloc}{\ptrtag}, i}}
          {\hp}{\sbstate_o}
          {\vptr{\cloc' + i}{\ptrtag''}}
    }
\end{judgment}

\subsection{Well-typed States}
Intuitively, a state is well-typed if the following conditions
hold:
(1) for each location \cloc the stack $\sbstate\dotstacks(\cloc)$
must be split into a section composed of only unique permissions
followed by a section composed of only shared permissions,
(2) pointers \vptr{\cloc}{\ptrtag} in the shared section
must be associated to shared references in \dynenv
(\ie $\dynenv(\cloc,\ptrtag) = \tref{\shr}{\typ}$),
(3) the unique section must further be split
into a section associated to strong pointers
($\dynenv(\cloc,\ptrtag) = \tptr{\cloc}$) and a section
associated with mutable references
($\dynenv(\cloc, \ptrtag) = \tref{\mut}{\typ}$),
and (4) for every pointer \vptr{\cloc}{\ptrtag} it must
be safe to read from it at type $\dynenv(\cloc, \ptrtag)$.
This implies, for example, that for every mutable reference
\tref{\mut}{\typ} associated to a location \cloc the type \typ
must be a subtype of $\loccx(\cloc)$.

\begin{judgment}{Well-typed state}{
  \statetyping[\varcx][\loccx][\dynenv]{\hp}{\sbstate}\quad
}
  \inferrule
  {
    \dom{\hp} = \dom{\sbstate\dotstacks} \\\\
    \forall \cloc\in \dom{\hp}.~\heaplettyping{\cloc}{\hp(\cloc)}{\sbstate\dotstacks(\cloc)}
  }
  {
    \statetyping{\hp}{\sbstate}
  }
\end{judgment}

\begin{judgment}{Well-typed heaplet}{\heaplettyping[\varcx][\loccx][\dynenv]{\cloc}{\val}{\stack}}

  \inferrule[\hptracked]
    {
    \cloc \in \dom{\loccx} \\
    \stacktyping{\shr}{\cloc}{\stack}{\loccx(\cloc)} \\\\
    \typing{\varcx}{\emptyset}{\loccx}{\dynenv}{\val}{\loccx(\cloc)}{\loccx}{}
    }
    {
      \heaplettyping{\cloc}{\val}{\stack}
    }

  \inferrule[\hpuntracked]
    {
    \cloc \notin \dom{\loccx} \\
    \stacktyping{\shr}{\cloc}{\stack}{\typ} \\\\
    \typing{\varcx}{\emptyset}{\loccx}{\dynenv}{\val}{\typ}{\loccx}{}
    }
    {
      \heaplettyping{\cloc}{\val}{\stack}
    }
\end{judgment}

\begin{judgment}{Well-typed stacks}{
    \stacktyping[\varcx][\dynenv]{\shr}{\cloc}{S,(\sharedro, \ptrtag, \_)}{\typ}
}

  \inferrule[\hpshr]
  {
    \dynenv(\cloc, \ptrtag) = \tref{\shr}{\typ'} \\
    \stacktyping{\shr}{\cloc}{S}{\typ} \\\\
    \subtyping{\typ}{\typ'}
  }
  {
    \stacktyping{\shr}{\cloc}{S,(\sharedro, \ptrtag, \_)}{\typ}
  }

  \inferrule[\hpshrmut]
  {
    \stacktyping{\mut}{\cloc}{S}{\typ}
  }
  {
    \stacktyping{\shr}{\cloc}{S}{\typ}
  }

  \inferrule[\hpmut]
  {
    \dynenv(\cloc, \ptrtag) = \tref{\mut}{\typ'} \\
    \stacktyping{\mut}{\cloc}{S}{\typ} \\\\
    \subtyping{\typ}{\typ'} \\
    \subtyping{\typ'}{\typ}
  }
  {
    \stacktyping{\mut}{\cloc}{S,(\unique, \ptrtag, \_)}{\typ}
  }

  \inferrule[\hpmutstrg]
  {
    \stacktyping{\strg}{\cloc}{S}{\typ}
  }
  {
    \stacktyping{\mut}{\cloc}{S}{\typ}
  }

  \inferrule[\hpstrg]
  {
    \dynenv(\cloc, \ptrtag) = \tptr{\cloc} \\
    % \valtyping{\varcx}{\emptyset}{\loccx}{\dynenv}{\val}{\loccx(\cloc)} \\\\
    \stacktyping{\strg}{\cloc}{S}{\typ}
  }
  {
    \stacktyping{\strg}{\cloc}{S,(\unique, \ptrtag, \_)}{\typ}
  }

  \inferrule[\hpempty]
  {}
  {
    \stacktyping{\strg}{\cloc}{\emptyset}{\typ}
  }

  \inferrule[\hpdisabled]
  {
    \stacktyping{\ast}{\cloc}{S}{\typ}
  }
  {
    \stacktyping{\ast}{\cloc}{S,(\disabled, \_, \_)}{\typ}
  }
\end{judgment}

\section{Soundness of \corelan.}
\label{subsec:formalism:soundness}

\clearpage
\subsection{Main theorems}

Our soundness claim states that
evaluation of a well typed expression will
1) return a value of the same type,
2) return a memory violation error (\memerr), or
3) diverge.

\begin{restatable}[Soundness]{theorem}{soundness}
\label{them:soundness}
If
\begin{itemize}
\item $
\typing{\varcx}{\emptyset}{\loccx_i}{\dynenv_i}{\rexpr_i}{\typ}{\loccx}{\_}
$,
\item \statetyping[\varcx][\loccx_i][\dynenv_i]{\hp_i}{\sbstate_i}, and
\item \goesto
      {\hp_i}{\sbstate_i}{\rexpr_i}
      {\hp}{\sbstate}{\rexpr}.
\end{itemize}
then
\begin{itemize}
    \item $\rexpr$ is a value and there exist $\loccx_o $ and $\dynenv_o \supseteq \dynenv_i$ so that
    \typing{\varcx}{\emptyset}{\loccx_o}{\dynenv_o}{\rexpr}{\typ}{\loccx}{\_}, or
    \item
     $\evalerr{\hp_o}{\sbstate_o}{\rexpr}$, or
     \item there exists $\loccx_o$, $\dynenv_o \supseteq \dynenv_i$, $\hp_o, \sbstate_o$, and $\rexpr_o$ such that
     $\eval{\hp}{\sbstate}{\rexpr}{\hp_o}{\sbstate_o}{\rexpr_o}$,
     \statetyping[\varcx][\loccx_o][\dynenv_o]{\hp_o}{\sbstate_o}, and
    \typing{\varcx}{\emptyset}{\loccx_o}{\dynenv_o}{\rexpr_o}{\typ}{\loccx}{\_}.
\end{itemize}
\end{restatable}

\begin{restatable}[Progress]{theorem}{progress}
\label{theorem:progress}
If
\typing{\emptyset}{\emptyset}{\loccx_i}{\dynenv_i}{\rexpr}{\typ}{\loccx_o}{\dynenv_o}
and
\statetyping[\emptyset][\loccx_i][\dynenv_i]{\hp_i}{\sbstate_i},
then
\begin{itemize}
\item \rexpr is a value,
\item \evalerr{\hp_i}{\sbstate_i}{\rexpr}, or
\item there exists
     $\hp_o$, $\sbstate_o$,
     and $\rexpr_o$ so that
    \eval{\hp_i}{\sbstate_i}{\rexpr}{\hp_o}{\sbstate_o}{\rexpr_o}.
\end{itemize}
\end{restatable}

\begin{restatable}[Preservation]{theorem}{preservation}
\label{theorem:preservation}
If
\begin{itemize}
\item $
\typing{\varcx}{\emptyset}{\loccx_i}{\dynenv_i}{\rexpr}{\typ}{\loccx}{\dynenv}
$,
\item \eval{\hp_i}{\sbstate_i}{\rexpr}{\hp_o}{\sbstate_o}{\rexpr_o}, and
\item \statetyping[\varcx][\loccx_i][\dynenv_i]{\hp_i}{\sbstate_i},
\end{itemize}
then there exist $\loccx_o$ and $\dynenv_o \supseteq \dynenv_i$, such that
\begin{itemize}
    \item $
    \typing{\varcx}{\emptyset}{\loccx_o}{\dynenv_o}{\rexpr_o}{\typ}{\loccx}{\dynenv}
    $ and
    \item \statetyping[\varcx][\loccx_o][\dynenv_o]{\hp_o}{\sbstate_o}
\end{itemize}
\end{restatable}

\clearpage
\subsection{Proof of soudness}
\soundness*
\begin{proof}
By induction on the length of the evaluation path.
For path of length 0, the theorem is a direct implication of Progress (Theorem~\ref{theorem:progress}).
For path of length $n+1$:
$\goesto
      {\hp_i}{\sbstate_i}{\rexpr_i}
      {\hp_n}{\sbstate_n}{\rexpr_n} \rightsquigarrow
      \langle \hp,\sbstate, \rexpr \rangle
$.
By the induction hypothesis and determinism of our operational semantics,
there exists $\loccx_o$ and $\dynenv_o \supseteq \dynenv_i$ such that
     $\statetyping[\varcx][\loccx_o][\dynenv_o]{\hp_o}{\sbstate_o}$ and
    \typing{\varcx}{\emptyset}{\loccx_o}{\dynenv_o}{\rexpr}{\typ}{\loccx}{\_}.
    The proof concludes by
    applying progress (Theorem~\ref{theorem:progress}) and then
    preservation (Theorem~\ref{theorem:preservation}).
\end{proof}

\clearpage
\subsection{Proof of preservation}
\preservation*
\begin{proof}
By induction on the type derivation tree.
\begin{itemize}
  \item \textbf{Rule \tsub:}
    By inversion of the rule:
    (1) \typing{\varcx}{\env}{\loccx_i}{\dynenv_i}{\ee}
    {\typ_1}
    {\loccx'}
    {\dynenv},
    (2) \subtyping{\typ_1}{\typ}, and
    (3) \loccxinc{\varcx}{}{}{\loccx'}{\loccx}.
    By inductive hypothesis on (1):
    then there exist $\loccx_o$ and $\dynenv_o \supseteq \dynenv_i$, such that
    (4) \typing{\varcx}{\emptyset}{\loccx_o}{\dynenv_o}{\rexpr_o}{\typ_1}{\loccx}{\dynenv}
    and
    (5) \statetyping[\varcx][\loccx_o][\dynenv_o]{\hp}{\sbstate}.
    The proof concludes by (4), (2), (3), and rule \tsub.

    \item \textbf{Rule \tif:}
    Let $\ee \equiv \bif{\ee_0}{\ee_1}{\ee_2}$.
    By inversion of the rule:

    \begin{enumerate}
      \item \typing{\varcx}{\emptyset}{\loccx_i}{\dynenv_i}{\ee_0}{\rtyp{\tbool}{\expr}}{\loccx_0}{\dynenv_o}
      \item \typing{\varcx, \expr}{\emptyset}{\loccx_0}{\dynenv_i}{\ee_1}{\typ}{\loccx}{\dynenv}
      \item \typing{\varcx, \lnot \expr}{\emptyset}{\loccx_0}{\dynenv_i}{\ee_2}{\typ_2}{\loccx}{\dynenv}.
    \end{enumerate}
    Since \ee steps, there are three cases:
    \begin{itemize}
    \item \textbf{Rule \opprop:}
    $\eval{\hp_i}{\sbstate_i}{\bif{\ee_0}{\ee_1}{\ee_2}}
    {\hp_o}{\sbstate_o}{\bif{\ee'_0}{\ee_1}{\ee_2}}$.
    By inversion:
    $\eval{\hp_i}{\sbstate_i}{\ee_0}
    {\hp_o}{\sbstate_o}{\ee'_0}$.
    By (1) and inductive hypothesis:
    there exists $\loccx_o$ and $\dynenv_o \supseteq \dynenv_i$, so that
    $\typing{\varcx}{\emptyset}{\loccx_o}{\dynenv_o}{\rexpr'_0}{\rtyp{\tbool}{\expr}}{\loccx_0}{\dynenv}$
    and
    \statetyping[\varcx][\loccx_o][\dynenv_o]{\hp_o}{\sbstate_o}
    By (2) and (3), weakened to $\dynenv_o$ using Lemma~\ref{lemma:weakening}, and rule \tif:
    $\typing{\varcx}{\emptyset}{\loccx_o}{\dynenv_o}{\bif{\ee'_0}{\ee_1}{\ee_2}}{\typ}{\loccx}{\dynenv}$,
    which concludes the proof.
    \item \textbf{Rule \opifTrue: }
    $\eval{\hp}{\sbstate}{\bif{\ctrue}{\rexpr_1}{\rexpr_2}}
    {\hp}{\sbstate}{\rexpr_1}$,
    where $\hp = \hp_i = \hp_o$ and $\sbstate = \sbstate_i = \sbstate_o$.
    Trivial by (2) and with $\loccx_o = \loccx_i$ and $\dynenv_o = \dynenv_i$.
    \item \textbf{Rule \opifFalse: }
    $\eval{\hp}{\sbstate}{\bif{\cfalse}{\rexpr_1}{\rexpr_2}}
    {\hp}{\sbstate}{\rexpr_2}$,
    where $\hp = \hp_i = \hp_o$ and $\sbstate = \sbstate_i = \sbstate_o$.
    Trivial by (3) and with $\loccx_o = \loccx_i$ and $\dynenv_o = \dynenv_i$.
    \end{itemize}
    \item \textbf{Rule \tnew:}
    Let $\ee \equiv \blet{\xx}{\new{\lvar}}{\ee'}$. By inversion of the rule we get:
    $$
    (1)~\typing{\varcx,\lvar: \sloc}
           {\mapstoenv{\xx}{\tptr{\lvar}}}
           {\loccx_i,\mapstoowned{\lvar}{\uninit{1}}}
           {\dynenv_i}
           {\ee'}
           {\typ}{\loccx}
           {}
    $$
    By assumption we have
    $\eval{\hp_i}{\sbstate_i}
          {\blet{\xx}{\new{\lvar}}{\ee'}}
          {\hp_o}{\sbstate_o}{\ee_o}$, thus the rule \opnew{} must have been applied and we know
    $\ee_o \equiv \ee'[\cloc/\lvar][\vptr{\cloc}{\ptrtag}/\xx]$ and
    $\hp_o \equiv \hp_i\hbind{\cloc}{\poison}$.
    By Lemma~\ref{lemma:type-substitution} we get
    $$
    (2)~\typing{\varcx}
           {\mapstoenv{\xx}{\tptr{\cloc}}}
           {\loccx_i[\cloc/\lvar],\mapstoowned{\cloc}{\uninit{1}}}
           {\dynenv_i[\cloc/\lvar]}
           {\ee'[\cloc/\lvar]}
           {\typ[\cloc/\lvar]}{\loccx[\cloc/\lvar]}
           {}
    $$
    We know \wf{\typ} and \wf{\loccx} by inversion of \tnew,
    thereby, we know $\typ=\typ[\cloc/\lvar]$ and $\loccx = \loccx[\cloc/\lvar]$
    by lemmas~\ref{lemma:fv-subst} and \ref{lemma:wf-fv}.
    Then, applying Lemma~\ref{lemma:program-substitution} to (2) we get:
    $$
    (3)~\typing{\varcx}
           {\mapstoenv{\xx}{\tptr{\cloc}}}
           {\loccx_i[\cloc/\lvar],\mapstoowned{\cloc}{\uninit{1}}}
           {\dynenv_i[\cloc/\lvar],\mapstoowned{(\cloc, \ptrtag)}{\tptr{\cloc}}}
           {\ee'[\cloc/\lvar][\vptr{\cloc}{\ptrtag}/\xx]}
           {\typ}{\loccx}
           {}
    $$
    Picking $T_o=T_i[\cloc/\lvar]$ and $\dynenv_o=\dynenv_i,\mapstoowned{(\cloc, \ptrtag)}{\tptr{\cloc}}$ we
    get the first part of the conclusion.
    It remains to show $\statetyping[\varcx][\loccx_o][\dynenv_o]{\hp_o}{\sbstate_o}$ which is a direct application
    of Lemma~\ref{lemma:event:alloc}.

    % \item \textbf{Rule \tseq:}
    % Let $\ee \equiv \bseq{\stmt}{\rexpr'}$.
    % By inversion of the rule we get:
    % (1) \stmtyping{\varcx}{\env}{\loccx_i}{\dynenv_i}{\stmt}{\loccx_{\stmt}}{\dynenv}
    % and
    % (2) \typing{\varcx}{\env}{\loccx_{\stmt}}{\dynenv_i}{\rexpr'}{\typ}{\loccx}{\dynenv}.
    % %
    % By assumption we have $\eval{\hp_i}{\sbstate_i}{\bseq{\stmt}{\ee'}}
    % {\hp_o}{\sbstate_o}{\rexpr_o}$.
    % There are two cases:
    % \begin{itemize}
    %   \item \textbf{Rule \opskip} We have $\ee_o=\ee'$. We know the rule \tskip does not update
    %   the location context, thus $\loccx_s=\loccx_i$. We can satisfy the requirements in the conclusion
    %   by picking $\loccx_o=\loccx_i$ and $\dynenv_o=\dynenv_i$.
    %   \item \textbf{Rule \opseq:} We have (3) $\ee_o= \ee'$.
    % By inversion of \opseq, we have (4) \eval{\hp_i}{\sbstate_i}{\stmt}{\hp_o}{\sbstate_o}{\stmt_o}.
    % %
    % By assumption we also have (5) \statetyping[\varcx][\loccx_i][\dynenv]{\hp_i}{\sbstate_i}.
    % By (1), (4), (5), and Lemma~\ref{theorem:preservation:statement} we have (6)
    % \statetyping[\varcx][\loccx_{\stmt}][\dynenv']{\hp_o}{\sbstate_o} for some $\dynenv'\supseteq \dynenv_i$.
    % By weakening (Lemma~\ref{lemma:weakening}) and (2) we know
    % $$
    % \typing{\varcx}{\env}{\loccx_{\stmt}}{\dynenv'}{\rexpr'}{\typ}{\loccx}{\dynenv}.
    % $$
    % Thus, it suffices to pick $\loccx_o=\loccx_S$ and $\dynenv_o=\dynenv'$ to satisfy the conclusion.
    % \end{itemize}

  \item \textbf{Rule \tlet:}
  Let $\ee \equiv \blet{\xx}{\ee_{\xx}}{\ee'}$. By inversion of the rule we get:
  (1) \typing{\varcx}{\emptyset}{\loccx_i}{\dynenv_i}{\ee_{\xx}}{\typ_{\xx}}{\loccx_0}{\dynenv} and
  (2) \typing{\varcx}{\mapstoenv{\xx}{\typ_\xx}}{\loccx_0}{\dynenv_i}{\ee}{\typ}{\loccx}{\dynenv_o}.
Since \ee steps, there are two cases:

\begin{itemize}

    \item \textbf{Rule \oplet:}
    {\eval{\hp_i}{\sbstate_i}{\blet{\xx}{\val}{\rexpr'}}
    {\hp_i}{\sbstate_i}{\rexpr'[\val/\xx]}}.
    Since $\ee_{\xx} = \val$, by (1), (2), and Lemma~\ref{lemma:program-substitution-2}:
    \typing{\varcx}{\emptyset}{\loccx_i}{\dynenv_i}{\rexpr'[\val/\xx]}{\typ}{\loccx}{\dynenv}
    which concludes the proof.
    \item \textbf{Rule \opprop:}
    {\eval{\hp_i}{\sbstate_i}{\blet{\xx}{\ee_x}{\rexpr'}}
    {\hp_o}{\sbstate_o}{\blet{\xx}{\ee'_x}{\rexpr'}}}.
    By inversion:
    {\eval{\hp_i}{\sbstate_i}{\ee_x}
    {\hp_o}{\sbstate_o}{\ee'_x}}.
    By (1) and inductive hypothesis:
    there exists $\loccx_o$ and $\dynenv_o \supseteq \dynenv_i$, so that
    $\typing{\varcx}{\emptyset}{\loccx_o}{\dynenv_o}{\rexpr'_x}{\typ_x}{\loccx_0}{\dynenv}$
    and
    \statetyping[\varcx][\loccx_o][\dynenv_o]{\hp_o}{\sbstate_o}.
    By (2), weakened to $\dynenv_o$ using Lemma~\ref{lemma:weakening}, and rule \tlet:
    $\typing{\varcx}{\emptyset}{\loccx_o}{\dynenv_o}{\blet{\xx}{\ee'_{\xx}}{\ee'}}{\typ}{\loccx}{\dynenv}$,
    which concludes the proof.

  \end{itemize}

  \item \textbf{Rule \tcall:}
  Let $\ee \equiv \fcall{\ee'}{\overline{\typ}}{\overline{\expr}}{\overline{\aval}}$. By inversion of the rule we get:
  (0) \wf{\dynenv}
  (1) $\forall i. \typing{\varcx}{\emptyset}{\loccx}{\dynenv}{\aval_i}{\applysubst{\substvar}{\typ_{i}}}{\loccx}{}$,
  (2) \typing{\varcx}{\emptyset}{\loccx}{\dynenv}{\ee'}
         {\polysig{\overline{\tvar}}
                  {\overline{\aa: \sort}}
                  {\expr}
                  {\loccx_{i}}
                  {\overline{\typ}}
                  {\typ_o}
                  {\loccx_{o}}}
        {\loccx_1 * \loccx_2 }{\dynenv},
  (3) $ \substvar = \subst{\overline{\aa}}{\overline{\expr}}$,
  (4) \loccxinc{\varcx}{}{}{\loccx_1}{\applysubst{\substvar}{\loccx_{i}}},
  (5) $\forall i.\sortck{\expr_i}{\sort_i}$, and
  (6) \lmodel{\varcx}{\applysubst{\substvar}{\expr}}.

  Since \ee steps, we have the following cases:
  \begin{itemize}
    \item \textbf{Rule \opprop}:
      \eval{\hp_i}{\sbstate_i}{\fcall{\ee'}{\overline{\typ}}{\overline{\expr}}{\overline{\aval}}}
          {\hp_o}{\sbstate_o}{\fcall{\ee'_o}{\overline{\typ}}{\overline{\expr}}{\overline{\aval}}}.
      By inversion of the rule
      \eval{\hp_i}{\sbstate_i}{\ee'}
          {\hp_o}{\sbstate_o}{\ee'_o}.
      By this, (2), and inductive hypothesis
      there exist $\loccx'_o$ and $\dynenv_o \supseteq \dynenv$, so that
      (7) $
          \typing{\varcx}{\emptyset}{\loccx'_o}{\dynenv_o}{\rexpr'_o}{\polysig{\overline{\tvar}}
          {\overline{\aa: \sort}}
          {\expr}
          {\loccx_{i}}
          {\overline{\typ}}
          {\typ_o}
          {\loccx_{o}}}
      {\loccx_1 * \loccx_2 }{\dynenv}
          $ and
      (8) \statetyping[\varcx][\loccx'_o][\dynenv_o]{\hp_o}{\sbstate_o}.
      By Lemmas~\ref{lemma:aval},~\ref{lemma:weakening}, and (1):
      (9) $\forall i. \typing{\varcx}{\emptyset}{\loccx'_o}{\dynenv_o}{\aval_i}{\applysubst{\substvar}{\typ_{i}}}{\loccx'_o}{}$,
      By rule \tcall on (9), (7), (3), (4), (5), (6), and (0):
      \typing{\varcx}{\emptyset}{\loccx'_o}{\dynenv_o}
                    {\fcall{\ee'}{\overline{\typ}}{\overline{\expr}}{\overline{\aval}}}
                    {\applysubst{\substvar}{\typ_o}}{\applysubst{\substvar}{\loccx_{o}} * \loccx_2}{}.
      Which, combined with (7), concludes the proof.

    \item \textbf{Rule \opcall:}
      $$
      \eval{\hp}{\sbstate}{\fcall{(\vrec{\ff}{\overline{\aa}}{\overline{\xx}}{\rexpr_\ff})}{\overline{\typ}}{\overline{\expr}}{\overline{\val}}}
                {\hp}{\sbstate}{\rexpr_\ff[\vrec{\ff}{\overline{\aa}}{\overline{\xx}}{\rexpr_\ff}/\ff,\overline{\val}/\overline{\xx},\overline{\aa}/\overline{\expr}]}
      $$

      Since $\ee' \equiv \vrec{\ff}{\overline{\aa}}{\overline{\xx}}{\rexpr_\ff}$, by inversion of (2), we get:
      $$(7)\quad
      \typing{\varcx,\overline{\aa: \sort},\expr}
                    {\overline{\xx : \typ},
                      \ff: \polysig{\overline{\tvar}}{{\overline{\aa: \sort}}}
                                  {{\expr}}{\loccx_{i}}
                                  {\overline{\typ}}
                                  {{\typ}}
                                  {\loccx_{o}}
                      }
                    {\loccx_i}{\dynenv}
                    {\rexpr_\ff}
                    {\typ_o}{\loccx_o}
                    {}$$
      By Lemma~\ref{lemma:type-substitution} and (5):
      $$(8)\quad
      \typing{\varcx,\applysubst{\substvar}{\expr}}
                    {\overline{\xx : \applysubst{\substvar}{\typ}},
                      \ff: \applysubst{\substvar}{\polysig{\overline{\tvar}}{{\overline{\aa: \sort}}}
                                  {{\expr}}{\loccx_{i}}
                                  {\overline{\typ}}
                                  {{\typ}}
                                  {\loccx_{o}}}
                      }
                    {\applysubst{\substvar}{\loccx_i}}{\applysubst{\substvar}{\dynenv}}
                    {\applysubst{\substvar}{\rexpr_\ff}}
                    {\applysubst{\substvar}{\typ_o}}
                    {\applysubst{\substvar}{\loccx_o}}
                    {}$$
      The \substvar application is an identity in the type of the function (that is forall-quantified),
      and in $\dynenv$ (by (0) and lemma~\ref{lemma:wf-fv}).
      Further, by (6) and Lemma~\ref{lemma:condition} we remove logical condition $\applysubst{\substvar}{\expr}$:
      $$(9)\quad
      \typing{\varcx}
                    {\overline{\xx : \applysubst{\substvar}{\typ}},
                      \ff: {\polysig{\overline{\tvar}}{{\overline{\aa: \sort}}}
                                  {{\expr}}{\loccx_{i}}
                                  {\overline{\typ}}
                                  {{\typ}}
                                  {\loccx_{o}}}
                      }
                    {\applysubst{\substvar}{\loccx_i}}
                    {{\dynenv}}
                    {\applysubst{\substvar}{\rexpr_\ff}}
                    {\applysubst{\substvar}{\typ_o}}
                    {\applysubst{\substvar}{\loccx_o}}
                    {}$$
      By (1), (2), and Lemmata~\ref{lemma:program-substitution} and~\ref{lemma:aval}:
      $$(10)\quad
      \typing{\varcx}{\emptyset}
                    {\applysubst{\substvar}{\loccx_i}}
                    {{\dynenv}}
                    {\rexpr_\ff[\vrec{\ff}{\overline{\aa}}{\overline{\xx}}{\rexpr_\ff}/\ff,\overline{\val}/\overline{\xx},\overline{\aa}/\overline{\expr}]}
                    {\applysubst{\substvar}{\typ_o}}
                    {\applysubst{\substvar}{\loccx_o}}
                    {}$$
      By (4) and Lemma~\ref{lemma:conctext-inclusion}
      $$(11)\quad
      \typing{\varcx}{\emptyset}
                    {\loccx_1}
                    {{\dynenv}}
                    {\rexpr_\ff[\vrec{\ff}{\overline{\aa}}{\overline{\xx}}{\rexpr_\ff}/\ff,\overline{\val}/\overline{\xx},\overline{\expr}/\overline{\aa}]}
                    {\applysubst{\substvar}{\typ_o}}
                    {\applysubst{\substvar}{\loccx_o}}
                    {}$$

      Finally, by Lemma~\ref{lemma:framing}
      $$(12)\quad
      \typing{\varcx}{\emptyset}
                    {\loccx_1 * \loccx_2}
                    {{\dynenv}}
                    {\rexpr_\ff[\vrec{\ff}{\overline{\aa}}{\overline{\xx}}{\rexpr_\ff}/\ff,\overline{\val}/\overline{\xx},\overline{\expr}/\overline{\aa}]}
                    {\applysubst{\substvar}{\typ_o}}
                    {\applysubst{\substvar}{\loccx_o}* \loccx_2}
                    {}$$
      Which concludes the proof, because $\ee'$ is a value,
      thus $\loccx_1 * \loccx_2 = \loccx$ and by assumption
      \statetyping[\varcx][\loccx][\dynenv]{\hp}{\sbstate}.

       \item \textbf{Rule \opvecnew:}
        We have
        $$
        \eval
          {\hp_i}{\sbstate_i}
          {\fcall{\vecnew[\typ_v]}{}{}{}}
          {\hp_i}{\sbstate_i}
          {\vvec{0}{\poison}}
        $$
        Because the output state does not change we know it is still well-typed.
        By inversion of (2) we know $\subtyping{\rtyp{\tvec[\typ_v]}{0}}{\typ_o}$.
        We conclude by applying \tvecvec and \tsub to prove the result is also well-typed.

        \item \textbf{Rule \opvecpush:}
        We have
        $$
        \eval
          {\hp_i}{\sbstate_i}
          {\fcall{\vecpush[\typ_v]}{}{\cloc}{\vptr{\cloc}{\ptrtag}, \val}}
          {\hp_o}{\sbstate_o}
          {\poison}
        $$

        By inversion of (1) we get $\dynenv_i(\cloc, \ptrtag) = \tptr{\cloc}$ and
        \typing{\varcx}{\emptyset}{\loccx}{\dynenv_i}{\val}{\typ_v}{\loccx}{}.
        Then, by Lemma~\ref{lemma:vec:push} we get
        \statetyping[\varcx][(\cloc \mapsto \rtyp{\tvec[\typ_v]}{n + 1}), \loccx_2][\dynenv_o]{\hp_o}{\sbstate_o}.
        Finally, by inversion of (2) we get \subtyping{\uninit{1}}{\typ_o} and consequently
        by applying \tumem and \tsub the result is well-typed.

        \item \textbf{Rule \opvecpushempty:}
        We have
        $$
        \eval
          {\hp_i}{\sbstate_i}
          {\fcall{\vecpush[\typ_v]}{}{\cloc}{\vptr{\cloc}{\ptrtag}, \val}}
          {\hp_o}{\sbstate_o}
          {\poison}
        $$
        and by inversion of the rule we also have $\hp(\cloc) = \vptr{0}{\val'}$.
        By inversion of (1) we also have
        \typing{\varcx}{\emptyset}{\loccx}{\dynenv_i}{\val}{\typ_v}{\loccx}{},
        $\dynenv_i(\cloc, \ptrtag) = \tptr{\cloc}$ and
        \subtyping{\uninit{1}}{\typ_o}.
        We pick $\dynenv_o = \dynenv_i, (\cloc', \ptrtag')\mapsto \tref{\mut}{\typ_v}$.
        By Lemma~\ref{lemma:vec:push-empty} we get
        \statetyping[\varcx][\cloc\mapsto \rtyp{\tvec[\typ_v]}{1}, \loccx_2][\dynenv_o]{\hp_o}{\sbstate_o}.
        We conclude by applying \tumem and \tsub to prove the result is well-typed.

        \item \textbf{Rule \opvecindexmut:}
        We have
        $$
        \eval
          {\hp_i}{\sbstate_i}
          {\fcall{\vecindexmut[\typ_v]}{}{}{\vptr{\cloc}{\ptrtag}, i}}
          {\hp_i}{\sbstate_o}
          {\vptr{\cloc' + i}{\ptrtag''}}
        $$
        By inversion of (1) we have $\dynenv_i(\cloc, \ptrtag) = \tref{\mut}{\rtyp{\tvec[\typ_v]}{n}}$.
        Therefore, by well-typedness of the input state and Lemma~\ref{lemma:event:read} we have
        (6) \typing{\varcx}{\emptyset}{\emptyset}{\dynenv}{\hp(\cloc)}{\rtyp{\tvec[\typ_v]}{n}}{\emptyset}{}.
        Then, by lemmas~\ref{lemma:canonical:vec} and \ref{lemma:value-refinement} we have $\hp(\cloc)=\vvec{n}{\val}$.
        There are two cases:
        \begin{itemize}
            \item $n=0$. This case is impossible because by (6) $\entailment{\varcx}{0\leq i < 0}$ would need to hold
            which is impossible.
            \item $n > 0$.
            By inversion of \tvecvec we have $\val=\vptr{\cloc'}{\ptrtag'}$.
            We conclude by picking $\dynenv_o=\dynenv,(\cloc', \ptrtag')\mapsto \tref{\mut}{\typ_v}$ and
            applying Lemma~\ref{lemma:vec:indexmut}.
        \end{itemize}
    \end{itemize}

      \item \textbf{Rule \ttvar:} Impossible because the typing environment \env is empty.
    \item \textbf{Rule \tunpack:} Impossible because the typing environment \env is empty.
    \item \textbf{Rules \ttrue, \tfalse, \tconstint, \tfun, \ttptr, \tumem:}
          These cases are trivial, since the expressions do not step.

    % \item \textbf{Case \tskip:} Impossible because \sskip cannot take a step.

    \item \textbf{Case \tassign:} Let $\ee=\sassign{\place}{\ee_0}$.
    Since $\ee$ steps we have two options
    By inversion of the rule we have
    \begin{enumerate}
      \item \rvaltyping{\varcx}{\emptyset}{\loccx_i}{\dynenv_i}{\ee_0}{\typ_v}{\loccx},
      \item \pltyping{\varcx}{\emptyset}{\loccx_i}{\dynenv_i}{\place}{\tref{\mut}{\typ}}{\loccx_i}
      \item \subtyping{\typ_v}{\typ}.
    \end{enumerate}
    Since $\ee$ takes a step there are two options:
    \begin{itemize}
        \item \textbf{Case \opprop:}
        By inversion of the rule we have \eval{\hp_i}{\sbstate_i}{\ee_0}{\hp_o}{\sbstate_o}{\ee_1}
        and $\ee_o=\sassign{\place}{\ee_2}$.
        By inductive hypothesis on (1) there exists $\dynenv_o$ and $\loccx_o$ such that
        \begin{enumerate}
          \item \valtyping{\varcx}{\emptyset}{\loccx_o}{\dynenv'}{\ee_1}{\typ_v}
          \item \statetyping[\varcx][\loccx_o][\dynenv']{\hp_o}{\sbstate_o}
        \end{enumerate}
        We conclude by applying \tassign to prove
        \typing{\varcx}{\emptyset}{\loccx_o}{\dynenv_o}{\sassign{\place}{\ee_o}}{\uninit{1}}{\loccx}{}.

        \item \textbf{Case \opass:} Let $\ee=\sassign{\vptr{\cloc}{\ptrtag}}{\val}$,
        $\ee_o=\poison$ and $\hp_o=\hp_i\hbind{\cloc}{\val}$.
        Replacing $\vptr{\cloc}{\ptrtag}$ for $\place$ in (2) we also get
        $\dynenv(\cloc,\ptrtag)=\tref{\mut}{\typ}$.
        By using (1), (3) and subsumption we get
        \valtyping{\varcx}{\emptyset}{\loccx_i}{\dynenv_i}{\val}{\typ}.
        Let us pick $\loccx_o=\loccx$ and $\dynenv_o=\dynenv_i$.
        We get the first part of the conclusion by applying \tumem.
        We conclude by applying Lemma~\ref{lemma:event:weak-write}.
    \end{itemize}
    \item \textbf{Case \tassignstrg:} Let $\ee=\sassign{\place}{\ee_0}$.
    By inversion of the rule we have
    \begin{enumerate}
      \item \rvaltyping{\varcx}{\emptyset}{\loccx_i}{\dynenv_i}{\ee_0}{\typ}{\loccx'} and
      \item $\loccx=\loccx'[\cloc\mapsto\typ]$.
    \end{enumerate}
    Since $\ee$ takes a step there are two options:
    \begin{itemize}
        \item \textbf{Case \opprop:} The proof is similar to the \opprop case
        for the \tassign case by applying the inductive hypothesis.

        \item \textbf{Case \opass:} Let $\ee=\sassign{\vptr{\cloc}{\ptrtag}}{\val}$,
        $\ee_o=\poison$ and $\hp_o=\hp_i\hbind{\cloc}{\val}$.
        Replacing $\vptr{\cloc}{\ptrtag}$ for $\place$ in (2) we also get
        $\dynenv(\cloc,\ptrtag)=\tptr{\cloc}$.
        Let us pick $\loccx_o=\loccx'$ and $\dynenv_o=\dynenv_i$.
        We conclude by applying Lemma~\ref{lemma:event:strg-write}
    \end{itemize}

    \item \textbf{Case \tstrgrebor:} Let $\ee=\rvstrgref{\place}$ and $T_o = T_i$.
    Since $\ee$ takes a step then the \opstrgrebor{} must have been applied and thus we know
    $\place = \vptr{\cloc}{\ptrtag}$ and $\ee_o=\vptr{\cloc}{\ptrtag'}$.
    By inversion of the typing rule we know that
    \pltyping{\varcx}{\emptyset}{\loccx_o}{\dynenv_i}{\vptr{\cloc}{\ptrtag}}{\tptr{\cloc}}{\loccx_o}
    and consequently $\dynenv_i(\cloc,\ptrtag)=\tptr{\cloc}$.
    Picking $\dynenv_o=\dynenv_i,\mapstoowned{(\cloc,\ptrtag')}{\tptr{\cloc}}$ we directly
    \pltyping{\varcx}{\emptyset}{\loccx_o}{\dynenv_i}{\vptr{\cloc}{\ptrtag'}}{\tptr{\cloc}}{\loccx_o}.
    We conclude by Lemma~\ref{lemma:event:strg-rebor} to prove the output state is well-typed.

    \item \textbf{Case \tstrgmutrebor:} Since $\ee$ takes a step then \opmutrebor{} must have been
    applied and we know $\ee=\rvmutref{\vptr{\cloc}{\ptrtag}}$ and $\ee_o=\vptr{\cloc}{\ptrtag'}$.
    We also know $\loccx_o=\loccx_i[\cloc\mapsto\typ]$.
    By inversion of the typing rule we have that
    (1) \pltyping{\varcx}{\emptyset}{\loccx_o}{\dynenv_i}{\vptr{\cloc}{\ptrtag}}{\tptr{\cloc}}{\loccx_o}
    and \subtyping{\loccx_i(\cloc)}{\typ}.
    By (1) we also know $\dynenv_i(\cloc, \ptrtag) = \tptr{\cloc}$.
    If we pick $\dynenv_o=\dynenv_i,\mapstoowned{(\cloc, \ptrtag')}{\tref{\mut}{\typ}}$
    we get directly
    \pltyping{\varcx}{\emptyset}{\loccx_o}{\dynenv_i}{\vptr{\cloc}{\ptrtag'}}{\tref{\mut}{\typ}}{\loccx_o}.
    We conclude by applying Lemma~\ref{lemma:event:weaken-rebor} to prove the output state is well-typed.

    \item \textbf{Case \tmutmutrebor:} Since $\ee$ takes a step then \opmutrebor{} must have been applied,
    thus we know $\ee=\rvmutref{\vptr{\cloc}{\ptrtag}}$ and $\ee_o=\vptr{\cloc}{\ptrtag'}$.
    We also know $T=T_i$.
    By inversion of the typing rule we know that
    \pltyping{\varcx}{\emptyset}{\loccx_i}{\dynenv_i}{\vptr{\cloc}{\ptrtag}}{\tref{\mut}{\typ}}{\loccx_i}
    and consequently $\dynenv_i(\cloc, \ptrtag)=\tref{\mut}{\typ}$.
    By definition of \statetyping[\varcx][\loccx_i][\dynenv_i]{\hp_i}{\sbstate_i} we know
    \subtyping{\typ}{\loccx_i(\cloc)}{\typ} and \valtyping{\varcx}{\emptyset}{\emptyset}{\dynenv_i}{\hp(\cloc)}{\typ}.
    We conclude picking $\dynenv_o=\dynenv_i,\mapstoowned{(\cloc, \ptrtag')}{\tref{\mut}{\typ}}$ and applying
    Lemma~\ref{lemma:event:mut-rebor}.

    \item \textbf{Case \tshrrebor:}
    Since \ee takes a step then \opshrrebor must have been applied.
    Therefore, $\ee=\rvshrref{\vptr{\cloc}{\ptrtag}}$ and $\ee_o=\vptr{\cloc}{\ptrtag'}$.
    We also know $\loccx=\loccx_i$ and by inversion of the typing rule we have
    (1) \pltyping{\varcx}{\emptyset}{\loccx_i}{\dynenv_i}{\vptr{\cloc}{\ptrtag}}{\tref{\bormode}{\typ'}}{\loccx_i} and (2)
    \subtyping{\typ'}{\typ}.
    By (1) we also have $\dynenv_i(\cloc, \ptrtag)=\tref{\bormode}{\typ'}$.
    Since the input stack is well-typed we know \subtyping{\loccx_i(\cloc)}{\typ'} and
    and transitivity of subtyping we have \subtyping{\loccx_i(\cloc)}{\typ}.
    We pick $\dynenv_o=\dynenv_i(\cloc,\ptrtag')\mapsto \tref{\shr}{\typ}$ and conclude
    applying Lemma~\ref{lemma:event:shr-rebor}.

    \item \textbf{Case \tderef:} Since $\ee$ takes a step then \opderef must have been applied,
    therefore $\ee=\deref{\vptr{\cloc}{\ptrtag}}$ and $\ee_o=\hp(\cloc)$.
    By inversion of the typing rule we know
    $\pltyping{\varcx}{\emptyset}{\loccx_i}{\dynenv_i}{\vptr{\cloc}{\ptrtag}}{\tref{\bormode}{\typ}}{\loccx_i}$
    and consequently $\dynenv_i(\cloc, \ptrtag)=\tref{\bormode}{\typ}$.
    We pick $\dynenv_o=\dynenv_i$ and conclude by applying Lemma~\ref{lemma:event:read} to pove
    the output state is well-typed.

    \item \textbf{Case \tderefstrg:}
    Since $\ee$ takes a step then \opderef must have been applied, therefore
    $\ee=\deref{\vptr{\cloc}{\ptrtag}}$ and $\ee_o=\hp(\cloc)$.
    By inversion of the typing rule we know
    $\pltyping{\varcx}{\emptyset}{\loccx_i}{\dynenv_i}{\vptr{\cloc}{\ptrtag}}{\tptr{\cloc}}{\loccx_i}$
    and $\loccx(\cloc)=\typ$.
    Consequently, we know $\dynenv_i(\cloc,\ptrtag)=\tptr{\cloc}$.
    We pick $\dynenv_o=\dynenv_i$ and conclude by applying Lemma~\ref{lemma:event:strg-read}.
\end{itemize}
\end{proof}

\input{metatheory/proofs/stmt-preservation}

\clearpage
\subsection{Proof of progress}
\progress*
\begin{proof}
By induction on the type derivation tree \typing{\emptyset}{\emptyset}{\loccx_i}{\dynenv_i}{\rexpr}{\typ}{\loccx_o}{\dynenv_o}.
\begin{itemize}
    \item \textbf{Rule \tsub:}
    By inversion of the rule we get
    \typing{\emptyset}{\emptyset}{\loccx_i}{\dynenv_i}{\rexpr}{\typ_1}{\loccx_o}{\dynenv_o}
    at which we apply the inductive hypothesis.

    \item \textbf{Rule \tlet:}
    Let $\ee \equiv  \blet{\xx}{\ee_\xx}{\ee'}$.
    By inversion of the rule,
    \typing{\emptyset}{\env}{\loccx_i}{\dynenv_i}{\ee_{\xx}}{\typ_{\xx}}{\loccx}{\dynenv}.
    By inductive hypothesis, there are three cases:
    (1) If $\ee_{\xx}$ is a value, the \oplet rule applies with $\hp_i$ and  $\sbstate_i$;
    (2) If $\evalerr{\hp_i}{\sbstate_i}{\rexpr_\xx}$, then, by rule \opproperr,
    $\evalerr{\hp_i}{\sbstate_i}{\rexpr}$; and
    (3) If $\eval{\hp_i}{\sbstate_i}{\rexpr_\xx}{\hp_o}{\sbstate_o}{\ee'_\xx}$,
    then, by rule \opprop,
    $\eval{\hp_i}{\sbstate_i}{\blet{\xx}{\ee_\xx}{\ee'}}{\hp_o}{\sbstate_o}{\blet{\xx}{\ee'_\xx}{\ee'}}$.
    \item \textbf{Rule \tnew:}
    Let $\ee \equiv \blet{\xx}{\new{\lvar}}{\rexpr'}$.
    One of the rules \opnew or \opnewerr applies.
    \item \textbf{Rule \tif:}
    Let $\ee \equiv  \bif{\ee'}{\ee_1}{\ee_2}$.
    By inversion of the rule,
    \typing{\emptyset}{\env}{\loccx_i}{\dynenv_i}{\ee'}{\rtyp{\tbool}{\expr}}{\loccx_o}{\dynenv_o}.
    By inductive hypothesis, there are three cases:
    (1) If $\ee'$ is a value, then, by Lemma~\ref{lemma:canonical:bool},
    it is either \ctrue or \cfalse and one of the  \opifTrue or \opifFalse rules applies with $\hp_i$ and  $\sbstate_i$;
    (2) If $\evalerr{\hp_i}{\sbstate_i}{\rexpr'}$, then, by rule \opproperr,
    $\evalerr{\hp_i}{\sbstate_i}{\rexpr}$; and
    (3) If $\eval{\hp_i}{\sbstate_i}{\rexpr'}{\hp_o}{\sbstate_o}{\ee''}$,
    then, by rule \opprop,
    $\eval{\hp_i}{\sbstate_i}{\ee}{\hp_o}{\sbstate_o}{\bif{\ee''}{\ee_1}{\ee_2}}$.
    \item \textbf{Rule \tseq:}
    Let $\ee \equiv \bseq{\stmt}{\rexpr'}$.
    By inversion of the rule we get:
    \stmtyping{\emptyset}{\emptyset}{\loccx_i}{\dynenv_i}{\stmt}{\loccx_{\stmt}}{\dynenv_{\stmt}}.
    By assumption we have \statetyping[\emptyset][\loccx_i][\dynenv_i]{\hp_i}{\sbstate_i}.
    By Lemma~\ref{lemma:progress-stmt}, we have that
    either (1)
there exists $\hp_o, \sbstate_o$ such that \evalstm{\hp_i}{\sbstate_i}{\stmt}{\hp_o}{\sbstate_o},
(2) \evalstmerr{\hp_i}{\sbstate_i}{\stmt} or (3) $\stmt_i=\sskip$.
In case (1) and by rule \opseq,
there exists $\hp_o, \sbstate_o$ such that
\eval{\hp_i}{\sbstate_i}{\bseq{\stmt}{\rexpr'}}
          {\hp_o}{\sbstate_o}{\rexpr'}.
In case (2) and by rule \opseqerr,
\evalerr{\hp_i}{\sbstate_i}{\bseq{\stmt}{\rexpr'}}.
Finally, in case (3) \opskip applies.

    \item \textbf{Rule \tcall:}
    Let $\ee \equiv \fcall{\ee'}{\overline{\typ}}{\overline{\expr}}{\overline{\aval}}$.
    By inversion of the rule,
    \typing{\emptyset}{\env}{\loccx_i}{\dynenv_i}{\ee'}{\polysig{\overline{\tvar}}{\overline{\aa: \sort}}
    {\expr}
    {\elftcx}{\overline{\xx : \typ}}{\overline{\loc}}{\loccx_{fi}}
    {\typ}{\loccx_{fo}}}{\loccx}{\dynenv}.
    By inductive hypothesis, there are three cases:
    (1) If $\evalerr{\hp_i}{\sbstate_i}{\rexpr'}$, then, by rule \opproperr,
    $\evalerr{\hp_i}{\sbstate_i}{\rexpr}$; and
    (2) If $\eval{\hp_i}{\sbstate_i}{\rexpr'}{\hp_o}{\sbstate_o}{\ee''}$,
    then, by rule \opprop,
    $\eval{\hp_i}{\sbstate_i}{\ee}{\hp_o}{\sbstate_o}{\fcall{\ee''}{\overline{\typ}}{\overline{\expr}}{\overline{\aval}}}$.
    (3) If $\ee'$ is a value, then, by Lemma~\ref{lemma:canonical:fun} we have the following cases
    \begin{itemize}
        \item $e' = \vrec{f}{\overline{\expr'}}{\overline{\yy}}{\expr_b}$.
        Arguments are a-values and by inversion of typing under the empty environment,
        they must be values, thus rule \opcall applies.
        \item $e' = \vecnew[\typ_v]$. In this case \opvecnew applies.
        \item $e' = \vecpush[\typ_v]$. Let $\val_1$ and $\val_2$ be the two arguments of the function call.
        By inversion of \tcall we have:
        \begin{enumerate}
            \item \typing{\emptyset}{\emptyset}{\loccx_i}{\dynenv_i}{\val_1}{\tptr{\cloc}}{\loccx_i}{}
            \item \typing{\emptyset}{\emptyset}{\loccx_i}{\dynenv_i}{\val_2}{\typ_v}{\loccx_i}{}
            \item \loccxinc{\emptyset}{}{}{\loccx_1}{\cloc \mapsto \rtyp{\tvec[\typ_v]}{n}}.
        \end{enumerate}
        By lemmas \ref{lemma:canonical:ptr} and \ref{lemma:canonical:int} we know $\val_1 = \vptr{\cloc}{\ptrtag}$.
        Since the input state is well-typedness we have by (3) that $\cloc \in \dom{\hp}$ and
        \typing{\emptyset}{\emptyset}{\emptyset}{\dynenv_i}{\hp(\cloc)}{\rtyp{\tvec[\typ_v]}{n}}{\emptyset}{}.
        By lemmas~\ref{lemma:canonical:vec} and \ref{lemma:value-refinement} we know $\hp(\cloc) = \vptr{n}{\val'}$.
        If $n=0$ then \opvecpushempty applies.
        If $n > 0$ then $\val' = \vptr{\cloc'}{\ptrtag'}$ and $\forall j \in [0, n). \cloc' + j \in \dom{\hp}$
        and \opvecpush applies.
        \item $e' = \vecindexmut[\typ_v]$. Let $\val_1$ and $\val_2$ be the two arguments of the function call.
        By inversion of \tcall we have:
        \begin{enumerate}
            \item \typing{\emptyset}{\emptyset}{\loccx_i}{\dynenv_i}{\val_1}{\tref{\mut}{\rtyp{\tvec[\typ_v]}{n}}}{\loccx_i}{}
            \item \typing{\emptyset}{\emptyset}{\loccx_i}{\dynenv_i}{\val_2}{\rtyp{\tint}{m}}{\loccx_i}{}
            \item \entailment{\emptyset}{0 \leq m < n}
        \end{enumerate}
        By lemmas \ref{lemma:canonical:ptr} and \ref{lemma:canonical:int} we have
        $\val_1 = \vptr{\cloc}{\ptrtag}$ and $\val_2 = z$.
        By Lemma~\ref{lemma:value-refinement} and (2) we have $z = m$, and by (3) we have (4) $0\leq z < n$.
        By well-formedness of the input state and (1) we have
        \typing{\emptyset}{\emptyset}{\loccx_i}{\dynenv_i}{\hp(\cloc)}{\rtyp{\tvec[\typ_v]}{n}}{\loccx_i}{}
        and by lemmas~\ref{lemma:canonical:vec} and \ref{lemma:value-refinement} we have $\hp(\cloc) = \vvec{n}{\val'}$.
        The case $n=0$ is impossible because (4) must hold.
        Since $n>0$, by inversion of \tvecvec we have $\val'= \vptr{\cloc'}{\ptrtag'}$ and $\cloc' + i \in \dom{\dynenv_i}$
        for all $0 \leq i < n$.
        By well-typeness of the input state we have $\dom{\dynenv_i} = \dom{\hp}$ and consequently $\cloc' + z \in \dom{\hp}$.
        Therefore, the rule \opvecindexmut applies, and we conclude the proof.
    \end{itemize}

    \item \textbf{Rule \ttvar:} Impossible because the typing environment \env is empty.

    \item \textbf{Rule \tunpack:} Impossible because the typing environment \env is empty.

    \item \textbf{Rules \ttrue, \tfalse, \tconstint, \tfun, \ttptr, and \tumem:} \ee is a value.

    \item \textbf{Case \tassign,\tassignstrg:} We have $\ee=\sassign{\place}{\ee'}$.
    Since the statement must be close since we are in an empty environment we have $\place=\vptr{\cloc}{\ptrtag}$.
    If $\ee'=\val$ then either stacked borrow transition in the premise of \opass holds and we take a step, or
    it does not hold and we step to an error by rule \opproperr.
    If $\ee'$ is not a value then by inductive hypothesis either takes a step or goes to an error
    in either case we make progress by rule \opassrval{} or \opasserr.

    \item \textbf{Case \tstrgrebor:} $\ee=\rvstrgref{\place}$. We know $p$ must be equal to $\vptr{\cloc}{\ptrtag}$
    because we are in an empty environment, thus either \opstrgrebor applies or we step to an error
    if the stacked borrow transition does not hold.

    \item \textbf{Case \tstrgmutrebor,\tmutmutrebor:} $\ee=\rvmutref{\place}$.
    We know $p$ must be equal to $\vptr{\cloc}{\ptrtag}$ because we are in an empty environment,
    thus either \opmutrebor applies or we step to an error if the stacked borrow transition does not hold.

    \item \textbf{Case \tshrrebor:} $\ee=\rvshrref{\place}$. We know $p$ must be equal to
    $\vptr{\cloc}{\ptrtag}$ because we are in an empty environment,
    thus either \opshrrebor applies or we step to an error if the stacked borrow transition does not hold.

    \item \textbf{Case \tderef,\tderefstrg:} $\ee=\deref{\place}$. We know $p$ must be equal to
    $\vptr{\cloc}{\ptrtag}$ because we are in an empty environment.
    If the stacked borrow transition in the premise of \opderef holds then \cloc must be in $\dom{\sbstate\dotstacks}$.
    Then, by well-typedness of the input state we have that $\cloc \in \dom{\hp}$ and the rule \opderef applies.
    If the stacked borrow transition does not hold then we step to an error.
    \end{itemize}
\end{proof}

\clearpage
\subsection{Lemmata}
\begin{lemma}[Subtyping Transitive]\label{lemma:subtype:trans}
  If \wf{\typ_1}, then
  if \subtyping{\typ_1}{\typ_2} and \subtyping{\typ_2}{\typ_3},
  then \subtyping{\typ_1}{\typ_3}.
\end{lemma}
\begin{proof}
By induction on the structure of the three types.
We split cases on $\typ_1$
\begin{itemize}
  \item $\typ_1 \equiv \rtyp{\tcon}{\expr_1}$.
  Then, the left rule can be either \subrtyp or \subexists.
  \begin{itemize}
  \item \textbf{Left rule is \subrtyp.}
    Then $\typ_2 \equiv \rtyp{\tcon}{\expr_2}$ and we know
    (1) $\subtyping
    {\rtyp{\tcon}{\expr_1}}
    {\rtyp{\tcon}{\expr_2}}$.
   The right rule can be either \subrtyp or \subexists.
    \begin{itemize}
      \item \textbf{Right rule is \subrtyp.}
      Then $\typ_3 \equiv \rtyp{\tcon}{\expr_3}$ and we know
      (2) $\subtyping
      {\rtyp{\tcon}{\expr_2}}
      {\rtyp{\tcon}{\expr_3}}$.
      By inversion of (1) and (2) we get:
      (3) \entailment{\varcx}{\expr_1 = \expr_2} and
      (4) \entailment{\varcx}{\expr_2 = \expr_3}.
      By (3), (4), and assumption~\ref{assumption:model:transitive}, we have
      (5) \entailment{\varcx}{\expr_1 = \expr_3}.
      By rule~\subrtyp we conclude the proof.
      \item \textbf{Right rule is \subexists.}
      Then $\typ_3 \equiv \texists{\aa}{\rtyp{\tcon}{\aa}}{\expr_3}$ and we know
      (2) \subtyping
      {\rtyp{\tcon}{\expr_2}}
      {\texists{\aa}{\rtyp{\tcon}{\aa}}{\expr_3}}.
      By inversion of (1) and (2) we get
      (3) \entailment{\varcx}{\expr_1 = \expr_2} and
      (4) \entailment{\varcx}{\expr_3[\expr_2/\aa]}.
      By (3), (4), and assumption~\ref{assumption:model:congruence}, we get
      (5) \entailment{\varcx}{\expr_3[\expr_1/\aa]},
      which concludes the proof by rule~\subexists.
    \end{itemize}
  \item \textbf{Left rule is \subexists.}
  Then $\typ_2 \equiv \texists{\aa}{\rtyp{\tcon}{\aa}}{\expr_2}$ and we know
  (1) $\subtyping
  {\rtyp{\tcon}{\expr_1}}
  {\texists{\aa}{\rtyp{\tcon}{\aa}}{\expr_2}}$.
 The right rule can only be \subunpack:
 (2) \subtyping
 {\texists{\aa}{\rtyp{\tcon}{\aa}}{\expr_2}}
 {\typ_3}.
 By inversion of (2):
 (3) \subtyping[\varcx, \aa: \getsort{\tcon}, \expr_2]
                {\rtyp{\tcon}{\aa}}
                {\typ_3}.
 Thus, $\typ_3$ can be either singleton or existential
 and, respectively, the applied rules are
 can be either \subrtyp or \subexists.
    \begin{itemize}
      \item \textbf{Right inverted rule is \subrtyp.}
      Then $\typ_3 \equiv \rtyp{\tcon}{\expr_3}$ and we know
      $$(4) \subtyping[\varcx, \aa: \getsort{\tcon}, \expr_2]
                {\rtyp{\tcon}{\aa}}
                {\rtyp{\tcon}{\expr_3}}$$
      Since by assumption, \wf{\typ_1}, \sortck[\varcx]{\expr_1}{\getsort{\tcon}}
      by which and lemma~\ref{lemma:type-substitution}, from (4) we get:
      $$(5) \subtyping[\varcx, \expr_2\subst{\aa}{\expr_1}]
                {\rtyp{\tcon}{\expr_1}}
                {\rtyp{\tcon}{\expr_3}}$$
      By inversion of (1) we know that \entailment{\varcx}{\expr_2[\expr_1/\aa]},
      by which and lemma~\ref{lemma:condition} we get
      $$(6) \subtyping[\varcx]
                {\rtyp{\tcon}{\expr_1}}
                {\rtyp{\tcon}{\expr_3}}$$
      Which concludes the proof.
      \item \textbf{Right inverted rule is \subexists.}
      Then $\typ_3 \equiv \texists{\aa}{\rtyp{\tcon}{\aa}}{\expr_3}$ and we know
      $$(4) \subtyping[\varcx, \aa: \getsort{\tcon}, \expr_2]
                {\rtyp{\tcon}{\aa}}
                \texists{\aa}{\rtyp{\tcon}{\aa}}{\expr_3}$$
      By inversion:
      $$ (5) \entailment{\varcx, \aa: \getsort{\tcon}, \expr_2}{\expr_3}$$
      Since by assumption, \wf{\typ_1}, \sortck[\varcx]{\expr_1}{\getsort{\tcon}}
      by which and assumption~\ref{assumption:model:substitution}, we get:
      $$ (6) \entailment{\varcx, \expr_2[\expr_1/\aa]}{\expr_3[\expr_1/\aa]}$$
      By inversion of (1) we know that \entailment{\varcx}{\expr_2[\expr_1/\aa]},
      by which and assumption~\ref{assumption:model:cut} we get
      $$ (7) \entailment{\varcx}{\expr_3[\expr_1/\aa]}$$
      Which concludes the proof by rule \subexists.
    \end{itemize}
\end{itemize}

  \item $\typ_1 \equiv \texists{\aa}{\rtyp{\tcon}{\aa}}{\expr_1}$.
  The left rule is \subunpack:
  (1) \subtyping
  {\texists{\aa}{\rtyp{\tcon}{\aa}}{\expr_1}}
  {\typ_2}.
  By inversion:
  (2) \subtyping
  [\varcx, \aa: \getsort{\tcon}, \expr_1]
  {\rtyp{\tcon}{\aa}}
  {\typ_2}. So, the inverted right rule can be either \subrtyp or \subexists:
  \begin{itemize}
    \item \textbf{Left inverted rule is \subrtyp.}
    Then, $\typ_2 \equiv \rtyp{\tcon}{\expr_2}$ and we know:
    (3): \subtyping
    [\varcx, \aa: \getsort{\tcon}, \expr_1]
    {\rtyp{\tcon}{\aa}}
    {\rtyp{\tcon}{\expr_2}}.
    By inversion:
    (4): \entailment{\varcx, \aa: \getsort{\tcon}, \expr_1}{\aa = \expr_2}.
    Since \subtyping{\rtyp{\tcon}{\expr_2}}{\typ_3}, the right rule can be
    either \subrtyp or \subexists:
    \begin{itemize}
      \item \textbf{Right rule is \subrtyp.}
      Then, $\typ_3 \equiv \rtyp{\tcon}{\expr_3}$ and we know:
      (5): \subtyping
      [\varcx]
      {\rtyp{\tcon}{\expr_2}}
      {\rtyp{\tcon}{\expr_3}}.
      By inversion: (6) \entailment{\varcx}{\expr_2 = \expr_3}.
      By assumption~\ref{assumption:model:equality} and (6), (4) becomes:
      (7) \entailment{\varcx, \aa: \getsort{\tcon}, \expr_1}{\aa = \expr_3}.
      By (7) and rule \subrtyp:
      \subtyping[\varcx, \aa: \getsort{\tcon}, \expr_1]
                {\rtyp{\tcon}{\aa}}
                {\rtyp{\tcon}{\expr_3}},
                which concludes the proof by rule \subunpack.
      \item \textbf{Right rule is \subexists.}
      Then $\typ_3 \equiv \texists{\aa_3}{\rtyp{\tcon}{\aa_3}}{\expr_3}$ and we know
      (5) \subtyping
                {\rtyp{\tcon}{\expr_2}}
                {\texists{\aa_3}{\rtyp{\tcon}{\aa_3}}{\expr_3}}.
      By inversion:
      (6) \entailment{\varcx}{\expr_3[\expr_2/\aa_3]}.
      By assumption~\ref{assumption:model:weakening} on (6):
      (7) \entailment{\varcx, \aa: \getsort{\tcon}, \expr_1}{\expr_3[\expr_2/\aa_3]}.
      By (4) and assumption~\ref{assumption:model:equality}
      (8) \entailment{\varcx, \aa: \getsort{\tcon}, \expr_1}{\expr_3[\aa/\aa_3]}.
      By rule \subexists
      \subtyping[\varcx, \aa: \getsort{\tcon}, \expr_1]{\rtyp{\tcon}{\aa}}{\texists{\aa_3}{\rtyp{\tcon}{\aa_3}}{\expr_3}}.
      The proof concludes by rule \subunpack.
    \end{itemize}
    \item \textbf{Left inverted rule is \subexists.}
    Then $\typ_2 \equiv \texists{\aa_2}{\rtyp{\tcon}{\aa_2}}{\expr_2}$ and we know
    (3) \subtyping
    [\varcx, \aa: \getsort{\tcon}, \expr_1]
    {\rtyp{\tcon}{\aa}}
    {\texists{\aa_2}{\rtyp{\tcon}{\aa_2}}{\expr_2}}.
    By inversion,
    (4) \entailment{\varcx, \aa: \getsort{\tcon}, \expr_1}{\expr_2[\aa/\aa_2]}.
    The right rule is \subunpack and by inversion we get:
    (5) \subtyping
    [\varcx, \aa_2: \getsort{\tcon}, \expr_2]
    {\rtyp{\tcon}{\aa_2}}
    {\typ_3}. Thus the right inverted rule can be either \subrtyp or \subexists.
    \begin{itemize}
      \item\textbf{Right inverted rule is \subrtyp.}
      Then $\typ_3 \equiv \rtyp{\tcon}{\expr_3}$ and we know
      \subtyping[\varcx, \aa_2: \getsort{\tcon}, \expr_2]{\rtyp{\tcon}{\aa_2}}{\rtyp{\tcon}{\expr_3}}.
      By inversion:
      (6) \entailment{\varcx, \aa_2: \getsort{\tcon}, \expr_2}{\aa_2 = \expr_3}.
      By (6) and assumption~\ref{assumption:model:weakening}:
      (7) \entailment{\varcx, \aa: \getsort{\tcon}, \expr_1, \aa_2: \getsort{\tcon}, \expr_2}{\aa_2 = \expr_3}.
      By assumption~\ref{assumption:model:substitution}:
      (8) \entailment{\varcx, \aa: \getsort{\tcon}, \expr_1, \expr_2[\aa/\aa_2]}{\aa = \expr_3}.
      By (4) and assumption~\ref{assumption:model:cut}:
      (9) \entailment{\varcx, \aa: \getsort{\tcon}, \expr_1}{\aa = \expr_3}.
      By rule ~\subrtyp:
      (10) \subtyping[\varcx, \aa: \getsort{\tcon}, \expr_1]
                {\rtyp{\tcon}{\aa}}
                {\rtyp{\tcon}{\expr_3}}.
      Then, rule~\subunpack concludes the proof.
      \item\textbf{Right inverted rule is \subexists.}
      Then $\typ_3 \equiv \texists{\aa_3}{\rtyp{\tcon}{\aa_3}}{\expr_3}$
      and we know \subtyping
      [\varcx, \aa_2: \getsort{\tcon}, \expr_2]
      {\rtyp{\tcon}{\aa_2}}
      {\texists{\aa_3}{\rtyp{\tcon}{\aa_3}}{\expr_3}}.
      By inversion:
      (6) \entailment{\varcx, \aa_2: \getsort{\tcon}, \expr_2}{\expr_3[\aa_2/\aa_3]}.
      By (6) and assumption~\ref{assumption:model:weakening}:
      (7) \entailment{\varcx, \aa: \getsort{\tcon}, \expr_1, \aa_2: \getsort{\tcon}, \expr_2}{\expr_3[\aa_2/\aa_3]}.
      By assumption~\ref{assumption:model:substitution}:
      (8) \entailment{\varcx, \aa: \getsort{\tcon}, \expr_1, \expr_2[\aa/\aa_2]}{\expr_3[\aa_2/\aa_3][\aa/\aa_2]}.
      By (4) and assumption~\ref{assumption:model:cut}:
      (9) \entailment{\varcx, \aa: \getsort{\tcon}, \expr_1}{\expr_3[\aa/\aa_3]}.
     The proof concludes by rules~\subexists and \subunpack.
    \end{itemize}
  \end{itemize}
  \item $\typ_1 \equiv \tptr{\loc}$.
  The left rule is \subptr and $\typ_2 \equiv \tptr{\loc}$.
  Similarly, the right rule is \subptr and $\typ_3 \equiv \tptr{\loc}$.
  The proof concludes by rule \subptr.
  \item $\typ_1 \equiv \uninit{n}$.
  As before, $\typ_2 \equiv \typ_3 \equiv \uninit{n}$
  and the proof concludes by rule \submem.
  \item $\typ_1 \equiv \tbor{\lft}{\shr}{\typ'_1}$.
  The left rule is \subborshr and $\typ_2 \equiv \tbor{\lft}{\shr}{\typ'_2}$.
  By inversion, (1) \subtyping{\typ'_1}{\typ'_2}.
  The right rule is \subborshr and $\typ_3 \equiv \tbor{\lft}{\shr}{\typ'_3}$.
  By inversion, (2) \subtyping{\typ'_2}{\typ'_3}.
  By inductive hypothesis on (1) and (2):  \subtyping{\typ'_1}{\typ'_3},
  which concludes the proof by rule \subborshr.

  \item $\typ_1 \equiv \tbor{\lft}{\mut}{\typ'_1}$.
  The left rule is \subbormut and $\typ_2 \equiv \tbor{\lft}{\mut}{\typ'_2}$.
  By inversion, (1) \subtyping{\typ'_1}{\typ'_2} and (2) \subtyping{\typ'_2}{\typ'_1}.
  The right rule is \subbormut and $\typ_3 \equiv \tbor{\lft}{\mut}{\typ'_3}$.
  By inversion, (3) \subtyping{\typ'_2}{\typ'_3} and (4) \subtyping{\typ'_3}{\typ'_2}.
  By inductive hypothesis on (1) and (3): (5) \subtyping{\typ'_1}{\typ'_3}.
  By inductive hypothesis on (4) and (2): (6) \subtyping{\typ'_3}{\typ'_1}.
  The proof concludes by (5), (6), and rule \subbormut.

  \item $\typ_1 \equiv \polysig{\overline{\tvar}}
  {\overline{\aa: \sort}}
  {\expr_1}
  {\loccx_{1i}}
  {\overline{\typ_1}}
  {\typ_{1o}}
  {\loccx_{1o}}$.
  Then,
  $\typ_2 \equiv \polysig{\overline{\tvar}}
  {\overline{\aa: \sort}}
  {\expr_2}
  {\loccx_{2i}}
  {\overline{\typ_2}}
  {\typ_{2o}}
  {\loccx_{2o}}$
  and $ \typ_3 \equiv
  \polysig{\overline{\tvar}}
            {\overline{\aa: \sort}}
            {\expr_3}
            {\loccx_{3i}}
            {\overline{\typ_3}}
            {\typ_{3o}}
            {\loccx_{3o}}$.
By inversion of the two rules:
(1) \entailment{\varcx, \overline{\aa: \sort}}{\expr_2 \Rightarrow \expr_1},
(2) \loccxinc
    {\varcx, \overline{\aa: \sort}}
    {\elftcx}{\llftcx}
    {\loccx_{2i}}
    {\loccx_{1i}},
(3) $\forall i. \subtyping[\varcx, \overline{\aa: \sort}]{\typ_{2i}}{\typ_{1i}}$
(4) \loccxinc
{\varcx, \overline{\aa: \sort}}
{\elftcx}{\llftcx}
{\loccx_{1o}}
{\loccx_{2o}},
(5) \subtyping[\varcx, \overline{\aa: \sort}]{\typ_{1o}}{\typ_{2o}},
(6) \entailment{\varcx, \overline{\aa: \sort}}{\expr_3 \Rightarrow \expr_2},
(7) \loccxinc
    {\varcx, \overline{\aa: \sort}}
    {\elftcx}{\llftcx}
    {\loccx_{3i}}
    {\loccx_{2i}},
(8) $\forall i. \subtyping[\varcx, \overline{\aa: \sort}]{\typ_{3i}}{\typ_{2i}}$
(9) \loccxinc
{\varcx, \overline{\aa: \sort}}
{\elftcx}{\llftcx}
{\loccx_{2o}}
{\loccx_{3o}}, and
(10) \subtyping[\varcx, \overline{\aa: \sort}]{\typ_{2o}}{\typ_{3o}}.

By (1), (5), and assumption~\ref{assumption:model:transitive:implication}:
(11) \entailment{\varcx, \overline{\aa: \sort}}{\expr_3 \Rightarrow \expr_1}.
By (2), (6), and rule \loccxinctrans:
(12) \loccxinc
    {\varcx, \overline{\aa: \sort}}
    {\elftcx}{\llftcx}
    {\loccx_{3i}}
    {\loccx_{1i}}.
By (3), (8), and inductive hypothesis:
(13) $\forall i. \subtyping[\varcx, \overline{\aa: \sort}]{\typ_{3i}}{\typ_{1i}}$.
By (4), (9), and rule \loccxinctrans:
(14) \loccxinc
{\varcx, \overline{\aa: \sort}}
{\elftcx}{\llftcx}
{\loccx_{1o}}
{\loccx_{3o}}.
By (5), (10), and inductive hypothesis:
(15) \subtyping[\varcx, \overline{\aa: \sort}]{\typ_{1o}}{\typ_{3o}}.
The proof concludes by (11)-(15) and rule \subfun.
\end{itemize}
\end{proof}

\begin{lemma}[Weakening]\label{lemma:weakening}
  If \typing{\varcx}
       {\env}
       {\loccx_i}
       {\dynenv}
       {\ee}
       {\typ}
       {\loccx_o}
       {}, \wf{\dynenv'}, and $\dynenv' \supseteq \dynenv$ then
\typing{\varcx}
       {\env}
       {\loccx_i}
       {\dynenv'}
       {\ee}
       {\typ}
       {\loccx_o}
       {}
\end{lemma}
\begin{proof}
 By induction on the expression typing derivation trees.
 \dynenv is only used in the rules \tcall to ensure well-formedness, which is established by assumption,
 and \ttptr, where the theorem holds because $\dynenv' \supseteq \dynenv$.
\end{proof}

\begin{lemma}[Context Inclusion]\label{lemma:conctext-inclusion}
If \loccxinc{\varcx}{}{}{\loccx_2}{\loccx_1} and \typing{\varcx}{\env}{\loccx_1}{\dynenv}{\ee}{\typ}{\loccx_{1o}}{\dynenv},
then \typing{\varcx}{\env}{\loccx_2}{\dynenv}{\ee}{\typ}{\loccx_{2o}}{\dynenv}
and \loccxinc{\varcx}{}{}{\loccx_{2o}}{\loccx_{1o}}.
\end{lemma}
\begin{proof}
  By induction on the derivation trees.
  \newline
  %%% EXPRESSIONS
    \begin{itemize}
        \item \textbf{Rule \tsub:}
        \typing{\varcx}{\env}{\loccx_1}{\dynenv}{\ee}
                {\typ}
                {\loccx_{1o}}
                {\dynenv}.
        By inversion:
        (1) \typing{\varcx}{\env}{\loccx_1}{\dynenv}{\ee}
        {\typ_1}
        {\loccx}
        {\dynenv},
        (2) \subtyping{\typ_1}{\typ}, and
        (3) \loccxinc{\varcx}{\elftcx}{\llftcx}{\loccx}{\loccx_{1o}}.
        By inductive hypothesis on (1):
        (4) \typing{\varcx}{\env}{\loccx_2}{\dynenv}{\ee}
        {\typ_1}
        {\loccx_{2o}}
        {\dynenv} and
        (5) \loccxinc{\varcx}{}{}{\loccx_{2o}}{\loccx}.
        By (2), (4), and rule \tsub,
        \typing{\varcx}{\env}{\loccx_2}{\dynenv}{\ee}
        {\typ}
        {\loccx_{2o}}
        {\dynenv}.
        By (3), (5), and rule~\loccxinctrans,
        (5) \loccxinc{\varcx}{}{}{\loccx_{2o}}{\loccx_{1o}}.

        \item \textbf{Rule \tlet:}
        \typing{\varcx}{\env}{\loccx_{1i}}{\dynenv}{\blet{\xx}{\ee_{\xx}}{\ee}}{\typ}{\loccx_{1o}}{\dynenv_o}.
        By inversion:
        (1) \typing{\varcx}{\env}{\loccx_{1i}}{\dynenv}{\ee_{\xx}}{\typ_{\xx}}{\loccx}{\dynenv},
        (2) \typing{\varcx}{\env,\mapstoenv{\xx}{\typ_\xx}}{\loccx}{\dynenv}{\ee}{\typ}{\loccx_{1o}}{\dynenv_o}, and
        (3) $\xx \not \in \dom{\env}$.
        By inductive hypothesis on (1):
        (4) \typing{\varcx}{\env}{\loccx_{2i}}{\dynenv}{\ee_{\xx}}{\typ_{\xx}}{\loccx'_2}{\dynenv}
        and (5) \loccxinc{\varcx}{}{}{\loccx'_2}{\loccx}.
        By inductive hypothesis on (2), with (5):
        (6) \typing{\varcx}{\env,\mapstoenv{\xx}{\typ_\xx}}{\loccx'_2}{\dynenv}{\ee}{\typ}{\loccx_{2o}}{\dynenv_o}, and
         (5) \loccxinc{\varcx}{}{}{\loccx_{2o}}{\loccx_{1o}}.
         The proof concludes by (5) and rule \tlet on (4), (6), and (3).

        \item \textbf{Rule \tnew:}
        \typing{\varcx}
            {\env}{\loccx_{1i}}{\dynenv}{\blet{\xx}{\new{\lvar}}{e}}{\typ}{\loccx_{1o}}{\dynenv}.
        By inversion:
        (1) \typing{\varcx, \lvar:\sloc}
        {\env, \mapstoenv{\xx}{\tptr{\lvar}}}
        {\loccx_{1i}, \mapstoowned{\lvar}{\uninit{1}}}
        {\dynenv}{\ee}{\typ}{\loccx_{1o}}{\dynenv},
        (2) \wf{\typ},
        (3) \wf{\loccx_{1o}},
        (4) $\xx \notin \dom{\env}$,
        (5) $\lvar \notin \dom{\varcx}$.
        By lemma~\ref{lemma:contextinclusion:endend} and inductive hypothesis on (1):
        (6) \typing{\varcx, \lvar:\sloc}
        {\env, \mapstoenv{\xx}{\tptr{\lvar}}}
        {\loccx_{2i}, \mapstoowned{\lvar}{\uninit{1}}}
        {\dynenv}{\ee}{\typ}{\loccx_{2o}}{\dynenv} and
        (7) \loccxinc{\varcx}{}{}{\loccx_{2o}}{\loccx_{1o}}.
        The proof concludes by (7) and rule \tnew on
        (6), (3), (4), (5), and lemma~\ref{lemma:wf}.

        \item \textbf{Rule \tif:}
        The proofs go by induction and transitive of context inclusion (as in the \tlet case).

        \item \textbf{Rule \tunpack:}
        The proof goes by induction and lemma~\ref{lemma:wf}.

        \item \textbf{Rule \tcall:}
        \typing{\varcx}{\env}{\loccx}{\dynenv}
               {\fcall{\ee}{\overline{\typ}}{\overline{\expr}}{\overline{\aval}}}
               {\applysubst{\substvar}{\typ_o}}{\applysubst{\substvar}{\loccx_{o}}, \loccx_2}{}.
        By inversion:
        (1) $\forall i. \typing{\varcx}{\env}{\loccx}{\dynenv}{\aval_i}{\applysubst{\substvar}{\typ_{i}}}{\loccx}{}$,
        (2) \typing{\varcx}{\env}{\loccx}{\dynenv}{e}
               {\polysig{\overline{\tvar}}
                        {\overline{\aa: \sort}}
                        {\expr}
                        {\loccx_{i}}
                        {\overline{\typ}}
                        {\typ_o}
                        {\loccx_{o}}}
              {\loccx_1, \loccx_2 }{\dynenv},
        (3) $ \substvar = \subst{\overline{\aa}}{\overline{\expr}}$,
        (4) \loccxinc{\varcx}{}{}{\loccx_1}{\applysubst{\substvar}{\loccx_{i}}},
        (5) $\forall i.\sortck{\expr_i}{\sort_i}$,
        (6) \lmodel{\varcx}{\applysubst{\substvar}{\expr}}, and
        (7) \wf{\dynenv}.
       Assume $\loccx'$, so that,
       (8) \loccxinc{\varcx}{}{}{\loccx'}{\loccx}.
       By inductive hypothesis on (1) ans (2):
       (9) $\forall i. \typing{\varcx}{\env}{\loccx'}{\dynenv}{\aval_i}{\applysubst{\substvar}{\typ_{i}}}{\loccx'}{}$,
       (10) \typing{\varcx}{\env}{\loccx'}{\dynenv}{e}
              {\polysig{\overline{\tvar}}
                       {\overline{\aa: \sort}}
                       {\expr}
                       {\loccx_{i}}
                       {\overline{\typ}}
                       {\typ_o}
                       {\loccx_{o}}}
             {\loccx'_{12} }{\dynenv},
        (11) \loccxinc{\varcx}{}{}{\loccx'_{12}}{\loccx_1, \loccx_2}.
        Because of (11), $\dom{\loccx_1, \loccx_2}\subseteq \dom{\loccx'_{12}}$.
        We split $\loccx'_{12}$ to $\loccx'_{12} \equiv \loccx'_1, \loccx'_2$,
        so that $\dom{\loccx_2} = \dom{\loccx'_2}$.
        Then,
        (12) \loccxinc{\varcx}{}{}{\loccx'_1}{\loccx_1} and
        (13) \loccxinc{\varcx}{}{}{\loccx'_2}{\loccx_2}.
        By (9), (10), (3), (5), (6), (7), and rule \loccxinctrans on (4) and (12),
        from rule \tcall we get:
        \typing{\varcx}{\env}{\loccx'}{\dynenv}
        {\fcall{\ee}{\overline{\typ}}{\overline{\expr}}{\overline{\aval}}}
        {\applysubst{\substvar}{\typ_o}}{\applysubst{\substvar}{\loccx_{o}}, \loccx'_2}{}.
        The proof concludes by \loccxincframe and (13).

        \item \textbf{Rule \ttvar, \ttrue, \tfalse, \tconstint, \tfun, \ttptr, and \tumem:}
        In these cases the context is not used and not changed, thus
        $\loccx_{2o} = \loccx_2$,
        $\loccx_{1o} = \loccx_1$, and by assumption:   \loccxinc{\varcx}{}{}{\loccx_{2o}}{\loccx_{1o}}.

        \item \textbf{Rule \tassign:}
        By inversion, inductive hypothesis and application of the rule.

        \item \textbf{Rule \tassignstrg:}
        By inversion, inductive hypothesis, application of the rule and lemma~\ref{lemma:contextinclusion:endend}.

        \item \textbf{Rule \tstrgmutrebor:}
        \rvaltyping{\varcx}{\env}{\loccx_1}{\dynenv}{\rvmutref{\place}}{\tref{\mut}{\typ}}{\loccx_1[\loc\mapsto \typ]}.
        By inversion:
        (1) \pltyping{\varcx}{\env}{\loccx_1}{\dynenv}{\place}{\tptr{\loc}}{\loccx_1} and
        (2) \subtyping{\loccx_1(\loc)}{\typ}.
        By case splitting on the two typing rules for (1):% \nv{note it is complicated that it has to return the same context....}
        (3) \pltyping{\varcx}{\env}{\loccx_2}{\dynenv}{\place}{\tptr{\loc}}{\loccx_2}.
        By assumption, (2), and lemma~\ref{lemma:inclusion:sub}:
        (5) \subtyping{\loccx_2(\loc)}{\typ}.
        By (3), (5), and rule \tstrgmutrebor:
        \rvaltyping{\varcx}{\env}{\loccx_2}{\dynenv}{\rvmutref{\place}}{\tref{\mut}{\typ}}{\loccx_2[\loc\mapsto \typ]}.
        By rules \loccxinctrans, \loccxincperm, and \loccxincframe,
        \loccxinc{\varcx}{}{}{\loccx_2[\loc\mapsto \typ]}{\loccx_1[\loc\mapsto \typ]}, which concludes the proof.

        \item \textbf{Rule \tstrgrebor, \tmutmutrebor, \tshrrebor, \tderef and \tderefstrg:}
        By inductive hypothesis and the fact that in these cases the context is not used and not changed, thus
        $\loccx_{2o} = \loccx_2$,
        $\loccx_{1o} = \loccx_1$, and by assumption:   \loccxinc{\varcx}{}{}{\loccx_{2o}}{\loccx_{1o}}.
  \end{itemize}

\end{proof}

\begin{lemma}[Context Inclusion Extend]\label{lemma:contextinclusion:endend}
  If \loccxinc{\varcx}{}{}{\loccx_2}{\loccx_1},
  then
  \loccxinc{\varcx}{}{}{\loccx_2[\loc\mapsto \typ]}{\loccx_1[\loc\mapsto \typ]}
  and
  \loccxinc{\varcx}{}{}{\loccx_2,\loc\mapsto \typ}{\loccx_1,\loc\mapsto \typ}.
\end{lemma}
\begin{proof}
  By rules \loccxincperm, \loccxincframe, and \loccxinctrans.
\end{proof}

\begin{lemma}[Framing]\label{lemma:framing}
  If {\wf{\loccx_{o1}, \loccx, \loccx_{o2}}}
  and \typing{\varcx}{\env}{\loccx_{i1}, \loccx_{i2}}{\dynenv}{\ee}{\typ}{\loccx_{o1}, \loccx_{o2}}{\dynenv},
then \typing{\varcx}{\env}{\loccx_{i1}, \loccx, \loccx_{i2}}{\dynenv}{\ee}{\typ}{\loccx_{o1}, \loccx, \loccx_{o2}}{\dynenv}.
\end{lemma}
\begin{proof}
  By induction on the derivation tree.
  \newline
  %%% EXPRESSIONS
    \begin{itemize}
        \item \textbf{Rule \tsub:}
        \typing{\varcx}{\env}{\loccx_{i1}, \loccx_{i2}}{\dynenv}{\ee}{\typ}{\loccx_{o1}, \loccx_{o2}}{\dynenv}.
        By inversion:
        (1) \typing{\varcx}{\env}{\loccx_{i1}, \loccx_{i2}}{\dynenv}{\ee}
                {\typ_1}
                {\loccx_1, \loccx_2}
                {\dynenv},
        (2) \subtyping{\typ_1}{\typ}, and
        (3) \loccxinc{\varcx}{\elftcx}{\llftcx}{\loccx_1, \loccx_2}{\loccx_{o1}, \loccx_{o2}}.
        By inductive hypothesis on (1):
        (4) \typing{\varcx}{\env}{\loccx_{i1}, \loccx, \loccx_{i2}}{\dynenv}{\ee}
                {\typ_1}
                {\loccx_1, \loccx, \loccx_2}
                {\dynenv}.
        By lemma~\ref{lemma:framing:context} on (3):
        (5) \loccxinc{\varcx}{\elftcx}{\llftcx}{\loccx_1, \loccx, \loccx_2}{\loccx_{o1}, \loccx, \loccx_{o2}}.
        The proof concludes by (4), (2), (5), and rule \tsub.

        \item \textbf{Rule \tlet:}
        \typing{\varcx}{\env}{\loccx_{i1}, \loccx_{i2}}{\dynenv}{\blet{\xx}{\ee_{\xx}}{\ee}}{\typ}{\loccx_{o1}, \loccx_{o2}}{\dynenv_o}.
        By inversion:
        (1) \typing{\varcx}{\env}{\loccx_{i1}, \loccx_{i2}}{\dynenv}{\ee_{\xx}}{\typ_{\xx}}{\loccx_1, \loccx_2}{\dynenv},
        (2) \typing{\varcx}{\env,\mapstoenv{\xx}{\typ_\xx}}{\loccx_1, \loccx_2}{\dynenv}{\ee}{\typ}{\loccx_{o1}, \loccx_{o2}}{\dynenv_o}, and
        (3) $\xx \not \in \dom{\env}$.
        By inductive hypothesis on (1) and (2):
        (4) \typing{\varcx}{\env}{\loccx_{i1}, \loccx, \loccx_{i2}}{\dynenv}{\ee_{\xx}}{\typ_{\xx}}{\loccx_1, \loccx, \loccx_2}{\dynenv} and
        (5) \typing{\varcx}{\env,\mapstoenv{\xx}{\typ_\xx}}{\loccx_1, \loccx, \loccx_2}{\dynenv}{\ee}{\typ}{\loccx_{o1}, \loccx, \loccx_{o2}}{\dynenv_o}.
        The proof concludes by (3)-(5) and rule \tlet.

        \item \textbf{Rule \tnew:}
        \typing{\varcx}{\env}{\loccx_{i1}, \loccx_{i2}}{\dynenv}{\blet{\xx}{\new{\lvar}}{e}}{\typ}{\loccx_{o1}, \loccx_{o2}}{\dynenv}.
        By inversion:
        (1) \typing{\varcx, \lvar:\sloc}
            {\env, \mapstoenv{\xx}{\tptr{\lvar}}}
            {\loccx_{i1}, \loccx_{i2}, \mapstoowned{\lvar}{\uninit{1}}}
            {\dynenv}{\ee}{\typ}{\loccx_{o1}, \loccx_{o2}}{\dynenv},
        (2) \wf{\typ},
        (3) \wf{\loccx_{o1}, \loccx_{o2}},
        (4) $\xx \notin \dom{\env}$, and
        (5) $\lvar \notin \dom{\varcx}$.
        By inductive hypothesis on (1):
        (6) \typing{\varcx, \lvar:\sloc}
        {\env, \mapstoenv{\xx}{\tptr{\lvar}}}
        {\loccx_{i1}, \loccx, \loccx_{i2}, \mapstoowned{\lvar}{\uninit{1}}}
        {\dynenv}{\ee}{\typ}{\loccx_{o1}, \loccx, \loccx_{o2}}{\dynenv}.
        By assumption: (7) \wf{\loccx_{o1}, \loccx, \loccx_{o2}}.
        The proof concludes by (6), (2), (7), (4), (5), and rule \tnew.
        \item \textbf{Rule \tif:}
        \typing{\varcx}{\env}{\loccx_{i1}, \loccx_{i2}}{\dynenv_i}{\bif{\ee}{\ee_1}{\ee_2}}{\typ}{\loccx_{o1}, \loccx_{o2}}{\dynenv}.
        By inversion:
        (1) \typing{\varcx}{\env}{\loccx_{i1}, \loccx_{i2}}{\dynenv}{\ee}{\rtyp{\tbool}{\expr}}{\loccx_1, \loccx_2}{\dynenv_o},
        (2) \typing{\varcx, \expr}{\env}{\loccx_1, \loccx_2}{\dynenv}{\ee_1}{\typ}{\loccx_{o1}, \loccx_{o2}}{\dynenv}, and
        (3) \typing{\varcx, \lnot \expr}{\env}{\loccx_1, \loccx_2}{\dynenv}{\ee_2}{\typ}{\loccx_{o1}, \loccx_{o2}}{\dynenv}.
        The proof concludes by inductive hypothesis on (1)-(3) and the rule \tif.

        % \item \textbf{Rule \tseq:}
        % By inversion, case~\ref{lemma:framing:stmt} and inductive hypothesis, and application of the rule.

        \item \textbf{Rule \tunpack:}
        By inversion, inductive hypothesis and the well formedness assumption, and application of the rule.

        \item \textbf{Rule \tcall:}
        \typing{\varcx}{\env}{\loccx_{i1}, \loccx_{i2}}{\dynenv}
               {\fcall{\ee}{\overline{\typ}}{\overline{\expr}}{\overline{\aval}}}
               {\applysubst{\substvar}{\typ_o}}{\applysubst{\substvar}{\loccx_{o}}, \loccx_2}{}
        By inversion:
        \begin{enumerate}
        \item $\forall i. \typing{\varcx}{\env}{\loccx_{i1}, \loccx_{i2}}{\dynenv}{\aval_i}{\applysubst{\substvar}{\typ_{i}}}{\loccx_{i1}, \loccx_{i2}}{}$,
        \item \typing{\varcx}{\env}{\loccx_{i1}, \loccx_{i2}}{\dynenv}{e}
               {\polysig{\overline{\tvar}}
                        {\overline{\aa: \sort}}
                        {\expr}
                        {\loccx_{i}}
                        {\overline{\typ}}
                        {\typ_o}
                        {\loccx_{o}}}
              {\loccx_1, \loccx_2 }{\dynenv},
        \item $\substvar = \subst{\overline{\aa}}{\overline{\expr}}$,
        \item \loccxinc{\varcx}{}{}{\loccx_1}{\applysubst{\substvar}{\loccx_{i}}},
        \item $\forall i.\sortck{\expr_i}{\sort_i}$,
        \item \lmodel{\varcx}{\applysubst{\substvar}{\expr}}, and
        \item \wf{\dynenv}.
        \end{enumerate}
%        (8) $\dom{\loccx_{o}} \cap \dom{\loccx_2} = \emptyset$.
        %
        By inductive hypothesis on (1) and (2):
        \begin{enumerate}
          \setcounter{enumi}{7}
          \item $\forall i. \typing{\varcx}{\env}{\loccx_{i1}, \loccx, \loccx_{i2}}{\dynenv}{\aval_i}{\applysubst{\substvar}{\typ_{i}}}{\loccx_{i1}, \loccx, \loccx_{i2}}{}$,
          \item \typing{\varcx}{\env}{\loccx_{i1}, \loccx, \loccx_{i2}}{\dynenv}{e}
                    {\polysig{\overline{\tvar}}
                              {\overline{\aa: \sort}}
                              {\expr}
                              {\loccx_{i}}
                              {\overline{\typ}}
                              {\typ_o}
                              {\loccx_{o}}}
                    {\loccx_1, \loccx, \loccx_2 }{\dynenv}.
        \end{enumerate}
        By (3)-(9) and rule \tcall, we get the following:
        $$
        \typing{\varcx}{\env}{\loccx_{i1}, \loccx, \loccx_{i2}}{\dynenv}
               {\fcall{\ee}{\overline{\typ}}{\overline{\expr}}{\overline{\aval}}}
               {\applysubst{\substvar}{\typ_o}}{\applysubst{\substvar}{\loccx_{o}}, (\loccx, \loccx_2)}{}.
        $$

        \item \textbf{Rule \tfun:} By inversion of the rule:
        $$
        \typing{\varcx,\overline{\aa: \sort},\expr}
               {\env,
                \overline{\xx : \typ},
                \ff: \polysig{\overline{\tvar}}{{\overline{\aa: \sort}}}
                             {{\expr}}{\loccx_{i}}
                             {\overline{\typ}}
                             {{\typ}}
                             {\loccx_{o}}
                }
               {\loccx_{i}}{\dynenv}
               {\ee}
               {\typ}{\loccx_o}
               {}
        $$

        \item \textbf{Rule \ttvar, \ttrue, \tfalse, \tconstint, \tfun, \ttptr, and \tumem:}
        These cases are trivial because typing preserves the location context.
        So, if
        \typing{\varcx}{\env}{\loccx_{i1}, \loccx_{i2}}{\dynenv}{\ee}{\typ}{\loccx_{i1}, \loccx_{i2}}{\dynenv},
        then \typing{\varcx}{\env}{\loccx_{i1}, \loccx, \loccx_{i2}}{\dynenv}{\ee}{\typ}{\loccx_{i1}, \loccx, \loccx_{i2}}{\dynenv}.

        \item \textbf{Rule \tassign:} by inversion, inductive hypothesis
        and application of the rule.

        \item \textbf{Rule \tassignstrg:} by inversion, inductive hypothesis
        and application of the rule.

      \item \textbf{Rule \tstrgrebor:} by inversion, inductive hypothesis, and application of the rule.

      \item \textbf{Rule \tstrgmutrebor:}
      \rvaltyping{\varcx}{\env}{\loccx_{1}, \loccx_{2}}{\dynenv}{\rvmutref{\place}}{\tref{\mut}{\typ}}{(\loccx_{1} , \loccx_{2})[\loc\mapsto \typ]}.
      By inversion:
      (1) \pltyping{\varcx}{\env}{\loccx_{1} , \loccx_{2}}{\dynenv}{\place}{\tptr{\loc}}{\loccx_{1} , \loccx_{2}} and
      (2) \subtyping{(\loccx_{1} , \loccx_{2})(\loc)}{\typ}.
      By inductive hypothesis on (1):
      (3) \pltyping{\varcx}{\env}{\loccx_{1} , \loccx , \loccx_{2}}{\dynenv}{\place}{\tptr{\loc}}{\loccx_{1}, \loccx , \loccx_{2}}.
      By the disjointness assumption  $(\loccx_{1} , \loccx_{2})(\loc) = (\loccx_{1}  , \loccx , \loccx_{2})(\loc)$, thus (2) becomes:
      (4) \subtyping{(\loccx_{1} , \loccx , \loccx_{2})(\loc)}{\typ}.
      The proof concludes by (2), (4), and rule \tstrgmutrebor.
      \item \textbf{Rule \tmutmutrebor, \tshrrebor, \tderef and \tderefstrg:} by inversion, inductive hypothesis, and application of the rule.
      % \item \textbf{Rule \tshrrebor:} by inversion, case~\ref{lemma:framing:expr}, and application of the rule.
      % \item \textbf{Rule \tderef:} by inversion, case~\ref{lemma:framing:expr}, and application of the rule.
      % \item \textbf{Rule \tderefstrg:} by inversion, case~\ref{lemma:framing:expr}, and application of the rule.
      % \item \textbf{Rule \trvalval:} by inversion, case~\ref{lemma:framing:expr}, and application of the rule.
  \end{itemize}
\end{proof}

\begin{lemma}[Context Inclusion Subtyping]\label{lemma:inclusion:sub}
  If \loccxinc{\varcx}{}{}{\loccx_2}{\loccx_1} and \subtyping{\loccx_1(\loc)}{\typ},
  then \subtyping{\loccx_2(\loc)}{\typ}.
\end{lemma}
\begin{proof}
By induction on the context inclusion tree and by splitting cases in the
\loccxincframe rule.
\end{proof}

\begin{lemma}[Inclusion Framing]\label{lemma:framing:context}
  If \loccxinc{\varcx}{\elftcx}{\llftcx}{\loccx_{i1}, \loccx_{i2}}{\loccx_{o1}, \loccx_{o2}},
  then \loccxinc{\varcx}{\elftcx}{\llftcx}{\loccx_{i1}, \loccx, \loccx_{i2}}{\loccx_{o1}, \loccx, \loccx_{o2}}.
\end{lemma}
\begin{proof}
    By assumption:
    $$(1) \loccxinc{\varcx}{\elftcx}{\llftcx}{\loccx_{i1}, \loccx_{i2}}{\loccx_{o1}, \loccx_{o2}}.$$
    By rule \loccxincframe:
    $$(2) \loccxinc{\varcx}{\elftcx}{\llftcx}{\loccx, \loccx_{i1}, \loccx_{i2}}{\loccx, \loccx_{o1}, \loccx_{o2}}.$$
    By rule \loccxincperm:
    $$(3) \loccxinc{\varcx}{\elftcx}{\llftcx}{\loccx_{i1}, \loccx, \loccx_{i2}}{\loccx, \loccx_{i1}, \loccx_{i2}}
    \text{ and }
    (4) \loccxinc{\varcx}{\elftcx}{\llftcx}{\loccx, \loccx_{o1}, \loccx_{o2}}{\loccx_{o1}, \loccx, \loccx_{o2}}.$$
    By (3), (2), and \loccxinctrans:
    $$(5) \loccxinc{\varcx}{\elftcx}{\llftcx}{\loccx_{i1}, \loccx, \loccx_{i2}}{\loccx, \loccx_{o1}, \loccx_{o2}}.$$
    By (5), (4), and \loccxinctrans:
    $$(6) \loccxinc{\varcx}{\elftcx}{\llftcx}{\loccx_{i1}, \loccx, \loccx_{i2}}{\loccx_{o1}, \loccx, \loccx_{o2}}.$$
    Which concludes the proof.
\end{proof}

\begin{lemma}[AVal Typing]\label{lemma:aval}
If \typing{\varcx}{\env}{\loccx_i}{\dynenv}{\aval}{\typ}{\loccx_o}{\dynenv},
then for any $\loccx$, so that \wf{\loccx},
\typing{\varcx}{\env}{\loccx}{\dynenv}{\aval}{\typ}{\loccx}{\dynenv}.
\end{lemma}
\begin{proof}
By exhaustion: the typing rules for \aval
and the type weakening part of rule \tsub, do not depent on \loccx.
\end{proof}

% \begin{lemma}[Well-formedness]\label{lemma:typing-implies-wf}
%   If \typing{\varcx{}}
%        {\env}
%        {\loccx_i}
%        {\dynenv}
%        {\ee}
%        {\typ}
%        {\loccx_o}
%        {}
% then \wf{\env}, \wf{\loccx_i}, \wf{\dynenv}, \wf{\typ} and \wf{\loccx_o}.
% \end{lemma}
% \begin{proof}
%   \todo{This does not hold, check the leaves. But we do not seem to need it.}
% \end{proof}

\begin{lemma}[Well-formed Variables]\label{lemma:wf-fv}
  Well-formedness ensures free variables are included in $\varcx$:
  \begin{itemize}
  \item If \wf{\typ} then $\fv{\typ}\subseteq \dom{\varcx}$.
  \item If \wf{\env} then $\fv{\env}\subseteq \dom{\varcx}$.
  \item If \wf{\loccx} then $\fv{\loccx}\subseteq \dom{\varcx}$.
  \item If \wf{\dynenv} then $\fv{\dynenv}\subseteq \dom{\varcx}$.
\end{itemize}
\end{lemma}
\begin{proof}
By structural induction on the type and the environments.
\end{proof}

\begin{lemma}[Id Substitution]\label{lemma:fv-subst}
When a variable is not free, substitution is identity:
  \begin{itemize}
    \item If $\aa \notin \fv{\typ}$, then $\typ[\expr/\aa]=\typ$.
    \item If $\aa \notin \fv{\env}$, then $\env[\expr/\aa]=\env$.
    \item If $\aa \notin \fv{\loccx}$, then $\loccx[\expr/\aa]=\loccx$.
    \item If $\aa \notin \fv{\dynenv}$, then $\dynenv[\expr/\aa]=\dynenv$.
  \end{itemize}
\end{lemma}
\begin{proof}
  By structural induction on the type and the environments.
\end{proof}

\begin{lemma}[Id Var Substitution]\label{lemma:subst:idvar}
$\typ[\aa/\aa]=\typ$
\end{lemma}
\begin{proof}
  By structural induction on the type.
\end{proof}

\begin{lemma}[Condition]\label{lemma:condition}
  If \lmodel{\varcx_1}{\expr}, then:
  \begin{enumerate}[label=\roman*]
  \item\label{lemma:condition:typing} If \typing{\varcx_1, \expr, \varcx_2}
           {\env}
           {\loccx_i}
           {\dynenv}
           {\ee}
           {\typ}
           {\loccx_o}
           {},
  then
  \typing{\varcx_1, \varcx_2}
           {\env}
           {\loccx_i}
           {\dynenv}
           {\ee}
           {\typ}
           {\loccx_o}
           {}.
  \item\label{lemma:condition:subtyping}
  If \subtyping[\varcx_1, \expr, \varcx_2]{\typ_1}{\typ_2},
  then \subtyping[\varcx_1, \varcx_2]{\typ_1}{\typ_2}.
  \item\label{lemma:condition:context}
  If \loccxinc{\varcx_1, \expr, \varcx_2}{\elftcx}{\llftcx}
           {\loccx_i}
           {\loccx_o},
  then
  \loccxinc{\varcx_1, \varcx_2}{\elftcx}{\llftcx}
           {\loccx_i}
           {\loccx_o}.
  \end{enumerate}
  \end{lemma}
  \begin{proof}
  By mutual induction on the derivation trees.
  \newline
  \textbf{Case \ref{lemma:condition:typing})}
  We split cases on the type derivation.
  \begin{itemize}
    \item \textbf{Rule \tsub:}
    \typing{\varcx_1, \expr, \varcx_2}{\env}{\loccx_i}{\dynenv}{\ee}
    {\typ}
    {\loccx_o}
    {\dynenv}.
    By inversion:
  (1) \typing{\varcx_1, \expr, \varcx_2}{\env}{\loccx_i}{\dynenv}{\ee}
    {\typ_1}
    {\loccx}
    {\dynenv},
  (2) \subtyping[\varcx_1, \expr, \varcx_2]{\typ_1}{\typ}, and
  (3) \loccxinc{\varcx_1, \expr, \varcx_2}{\elftcx}{\llftcx}{\loccx}{\loccx_o}.
  By inductive hypothesis on (1) we get
  (4) \typing{\varcx_1, \varcx_2}{\env}{\loccx_i}{\dynenv}{\ee}
    {\typ_1}
    {\loccx}
    {\dynenv}.
  By (2) and case~\ref{lemma:condition:subtyping}, we get
  (5) \subtyping[\varcx_1, \varcx_2]{\typ_1}{\typ}.
  By (3) and case~\ref{lemma:condition:context}, we get
  (6) \loccxinc{\varcx_1, \varcx_2}{\elftcx}{\llftcx}{\loccx}{\loccx_o}.
  By (4), (5), (6), and rule \tsub, we conclude the proof.
    \item \textbf{Rule \tlet:}
    $\typing{\varcx_1, \expr, \varcx_2}{\env}{\loccx_i}{\dynenv}{\blet{\xx}{\ee_{\xx}}{\ee}}{\typ}{\loccx_o}{\dynenv_o}$.
    By inversion:
    (1) \typing{\varcx_1, \expr, \varcx_2}{\env}{\loccx_i}{\dynenv}{\ee_{\xx}}{\typ_{\xx}}{\loccx}{\dynenv} and
    (2) \typing{\varcx_1, \expr, \varcx_2}{\env,\mapstoenv{\xx}{\typ_\xx}}{\loccx}{\dynenv}{\ee}{\typ}{\loccx_o}{\dynenv_o}.
    By inductive hypothesis:
    (3) \typing{\varcx_1, \varcx_2}{\env}{\loccx_i}{\dynenv}{\ee_{\xx}}{\typ_{\xx}}{\loccx}{\dynenv} and
    (4) \typing{\varcx_1, \varcx_2}{\env,\mapstoenv{\xx}{\typ_\xx}}{\loccx}{\dynenv}{\ee}{\typ}{\loccx_o}{\dynenv_o}.
    By (3), (4), and rule \tlet, we conclude the proof.
    \item \textbf{Rule \tnew:}
    \typing{\varcx_1, \expr, \varcx_2}
              {\env}{\loccx_i}{\dynenv}{\blet{\xx}{\new{\lvar}}{e}}{\typ}{\loccx_o}{\dynenv}.
    By inversion:
    (1) \typing{\varcx_1, \expr, \varcx_2, \lvar:\sloc}
    {\env, \mapstoenv{\xx}{\tptr{\lvar}}}
    {\loccx_i, \mapstoowned{\lvar}{\uninit{1}}}
    {\dynenv}{\ee}{\typ}{\loccx_o}{\dynenv},
    (2) \wf[\varcx_1, \expr, \varcx_2]{\typ}, and
    (3) \wf[\varcx_1, \expr, \varcx_2]{\loccx_o}.
    By inductive hypothesis on (1), and lemma~\ref{lemma:condition:weaken} on (2) and (3):
    (4) \typing{\varcx_1, \varcx_2, \lvar:\sloc}
    {\env, \mapstoenv{\xx}{\tptr{\lvar}}}
    {\loccx_i, \mapstoowned{\lvar}{\uninit{1}}}
    {\dynenv}{\ee}{\typ}{\loccx_o}{\dynenv},
    (5) \wf[\varcx_1, \varcx_2]{\typ}, and
    (6) \wf[\varcx_1, \varcx_2]{\loccx_o}.
    By (4), (5), (6), and rule \tnew, we conclude the proof.
    \item \textbf{Rule \tif:}
    (1) $\typing{\varcx_1, \expr, \varcx_2}{\env}{\loccx_i}{\dynenv_i}{\bif{\ee}{\ee_1}{\ee_2}}{\typ}{\loccx}{\dynenv}$.
    By inversion:
    (2) \typing{\varcx_1, \expr, \varcx_2}{\env}{\loccx_i}{\dynenv}{\ee}{\rtyp{\tbool}{\expr_\ee}}{\loccx_o}{\dynenv_o},
    (3) \typing{\varcx_1, \expr, \varcx_2, \expr_\ee}{\env}{\loccx_o}{\dynenv}{\ee_1}{\typ}{\loccx}{\dynenv}, and
    (4) \typing{\varcx_1, \expr, \varcx_2, \lnot \expr_\ee}{\env}{\loccx_o}{\dynenv}{\ee_2}{\typ}{\loccx}{\dynenv}.
    By inductive hypothesis:
    (5) \typing{\varcx_1, \varcx_2}{\env}{\loccx_i}{\dynenv}{\ee}{\rtyp{\tbool}{\expr_\ee}}{\loccx_o}{\dynenv_o},
    (6) \typing{\varcx_1, \varcx_2, \expr_\ee}{\env}{\loccx_o}{\dynenv}{\ee_1}{\typ}{\loccx}{\dynenv}, and
    (7) \typing{\varcx_1, \varcx_2, \lnot \expr_\ee}{\env}{\loccx_o}{\dynenv}{\ee_2}{\typ}{\loccx}{\dynenv}.
    By (5), (6), (7), and rule \tif we conclude the proof.
    % \item \textbf{Rule \tseq:}
    % (1) \typing{\varcx_1, \expr, \varcx_2}{\env}{\loccx_i}{\dynenv}{\bseq{\stmt}{\rexpr}}{\typ}{\loccx_o}{\dynenv_o}.
    % By inversion:
    % (2) \stmtyping{\varcx_1, \expr, \varcx_2}{\env}{\loccx_i}{\dynenv}{\stmt}{\loccx_{\stmt}}{\dynenv_{\stmt}} and
    % (3) \typing{\varcx_1, \expr, \varcx_2}{\env}{\loccx_{\stmt}}{\dynenv}{\rexpr}{\typ}{\loccx_o}{\dynenv_o}.
    % By case~\ref{lemma:condition:statements} on (2) and inductive hypothesis on (3):
    % (4) \stmtyping{\varcx_1, \varcx_2}{\env}{\loccx_i}{\dynenv}{\stmt}{\loccx_{\stmt}}{\dynenv_{\stmt}} and
    % (5) \typing{\varcx_1, \varcx_2}{\env}{\loccx_{\stmt}}{\dynenv}{\rexpr}{\typ}{\loccx_o}{\dynenv_o}.
    % By (4), (5), and rule \tseq we conclude the proof.
    \item \textbf{Rule \tunpack:}
    (1) \typing{\varcx_1, \expr, \varcx_2}{\env_1,\mapstoenv{\xx}{\texists{\aa}{\rtyp{\tcon}{\aa}}{\expr}}, \env_2}
                 {\loccx_i}{\dynenv}
                 {\eunpack{\xx}{\aa}{e}}{\typ}
                 {\loccx_o}{\dynenv}.
    By inversion:
    (2) \typing{\varcx_1, \expr, \varcx_2, \aa : \getsort{\tcon}, \expr}{\env_1,\mapstoenv{\xx}{\rtyp{\tcon}{\aa}}, \env_2}
                 {\loccx_i}{\dynenv}
                 {\ee}{\typ}
                 {\loccx_o}{\dynenv}.
    By inductive hypothesis:
    (2) \typing{\varcx_1, \varcx_2, \aa : \getsort{\tcon}, \expr}{\env_1,\mapstoenv{\xx}{\rtyp{\tcon}{\aa}}, \env_2}
                 {\loccx_i}{\dynenv}
                 {\ee}{\typ}
                 {\loccx_o}{\dynenv}.
    Which concludes the proof by rule \tunpack.
    \item \textbf{Rule \tcall:}
    (1)         \typing{\varcx_1, \expr, \varcx_2}{\env}{\loccx}{\dynenv}
    {\fcall{e}{\overline{\typ}}{\overline{\expr}}{\overline{\aval}}}
    {\applysubst{\substvar}{\typ_o}}{\applysubst{\substvar}{\loccx_{o}}, \loccx_2}{}.
    By inversion, for $\substvar = \subst{\overline{\aa}}{\overline{\expr}}$:
    (2) $ \forall i. \typing{\varcx_1, \expr, \varcx_2}{\env}{\loccx}{\dynenv}{\aval_i}{\applysubst{\substvar}{\typ_{i}}}{\loccx}{}$,
    (3) $\typing{\varcx_1, \expr, \varcx_2}{\env}{\loccx}{\dynenv}{e}
           {\polysig{\overline{\tvar}}
                    {\overline{\aa: \sort}}
                    {\expr}
                    {\loccx_{i}}
                    {\overline{\typ}}
                    {\typ_o}
                    {\loccx_{o}}}
          {\loccx_1, \loccx_2 }{\dynenv}$,
    (4) \loccxinc{\varcx_1, \expr, \varcx_2}{}{}{\loccx_1}{\applysubst{\substvar}{\loccx_{i}}},
    (5) $ \forall i.\sortck[\varcx_1, \expr, \varcx_2]{\expr_i}{\sort_i}$,
    (6) \lmodel{\varcx_1, \expr, \varcx_2}{\applysubst{\substvar}{\expr}}, and
    (7) \wf[\varcx_1, \expr, \varcx_2]{\dynenv}.
    By inductive hypothesis on (2) and (3),
    case~\ref{lemma:condition:context} on (4),
    assumption~\ref{assumption:model:cut} on (6), and
    lemma~\ref{lemma:condition:weaken} on (5) and (7):
    (8) $ \forall i. \typing{\varcx_1,  \varcx_2}{\env}{\loccx}{\dynenv}{\aval_i}{\applysubst{\substvar}{\typ_{i}}}{\loccx}{}$,
    (9) $\typing{\varcx_1,  \varcx_2}{\env}{\loccx}{\dynenv}{e}
           {\polysig{\overline{\tvar}}
                    {\overline{\aa: \sort}}
                    {\expr}
                    {\loccx_{i}}
                    {\overline{\typ}}
                    {\typ_o}
                    {\loccx_{o}}}
          {\loccx_1, \loccx_2 }{\dynenv}$,
    (10) \loccxinc{\varcx_1,  \varcx_2}{}{}{\loccx_1}{\applysubst{\substvar}{\loccx_{i}}},
    (11) $ \forall i.\sortck[\varcx_1,  \varcx_2]{\expr_i}{\sort_i}$,
    (12) \lmodel{\varcx_1,  \varcx_2}{\applysubst{\substvar}{\expr}}, and
    (13) \wf[\varcx_1,  \varcx_2]{\dynenv}.
    BY (8)-(13) and rule \tcall we conclude the proof.
    \item \textbf{Rule \tfun:}
    (1) \typing{\varcx_1, \expr, \varcx_2}{\env}{\loccx}{\dynenv}
                 {\vrec{\ff}{\overline{\aa}}{\overline{\xx}}{{e}}}
                 {\polysig{\overline{\tvar}}{{\overline{\aa: \sort}}}
                            {\expr}{\loccx_{i}}{\overline{\typ}}
                            {\typ}{\loccx_{o}}
                 }
                 {\loccx}{\dynenv}.
    By inversion:
    (2) \typing{\varcx_1, \expr, \varcx_2,\overline{\aa: \sort},\expr}
                 {\env,
                  \overline{\xx : \typ},
                  \ff: \polysig{\overline{\tvar}}{{\overline{\aa: \sort}}}
                               {{\expr}}{\loccx_{i}}
                               {\overline{\typ}}
                               {{\typ}}
                               {\loccx_{o}}
                  }
                 {\loccx_i}{\dynenv}
                 {\ee}
                 {\typ}{\loccx_o}
                 {}.
    By inductive hypothesis:
    (3) \typing{\varcx_1, \varcx_2,\overline{\aa: \sort},\expr}
                 {\env,
                  \overline{\xx : \typ},
                  \ff: \polysig{\overline{\tvar}}{{\overline{\aa: \sort}}}
                               {{\expr}}{\loccx_{i}}
                               {\overline{\typ}}
                               {{\typ}}
                               {\loccx_{o}}
                  }
                 {\loccx_i}{\dynenv}
                 {\ee}
                 {\typ}{\loccx_o}
                 {}.
     (3) and rule \tfun concludes the proof.
    \item \textbf{Rules \ttvar, \ttrue, \tfalse, \tconstint, \ttptr, and \tumem:}
    are trivial since they do not depend on the logical environment.

    % \item \textbf{Rule \tskip:}
    % \stmtyping{\varcx_1, \expr, \varcx_2}{\env}{\loccx}{\dynenv}{\sskip}{\loccx}{\dynenv}.
    % By rule \tskip,
    % \stmtyping{\varcx_1, \varcx_2}{\env}{\loccx}{\dynenv}{\sskip}{\loccx}{\dynenv},
    % which concludes the proof.

    \item \textbf{Rule \tassign:}
    (1) \typing{\varcx_1, \expr, \varcx_2}{\env}{\loccx_i}{\dynenv}{\sassign{\place}{\ee}}{\uninit{1}}{\loccx_o}{}.
    By inversion:
    (2) \rvaltyping{\varcx_1, \expr, \varcx_2}{\env}{\loccx_i}{\dynenv}{\ee'}{\typ_v}{\loccx_i},
    (3) \pltyping{\varcx_1, \expr, \varcx_2}{\env}{\loccx_i}{\dynenv}{\place}{\tref{\mut}{\typ}}{\loccx_i}, and
    (4) \subtyping[\varcx_1, \expr, \varcx_2]{\typ_v}{\typ}.
    By inductive hypothesis on (2) and case~\ref{lemma:condition:subtyping} on (4):
    (5) \rvaltyping{\varcx_1, \varcx_2}{\env}{\loccx_i}{\dynenv}{\ee'}{\typ_v}{\loccx_i},
    (6) \subtyping[\varcx_1, \varcx_2]{\typ_v}{\typ}.
    By (5), (3), (6), and rule \tassign, we conclude the proof.

    \item \textbf{Rule \tassignstrg:}
    (1) \stmtyping{\varcx_1, \expr, \varcx_2}{\env}{\loccx_i}{\dynenv}{\sassign{\place}{\ee'}}{\loccx_o[\loc \mapsto \typ]}{}.
    By inversion:
    (2) \rvaltyping{\varcx_1, \expr, \varcx_2}{\env}{\loccx_i}{\dynenv}{\ee'}{\typ}{\loccx_o} and
    (3) \pltyping{\varcx_1, \expr, \varcx_2}{\env}{\loccx_i}{\place}{\tptr{\loc}}{\loccx_i}.
    By inductive hypothesis on (2):
    (4) \rvaltyping{\varcx_1, \varcx_2}{\env}{\loccx_i}{\dynenv}{\ee'}{\typ}{\loccx_o}.
    By (4), (3), and rule \tassignstrg we conclude the proof.

    \item \textbf{Rule \tstrgmutrebor and \tshrrebor:}
    By inversion, application of case~\ref{lemma:condition:subtyping},
    and application of the respective rule.

    \item \textbf{Rule \tstrgrebor, \tmutmutrebor, \tderef, and \tderefstrg:}
    These cases are trivial since they do not depend on the logical environment.
  \end{itemize}

  \textbf{Case \ref{lemma:condition:subtyping})} We split cases on the subtyping derivation:
  \begin{itemize}
    \item \textbf{Rule \tstrgrebor:}
    \subtyping[\varcx_1, \expr, \varcx_2, \aa: \getsort{\tcon}, \expr_\aa]
    {\rtyp{\tcon}{\aa}}
    By inductive hypothesis:
    (3) \subtyping
    [\varcx_1, \varcx_2, \aa: \getsort{\tcon}, \expr_\aa]
    {\rtyp{\tcon}{\aa}}
    {\typ}.
    (3) and rule \subunpack conclude the proof.
    \item \textbf{Rule \subexists:}
    (1) \subtyping[\varcx_1, \expr, \varcx_2]
                  {\rtyp{\tcon}{\expr_1}}
                  {\texists{\aa}{\rtyp{\tcon}{\aa}}{\expr_2}}.
    By inversion:
    (2) \entailment{\varcx_1, \expr, \varcx_2}{\expr_2[\expr_1/\aa]}.
    By hypothesis, (2), and assumption~\ref{assumption:model:cut}:
    (3) \entailment{\varcx_1, \varcx_2}{\expr_2[\expr_1/\aa]}.
    (3) and rule \subexists conclude the proof.
    \item \textbf{Rule \subborshr:}
    \subtyping[\varcx_1, \expr, \varcx_2]
    {\tbor{\lft}{\shr}{\typ_1}}
    {\tbor{\lft}{\shr}{\typ_2}}.
    By inversion:
    \subtyping[\varcx_1, \expr, \varcx_2]{\typ_1}{\typ_2}.
    By inductive hypothesis:
    \subtyping[\varcx_1, \varcx_2]{\typ_1}{\typ_2},
    which, by rule \subborshr concludes the proof.
    \item \textbf{Rule \subbormut:}
    \subtyping[\varcx_1, \expr, \varcx_2]
    {\tbor{\lft}{\mut}{\typ_1}}
    {\tbor{\lft}{\mut}{\typ_2}}.
    By inversion:
    \subtyping[\varcx_1, \expr, \varcx_2]{\typ_1}{\typ_2} and
    \subtyping[\varcx_1, \expr, \varcx_2]{\typ_2}{\typ_1}.
    By inductive hypothesis:
    \subtyping[\varcx_1, \varcx_2]{\typ_1}{\typ_2} and
    \subtyping[\varcx_1, \varcx_2]{\typ_2}{\typ_1},
    which, by rule \subbormut concludes the proof.
  \end{itemize}

  \textbf{Case \ref{lemma:condition:context})}
  We split cases on the context derivation:
  \begin{itemize}
    \item \textbf{Rule \loccxincperm:}
    \loccxinc
    {\varcx_1, \expr, \varcx_2}
    {\elftcx}{\llftcx}
    {\loccx}
    {\loccx'}.
    By inversion $\loccx'$  is a permutation of  $\loccx$.
    By rule \loccxincperm,
    \loccxinc
    {\varcx_1, \varcx_2}
    {\elftcx}{\llftcx}
    {\loccx}
    {\loccx'}, which concludes the proof.
    \item \textbf{Rule \loccxincweaken:}
    \loccxinc{\varcx_1, \expr, \varcx_2}
                  {\elftcx}{\llftcx}
                  {\loccx,\loccx'}
                  {\loccx}.
    By rule \loccxincweaken:
    \loccxinc{\varcx_1, \varcx_2}
    {\elftcx}{\llftcx}
    {\loccx,\loccx'}
    {\loccx}, which concludes the proof.
    \item \textbf{Rule \loccxincframe:}
    \loccxinc
    {\varcx_1, \expr, \varcx_2}
    {\elftcx}{\llftcx}
    {\loccx,\loccx_1}
    {\loccx, \loccx_2}.
    By inversion:
    \loccxinc{\varcx_1, \expr, \varcx_2}
             {\elftcx}{\llftcx}
             {\loccx_1}{\loccx_2}.
    By inductive hypothesis:
    \loccxinc{\varcx_1, \varcx_2}
             {\elftcx}{\llftcx}
             {\loccx_1}{\loccx_2}.
    By which and rule \loccxincframe we conclude the proof.
    \item \textbf{Rule \loccxincsub:}
    \loccxinc{\varcx_1, \expr, \varcx_2}
                  {\elftcx}{\llftcx}
                  {\mapstoowned{\loc}{\typ_1}}
                  {\mapstoowned{\loc}{\typ_2}}.
    By inversion: \subtyping[\varcx_1, \expr, \varcx_2]{\typ_1}{\typ_2}.
    By case~\ref{lemma:condition:subtyping},
    By inversion: \subtyping[\varcx_1, \varcx_2]{\typ_1}{\typ_2}.
    Which concludes the proof by rule \loccxincsub.
  \end{itemize}
  \end{proof}

  \begin{lemma}[Condition Weakening]\label{lemma:condition:weaken}.
    \begin{enumerate}
    \item\label{lemma:condition:wftyp}
    If \wf[\varcx_1, \expr, \varcx_2]{\typ}, then \wf[\varcx_1, \varcx_2]{\typ}.
    \item\label{lemma:condition:context:wft}
    If \wf[\varcx_1, \expr, \varcx_2]{\loccx}, then \wf[\varcx_1, \varcx_2]{\loccx}.
    \item\label{lemma:condition:context:sort}
    If \sortck[\varcx_1, \expr, \varcx_2]{\expr}{\sort}, \sortck[\varcx_1, \varcx_2]{\expr}{\sort}.
    \end{enumerate}
  \end{lemma}
  \begin{proof}
  By mutual induction on the derivation trees.
  Note that all three derivations depend on the bindings and not
  the expressions of the logical environment.
  \end{proof}

\begin{lemma}[Substitution]\label{lemma:program-substitution}\label{lemma:program-substitution-2}
  If  \typing{\varcx}{\env_1}{\loccx_i}{\dynenv}{\val}{\typ_x}{\loccx_i}{}, then
  If \typing{\varcx}
         {\env_1,\mapstoenv{\xx}{\typ_x},\env_2}
         {\loccx_i}
         {\dynenv}
         {\ee}
         {\typ}
         {\loccx_o}
         {},
  then
  \typing{\varcx}
         {\env_1,\env_2}
         {\loccx_i}
         {\dynenv}
         {\ee[\val/\xx]}
         {\typ}
         {\loccx_o}
         {}.
  \end{lemma}
  \begin{proof}
    By induction on the derivation tree.
\begin{itemize}
\item \textbf{Rule \tsub:}
(1) \typing{\varcx}{\env_1,\mapstoenv{\xx}{\typ_x},\env_2}{\loccx_i}{\dynenv}{\ee[\val/\xx]}
{\typ}
{\loccx_o}
{\dynenv}.
By inversion:
(2) \typing{\varcx}{\env_1,\mapstoenv{\xx}{\typ_x},\env_2}{\loccx_i}{\dynenv}{\ee[\val/\xx]}
                {\typ_1}
                {\loccx}
                {\dynenv},
(3) \subtyping{\typ_1}{\typ}, and
(4) \loccxinc{\varcx}{\elftcx}{\llftcx}{\loccx}{\loccx_o}.
By inductive hypothesis on (2):
(5) \typing{\varcx}{\env_1,\env_2}{\loccx_i}{\dynenv}{\ee[\val/\xx]}
                {\typ_1}
                {\loccx}
                {\dynenv}.
By (5), (3), (4), and rule \tsub, we conclude the proof.
\item \textbf{Rule \tlet:}
(1) \typing{\varcx}{\env_1,\mapstoenv{\xx}{\typ_x},\env_2}{\loccx_i}{\dynenv}{\blet{\xx}{\ee_{\xx}}{\ee}}{\typ}{\loccx_o}{\dynenv_o}.
By inversion we get
(2) \typing{\varcx}{\env_1,\mapstoenv{\xx}{\typ_x},\env_2}{\loccx_i}{\dynenv}{\ee_{\xx}}{\typ_{\xx}}{\loccx}{\dynenv},
(3) \typing{\varcx}{\env_1,\mapstoenv{\xx}{\typ_x},\env_2,\mapstoenv{\xx}{\typ_\xx}}{\loccx}{\dynenv}{\ee}{\typ}{\loccx_o}{\dynenv_o}, and
(4) $\xx \not \in \dom{\env_1,\mapstoenv{\xx}{\typ_x},\env_2}$.
By inductive hypothesis on (2) and (3) we get:
(5) \typing{\varcx}{\env_1,\env_2}{\loccx_i}{\dynenv}{\ee_{\xx}[\val/\xx]}{\typ_{\xx}}{\loccx}{\dynenv} and
(6) \typing{\varcx}{\env_1,\env_2,\mapstoenv{\xx}{\typ_\xx}}{\loccx}{\dynenv}{\ee[\val/\xx]}{\typ}{\loccx_o}{\dynenv_o}.
By (7), we get  $\xx \not \in \dom{\env_1,\env_2}$.
By (5)-(7) and rule \tlet we conclude the proof.

\item \textbf{Rule \tnew:}
(1) \typing{\varcx}{\env_1,\mapstoenv{\xx}{\typ_x},\env_2}{\loccx_i}{\dynenv}{\blet{\yy}{\new{\lvar}}{e}}{\typ}{\loccx_o}{\dynenv}.
By inversion:
(2) \typing{\varcx, \lvar:\sloc}
            {\env_1,\mapstoenv{\xx}{\typ_x},\env_2, \mapstoenv{\yy}{\tptr{\lvar}}}
            {\loccx_i, \mapstoowned{\lvar}{\uninit{1}}}
            {\dynenv}{\ee}{\typ}{\loccx_o}{\dynenv},
     (3) \wf{\typ},
     (4) \wf{\loccx_o}, and
     (5) $\yy \not \in \dom{\env_1,\mapstoenv{\xx}{\typ_x},\env_2}$.
By inductive hypothesis on (2):
(6) \typing{\varcx, \lvar:\sloc}
            {\env_1,\env_2, \mapstoenv{\yy}{\tptr{\lvar}}}
            {\loccx_i, \mapstoowned{\lvar}{\uninit{1}}}
            {\dynenv}{\ee[\val/\xx]}{\typ}{\loccx_o}{\dynenv}.
By (5) we get (7): $\yy \not \in \dom{\env_1,\env_2}$.
By (6), (3), (4), (7), and rule \tnew we conclude the proof.

\item \textbf{Rule \tif:}
(1) {\typing{\varcx}{\env_1,\mapstoenv{\xx}{\typ_x},\env_2}{\loccx_i}{\dynenv_i}{\bif{\ee}{\ee_1}{\ee_2}}{\typ}{\loccx}{\dynenv}}.
By inversion:
(2) \typing{\varcx}{\env_1,\mapstoenv{\xx}{\typ_x},\env_2}{\loccx_i}{\dynenv}{\ee}{\rtyp{\tbool}{\expr}}{\loccx_o}{\dynenv_o},
(3) \typing{\varcx, \expr}{\env_1,\mapstoenv{\xx}{\typ_x},\env_2}{\loccx_o}{\dynenv}{\ee_1}{\typ}{\loccx}{\dynenv}, and
(4) \typing{\varcx, \lnot \expr}{\env_1,\mapstoenv{\xx}{\typ_x},\env_2}{\loccx_o}{\dynenv}{\ee_2}{\typ}{\loccx}{\dynenv}.
By inductive hypothesis on (2) - (4):
(5) \typing{\varcx}{\env_1,\env_2}{\loccx_i}{\dynenv}{\ee[\val/\xx]}{\rtyp{\tbool}{\expr}}{\loccx_o}{\dynenv_o},
(6) \typing{\varcx, \expr}{\env_1,\env_2}{\loccx_o}{\dynenv}{\ee_1[\val/\xx]}{\typ}{\loccx}{\dynenv}, and
(7) \typing{\varcx, \lnot \expr}{\env_1,\env_2}{\loccx_o}{\dynenv}{\ee_2[\val/\xx]}{\typ}{\loccx}{\dynenv}.
The proof concludes by (5)-(7) and rule \tif.

% \item \textbf{Rule \tseq:}
% (1) \typing{\varcx}{\env_1,\mapstoenv{\xx}{\typ_x},\env_2}{\loccx_i}{\dynenv}{\bseq{\stmt}{\rexpr}}{\typ}{\loccx_o}{\dynenv_o}.
% By inversion:
% (2) \stmtyping{\varcx}{\env_1,\mapstoenv{\xx}{\typ_x},\env_2}{\loccx_i}{\dynenv}{\stmt}{\loccx_{\stmt}}{\dynenv_{\stmt}} and
% (3) \typing{\varcx}{\env_1,\mapstoenv{\xx}{\typ_x},\env_2}{\loccx_{\stmt}}{\dynenv}{\rexpr}{\typ}{\loccx_o}{\dynenv_o}.
% By case~\ref{lemma:program:substitution:stmt} on (2) and inductive hypothesis on (3):
% (4) \stmtyping{\varcx}{\env_1,\env_2}{\loccx_i}{\dynenv}{\stmt[\val/\xx]}{\loccx_{\stmt}}{\dynenv_{\stmt}} and
% (5) \typing{\varcx}{\env_1,\env_2}{\loccx_{\stmt}}{\dynenv}{\rexpr[\val/\xx]}{\typ}{\loccx_o}{\dynenv_o}.
% The proof concludes by rule \tseq.
\item \textbf{Rule \tunpack:}
Let the environment of the typing rule be
$\env_{u1},\mapstoenv{\xx_u}{\texists{\aa}{\rtyp{\tcon}{\aa}}{\expr}}, \env_{u2}$.
We split three cases depending on where the substituted variable \xx is:
\begin{itemize}
  \item $\xx \in \env_{u1}:$
  (1) $\typing{\varcx}{\env_1,\mapstoenv{\xx}{\typ_x},\env_2,\mapstoenv{\xx_u}{\texists{\aa}{\rtyp{\tcon}{\aa}}{\expr}}, \env_{u2}}
  {\loccx_i}{\dynenv}
  {\eunpack{\xx_u}{\aa}{e}}{\typ}
  {\loccx_o}{\dynenv}$.
  By inversion, (2)
  \typing{\varcx, \aa : \getsort{\tcon}, \expr}{\env_1,\mapstoenv{\xx}{\typ_x},\env_2,\mapstoenv{\xx_u}{\rtyp{\tcon}{\aa}}, \env_{u2}}
  {\loccx_i}{\dynenv}
  {\ee}{\typ}
  {\loccx_o}{\dynenv}.
  By inductive hypothesis
  (3)
  \typing{\varcx, \aa : \getsort{\tcon}, \expr}{\env_1,\env_2,\mapstoenv{\xx_u}{\rtyp{\tcon}{\aa}}, \env_{u2}}
  {\loccx_i}{\dynenv}
  {\ee[\val/\xx]}{\typ}
  {\loccx_o}{\dynenv}.
  The proof concludes by rule \tunpack, since  $(\eunpack{\xx_u}{\aa}{e})[\val/\xx] = \eunpack{\xx_u}{\aa}{e[\val/\xx]}$.
  \item $\xx  = \xx_u:$
  (1) $\typing{\varcx}{\env_1,\mapstoenv{\xx}{\texists{\aa}{\rtyp{\tcon}{\aa}}{\expr}}, \env_{2}}
  {\loccx_i}{\dynenv}
  {\eunpack{\xx_}{\aa}{e}}{\typ}
  {\loccx_o}{\dynenv}$.
  By inversion:
  (2)
  \typing{\varcx, \aa : \getsort{\tcon}, \expr}{\env_1,\mapstoenv{\xx}{\rtyp{\tcon}{\aa}}, \env_2}
               {\loccx_i}{\dynenv}
               {\ee}{\typ}
               {\loccx_o}{\dynenv}.
  By inductive hypothesis:
  $$(3)\
  \typing{\varcx, \aa : \getsort{\tcon}, \expr}{\env_1, \env_2}
               {\loccx_i}{\dynenv}
               {\ee[\val/\xx]}{\typ}
               {\loccx_o}{\dynenv}.$$
By hypothesis: $\typing{\varcx}{\env_1}{\loccx_i}{\dynenv}{\val}{\texists{\aa}{\rtyp{\tcon}{\aa}}{\expr}}{\loccx_i}{}$
and lemma~\ref{lemma:value-refinement}:
$$(4)\
\sortck[\varcx]{\interp{\val}}{\getsort{\tcon}}\ \text{and}\
(5)\
\lmodel{\varcx}{\expr[\interp{\val}/\aa]}.$$
By (3), (4), and lemma~\ref{lemma:type-substitution}:
$$(6)\
\typing{\varcx, \expr[\interp{\val}/\aa]}{\env_1[\interp{\val}/\aa], \env_2[\interp{\val}/\aa]}
             {\loccx_i[\interp{\val}/\aa]}{\dynenv[\interp{\val}/\aa]}
             {\ee[\val/\xx][\interp{\val}/\aa]}{\typ[\interp{\val}/\aa]}
             {\loccx_o[\interp{\val}/\aa]}{\dynenv[\interp{\val}/\aa]}.$$
By (6), (5), and lemma~\ref{lemma:condition}:
$$(7)\
\typing{\varcx}{\env_1[\interp{\val}/\aa], \env_2[\interp{\val}/\aa]}
             {\loccx_i[\interp{\val}/\aa]}{\dynenv[\interp{\val}/\aa]}
             {\ee[\val/\xx][\interp{\val}/\aa]}{\typ[\interp{\val}/\aa]}
             {\loccx_o[\interp{\val}/\aa]}{\dynenv[\interp{\val}/\aa]}.$$
By the well-formedness premise and lemmata~\ref{lemma:fv-subst} and~\ref{lemma:wf-fv}:
$$(8)\
\typing{\varcx}{\env_1, \env_2}
             {\loccx_i}{\dynenv}
             {\ee[\val/\xx][\interp{\val}/\aa]}{\typ}
             {\loccx_o}{\dynenv}$$
Which concludes the proof, since
$(\eunpack{\xx}{\aa}{e})[\val/\xx] = \ee[\val/\xx]\subst{\aa}{\interp{\val}}$.
  \item $\xx \in \env_{u2}:$ Similar to first case.
\end{itemize}

\item \textbf{Rule \tcall:}
(1) \typing{\varcx}{\env_1,\mapstoenv{\xx}{\typ_x},\env_2}{\loccx}{\dynenv}
               {\fcall{\ee}{\overline{\typ}}{\overline{\expr}}{\overline{\aval}}}
               {\applysubst{\substvar}{\typ_o}}{\applysubst{\substvar}{\loccx_{o}}, \loccx_2}{}.
By inversion, for $\substvar = \subst{\overline{\aa}}{\overline{\expr}}$:
(2) $ \forall i. \typing{\varcx}{\env_1,\mapstoenv{\xx}{\typ_x},\env_2}{\loccx}{\dynenv}{\aval_i}{\applysubst{\substvar}{\typ_{i}}}{\loccx}{}$,
(3) $ \typing{\varcx}{\env_1,\mapstoenv{\xx}{\typ_x},\env_2}{\loccx}{\dynenv}{e}
       {\polysig{\overline{\tvar}}
                {\overline{\aa: \sort}}
                {\expr}
                {\loccx_{i}}
                {\overline{\typ}}
                {\typ_o}
                {\loccx_{o}}}
      {\loccx_1, \loccx_2 }{\dynenv}$,
(4) $\loccxinc{\varcx}{}{}{\loccx_1}{\applysubst{\substvar}{\loccx_{i}}}$,
(5) $ \forall i.\sortck{\expr_i}{\sort_i}$,
(6) \lmodel{\varcx}{\applysubst{\substvar}{\expr}}, and
(7) \wf{\dynenv}.
The proof concludes by inductive hypothesis on (2) and (3) and application of the \tcall rule.

\item \textbf{Rule \ttvar:}
(1) \typing{\varcx}{\env_1,\mapstoenv{\yy}{\typ_\yy},\env_2}{\loccx}{\dynenv}{\xx}{\selfty{\typ}{\xx}}{\loccx}{\dynenv}.
By inversion: (2) $\mapstoenv{\xx}{\typ} \in \env_1,\mapstoenv{\yy}{\typ_\yy},\env_2$.
We split cases on wheather $\xx = \yy$:
\begin{itemize}
  \item \textbf{$\xx \not = \yy$:}
  $\xx[\val/\yy] = \xx$ and by (2)
  $\mapstoenv{\xx}{\typ} \in \env_1,\env_2$. So, rule \ttvar concludes the proof.
  \item \textbf{$\xx = \yy$}
  $\xx[\val/\yy] = \val$ and by (2)
  $\typ = \typ_\yy$. So, the assumption, strengthened by lemma~\ref{lemma:strengthen} with $\env_2$,
  concludes the proof.
\end{itemize}

\item \textbf{Rule \tfun:}
(1) \typing{\varcx}{\env_1,\mapstoenv{\yy}{\typ_\yy},\env_2}{\loccx}{\dynenv}
               {\vrec{\ff}{\overline{\aa}}{\overline{\xx}}{{e}}}
               {\polysig{\overline{\tvar}}{{\overline{\aa: \sort}}}
                          {\expr}{\loccx_{i}}{\overline{\typ}}
                          {\typ}{\loccx_{o}}
               }
               {\loccx}{\dynenv}.
By inversion,
(2) \typing{\varcx,\overline{\aa: \sort},\expr}
{\env_1,\mapstoenv{\yy}{\typ_\yy},\env_2,
 \overline{\xx : \typ},
 \ff: \polysig{\overline{\tvar}}{{\overline{\aa: \sort}}}
              {{\expr}}{\loccx_{i}}
              {\overline{\typ}}
              {{\typ}}
              {\loccx_{o}}
 }
{\loccx_i}{\dynenv}
{\ee}
{\typ}{\loccx_o}
{}.
By inductive hypothesis,
(3) \typing{\varcx,\overline{\aa: \sort},\expr}
{\env_1,\env_2,
 \overline{\xx : \typ},
 \ff: \polysig{\overline{\tvar}}{{\overline{\aa: \sort}}}
              {{\expr}}{\loccx_{i}}
              {\overline{\typ}}
              {{\typ}}
              {\loccx_{o}}
 }
{\loccx_i}{\dynenv}
{\ee[\val/\yy]}
{\typ}{\loccx_o}
{}.
By rule \tfun:
(4) \typing{\varcx}{\env_1,\env_2}{\loccx}{\dynenv}
               {\vrec{\ff}{\overline{\aa}}{\overline{\xx}}{{e[\val/\yy]}}}
               {\polysig{\overline{\tvar}}{{\overline{\aa: \sort}}}
                          {\expr}{\loccx_{i}}{\overline{\typ}}
                          {\typ}{\loccx_{o}}
               }
               {\loccx}{\dynenv}.
Because \yy is in the original typing environment,
by the premise of the rule it is different than \ff and $\overline{\xx}$,
so (5) $(\vrec{\ff}{\overline{\aa}}{\overline{\xx}}{{e}})[\val/\yy] = \vrec{\ff}{\overline{\aa}}{\overline{\xx}}{{e[\val/\yy]}}$,
which concludes the proof.
\item \textbf{Rules \ttrue, \tfalse, \tconstint, \ttptr, and \tumem:}
Trivial because $\ee[\val/\xx] = \ee$ and typing does not depend on the environment \env.

    % \item \textbf{Rule \tskip:}
    % \stmtyping{\varcx}{\env_1,\mapstoenv{\xx}{\typ_\xx},\env_2}{\loccx}{\dynenv}{\sskip}{\loccx}{\dynenv}.
    % By rule \tskip, trivially,
    % \stmtyping{\varcx}{\env_1,\env_2}{\loccx}{\dynenv}{\sskip\subst{\xx}{\val}}{\loccx}{\dynenv}.

    \item \textbf{Rule \tassign:}
    (1) \stmtyping{\varcx}{\env_1,\mapstoenv{\xx}{\typ_\xx},\env_2}{\loccx_i}{\dynenv}{\sassign{\place}{\ee'}}{\loccx_o}{}.
    By inversion:
    (2) \rvaltyping{\varcx}{\env_1,\mapstoenv{\xx}{\typ_\xx},\env_2}{\loccx_i}{\dynenv}{\ee'}{\typ_v}{\loccx_o},
    (3) \pltyping{\varcx}{\env_1,\mapstoenv{\xx}{\typ_\xx},\env_2}{\loccx_i}{\dynenv}{\place}{\tref{\mut}{\typ}}{\loccx_i}, and
    (4) \subtyping{\typ_v}{\typ}.
    By inductive hypothesis on (2) and (3):
    (5) \rvaltyping{\varcx}{\env_1,\env_2}{\loccx_i}{\dynenv}{\rval\subst{\xx}{\ee'}}{\typ_v}{\loccx_o},
    (6) \pltyping{\varcx}{\env_1,\env_2}{\loccx_i}{\dynenv}{\place\subst{\xx}{\ee'}}{\tref{\mut}{\typ}}{\loccx_i}.
    The proof concludes by rule (5), (6), (4), and \tassign.

    \item \textbf{Rule \tassignstrg:}
    (1) \stmtyping{\varcx}{\env_1,\mapstoenv{\xx}{\typ_\xx},\env_2}{\loccx_i}{\dynenv}{\sassign{\place}{\ee'}}{\loccx_o[\loc \mapsto \typ]}{}.
    By inversion:
    (2) \rvaltyping{\varcx}{\env_1,\mapstoenv{\xx}{\typ_\xx},\env_2}{\loccx_i}{\dynenv}{\ee'}{\typ}{\loccx_o} and
    (3) \pltyping{\varcx}{\env_1,\mapstoenv{\xx}{\typ_\xx},\env_2}{\loccx_i}{\dynenv}{\place}{\tptr{\loc}}{\loccx_i}.
    By inductive hypothesis on (2) and (3):
    (4) \rvaltyping{\varcx}{\env_1,\env_2}{\loccx_i}{\dynenv}{\rval\subst{\xx}{\ee'}}{\typ}{\loccx_o} and
    (5) \pltyping{\varcx}{\env_1,\env_2}{\loccx_i}{\dynenv}{\place\subst{\xx}{\ee'}}{\tptr{\loc}}{\loccx_i}.
    The proof concludes by (4), (5), and rule \tassignstrg.

    \item \textbf{Rules \tstrgrebor, \tstrgmutrebor, \tmutmutrebor and \tshrrebor} The proof goes by case splitting on the rules,
inversion, application of the inductive hypothesis, and application of the respective rule.

\end{itemize}
\end{proof}

% \begin{lemma}[Existential Values]\label{existential:values}
% If $\typing{\varcx}{\env_1}{\loccx}{\dynenv}{\val}{\texists{\aa}{\rtyp{\tcon}{\aa}}{\expr}}{\loccx}{}$
% then
% \sortck[\varcx]{\interp{\val}}{\getsort{\tcon}}
% and
% \lmodel{\varcx}{\expr[\interp{\val}/\aa]}.
% \end{lemma}
% \begin{proof}
%     Let {\tcon = \tint: }
%     By lemma~\ref{lemma:canonical}, $\val = \interp{\val} = n$, for some $n \in \mathbb{Z}$.
%     Thus, \sortck[\varcx]{n}{\getsort{\tint}} holds.
%     Since subtyping is reflexive and transitive (lemmata\ref{lemma:subtype:trans} and~\ref{lemma:subtype:refl}),
% the value derivation tree was the following:
% $$
% \inferrule*[Right=\tsub]
%         {
%           {\inferrule*[Right=\tconstint]
%           {}
%           {\typing{\varcx}{\env}{\loccx}{\dynenv}{n}{\rtyp{\tint}{n}}{\loccx}{\dynenv}}} \\
%           \\
%             \subtyping{\rtyp{\tint}{n}}{\texists{\aa}{\rtyp{\tcon}{\aa}}{\expr}} \\
%             \loccxinc{\varcx}{\elftcx}{\llftcx}{\loccx}{\loccx}\\
%         }
%         {
%             \typing{\varcx}{\env}{\loccx_i}{\dynenv}{n}
%                 {\texists{\aa}{\rtyp{\tcon}{\aa}}{\expr}}
%                 {\loccx}
%                 {\dynenv}
%         }
% $$
% Thus, by inversion \subtyping{\rtyp{\tint}{n}}{\texists{\aa}{\rtyp{\tcon}{\aa}}{\expr}}.
% By inverting the rule \subexists
% we get the requirement \entailment{\varcx}{\expr[n/\aa]}.

% The proof is the same for $\tcon = \tbool$.

% \end{proof}

\begin{lemma}[Subtyping Reflexive]\label{lemma:subtype:refl}
  \subtyping{\typ}{\typ}
\end{lemma}
\begin{proof}
By induction on the structure of \typ:
\begin{itemize}
  \item $\typ \equiv \rtyp{\tcon}{\expr}$.
  Since, by assumption~\ref{assumption:model:reflexive} \entailment{\varcx}{\expr = \expr},
  by rule \subrtyp we get
  \subtyping{\rtyp{\tcon}{\expr}}{\rtyp{\tcon}{\expr}}.
  \item $\typ \equiv \texists{\aa}{\rtyp{\tcon}{\aa}}{\expr}$.
  By assumption~\ref{assumption:model:identity}, we have
  (1) \entailment{\varcx, \aa:\getsort{\tcon}, \expr}{\expr}.
  By lemma~\ref{lemma:subst:idvar}, we have:
  (2) \entailment{\varcx, \aa:\getsort{\tcon}, \expr}{\expr\subst{\aa}{\aa}}.
  By (2) and rule \subexists,
  (3) \subtyping[\varcx, \aa:\getsort{\tcon}, \expr]
            {\rtyp{\tcon}{\aa}}{\texists{\aa}{\rtyp{\tcon}{\aa}}{\expr}}.
  By (3) and rule \subunpack, we conclude the proof.
  \item $\typ \equiv \tptr{\loc}$. Trivially, by rule \subptr.
  \item $\typ \equiv \uninit{n}$. Trivially, by rule \submem.
  \item $\typ \equiv \tbor{\lft}{\shr}{\typ'}$.
  By inductive hypothesis on $\typ'$ and rule \subborshr.
  \item $\typ \equiv \tbor{\lft}{\mut}{\typ'}$.
  By inductive hypothesis on $\typ'$ and rule \subbormut.
  \item $\typ \equiv \polysig{\overline{\tvar}}
  {\overline{\aa: \sort}}
  {\expr}
  {\loccx_i}
  {\overline{\typ}}
  {\typ_o}
  {\loccx_o}$.
  By assumption~\ref{assumption:model:identity}:
  (1) \entailment{\varcx, \overline{\aa: \sort}}{\expr \Rightarrow \expr}.
  By lemma~\ref{context:reflexive}
  (2) \loccxinc
  {\varcx, \overline{\aa: \sort}}
  {\elftcx}{\llftcx}
  {\loccx_{i}}
  {\loccx_{i}} and
  (3) \loccxinc
  {\varcx, \overline{\aa: \sort}}
  {\elftcx}{\llftcx}
  {\loccx_{o}}
  {\loccx_{o}}.
  By inductive hypothesis:
  (4) $\forall i. \subtyping[\varcx, \overline{\aa: \sort}]{\typ_{i}}{\typ_{i}}$ and
  (5) \subtyping[\varcx, \overline{\aa: \sort}]{\typ_{o}}{\typ_{o}}.
  The proof concludes by (1)-(5) and rule \subfun.
\end{itemize}
\end{proof}

\begin{lemma}[Context Inclusion Reflexive]\label{context:reflexive}
  Forall \varcx and \loccx, \loccxinc{\varcx}{\elftcx}{\llftcx}{\loccx}{\loccx}.
\end{lemma}
\begin{proof}
  By rule \loccxincperm.
\end{proof}

\begin{lemma}[Strengthening]\label{lemma:strengthen}
  Let \env be an environment that does not contain any variables bound at \ee, $\env_1$, or $\env_2$.
  If \typing{\varcx}{\env_1, \env_2}{\loccx_i}{\dynenv}{\ee}{\typ}{\loccx_o}{},
  then \typing{\varcx}{\env_1, \env, \env_2}{\loccx_i}{\dynenv}{\ee}{\typ}{\loccx_o}{}.
\end{lemma}
\begin{proof}
By induction on the derivation tree.
\newline
%%% EXPRESSIONS
We split cases on the typing derivation tree:
  \begin{itemize}
      \item \textbf{Rule \tsub:}
      By inductive hypothesis and rule \tsub.
      \item \textbf{Rule \tlet:}
      (1) \typing{\varcx}{\env_1, \env_2}{\loccx_i}{\dynenv}{\blet{\xx}{\ee_{\xx}}{\ee}}{\typ}{\loccx_o}{\dynenv_o}.
      By inversion:
      (2) \typing{\varcx}{\env_1, \env_2}{\loccx_i}{\dynenv}{\ee_{\xx}}{\typ_{\xx}}{\loccx}{\dynenv},
      (3) \typing{\varcx}{\env_1, \env_2,\mapstoenv{\xx}{\typ_\xx}}{\loccx}{\dynenv}{\ee}{\typ}{\loccx_o}{\dynenv_o}, and
      (4) $\xx \not \in \dom{\env_1, \env_2}$.
      By inductive hypothesis on (2) and (3):
      (5) \typing{\varcx}{\env_1, \env, \env_2}{\loccx_i}{\dynenv}{\ee_{\xx}}{\typ_{\xx}}{\loccx}{\dynenv} and
      (6) \typing{\varcx}{\env_1, \env, \env_2,\mapstoenv{\xx}{\typ_\xx}}{\loccx}{\dynenv}{\ee}{\typ}{\loccx_o}{\dynenv_o}.
      By hypothesis and (4): (7) $\xx \not \in \dom{\env_1,\env, \env_2}$.
      By (5)-(7) and rule \tlet we conclude the proof.

      \item \textbf{Rule \tnew:}
      By inductive hypothesis, assumption, and rule \tnew.
      \item \textbf{Rule \tif:}
      By inductive hypothesis and rule \tif.
      % \item \textbf{Rule \tseq:}
      % By induction hypothesis, case~\ref{lemma:strengthen:stmt}, and rule~\tseq.
      \item \textbf{Rule \tunpack:}
      We split two cases based on the location of \xx. Both go by inductive hypothesis and rule \tunpack.
      \item \textbf{Rule \tcall:}
      By inductive hypothesis and rule \tcall.
      \item \textbf{Rule \ttvar:}
      Since the domains of the environments are disjoint,
      $\mapstoenv{\xx}{\typ} \in \env_1,\env, \env_2$.
      \item \textbf{Rule \tfun:}
      By inductive hypothesis and rule \tfun.
      \item \textbf{Rules \ttrue, \tfalse, \tconstint, \ttptr, \tumem:}
      Trivial since the rules do not depend on the typing environment.

      \item \textbf{Rules \tassign and \tassignstrg} By inductive hypothesis.

      \item \textbf{Rules \tstrgrebor, \tstrgmutrebor, \tmutmutrebor, \tshrrebor , \tderef and \tderefstrg:} By inductive hypothesis.
  \end{itemize}
\end{proof}

\begin{lemma}[Well Formedness]\label{lemma:wf}
  If \typing{\varcx}{\env}{\loccx_i}{\dynenv}{\ee}{\typ}{\loccx_o}{\dynenv}
  and \wf{\env}, \wf{\loccx_i}, \wf{\dynenv},
  then \wf{\loccx_o} and \wf{\typ}.
\end{lemma}
\begin{proof}
By induction on the type derivation trees.
\end{proof}

\begin{lemma}[Subtyping weakening]\label{lemma:varcx-subtyping-weakening}
    \quad
    \begin{enumerate}
    \item If \subtyping[\varcx_1,\varcx_2]{\typ_1}{\typ_2} then \subtyping[\varcx_1,\varcx',\varcx_2]{\typ_1}{\typ_2}.
    \item If \loccxinc{\varcx_1,\varcx_2}{}{}{\loccx_1}{\loccx_2} then \loccxinc{\varcx_1,\varcx',\varcx_2}{}{}{\loccx_1}{\loccx_2}.
    \end{enumerate}
\end{lemma}
\begin{proof}
    By mutual induction in the definition of subtyping and context inclusion generalizing over $\varcx_2$.
    \begin{itemize}
        \item \textbf{Case \subptr, \submem:} Direct by applying the rules since they do not depend on the logical context.
        \item \textbf{Case \subbormut, \subborshr:} By applying the induction hypothesis for (1)
        \item \textbf{Case \subrtyp:} By assumption~\ref{assumption:model:weakening}
        \item \textbf{Case \subunpack:} By applying the induction hypothesis for (1) picking
        $\varcx_2,\aa:\getsort{B},\expr$ for the generalized logical context.
        \item \textbf{Case \subexists:} By assumption~\ref{assumption:model:weakening}.
        \item \textbf{Case \subfun:} By inductive hypotheses and assumption~\ref{assumption:model:weakening}.
        \item \textbf{Case \loccxincperm,\loccxincweaken:} Direct by applying the rules since they do not depend on the logical context.
        \item \textbf{Case \loccxincframe, \loccxincsub:} By inductive hypotheses.
    \end{itemize}
\end{proof}

\begin{restatable}[Value refinement]{lemma}{valuerefinement}
\label{lemma:value-refinement}
Given $\typing{\varcx}{\env}{\loccx}{\dynenv}{\val}{\typ}{\loccx}{}$.
The following holds:
\begin{enumerate}
    \item If $\typ = \bty[\expr]$ then \sortck{\interp{\val}}{\getsort{\tcon}} and \entailment{\varcx}{\expr = \interp{\val}}.
    \item If $\typ = \texists{\aa}{\bty[\aa]}{\expr}$ then \sortck{\interp{\val}}{\getsort{\bty}} and \entailment{\varcx}{\expr[\interp{\val}/\aa]}
\end{enumerate}
\end{restatable}
\begin{proof}
    By induction on the typing derivation generalizing over \varcx.
    The following cases apply to values.
    \begin{itemize}
        \item \textbf{Case \tconstint,\ttrue, \tfalse:} Only the premise of (1) holds.
        The conclusion is direct since the rules assign the exact value to the index.

        \item \textbf{Case \tvecvec:} Only the premise of (1) holds.
        The conclusion is direct since the rule assigns the length of the vector as the index which
        is exactly the interpretation of vectors.

        \item \textbf{Case \tsub:} By inversion of the rule we have:
        \begin{enumerate}
            \setcounter{enumi}{2}
            \item \typing{\varcx}{\env}{\loccx}{\dynenv}{\val}{\typ'}{\loccx}{}
            \item \subtyping{\typ'}{\typ}
        \end{enumerate}
        We prove (1) and (2) separately, assuming the premise in each case:
        \begin{itemize}
            \item $\typ = \bty[\expr]$. By inversion of (4) we have two cases
            \begin{itemize}
                \item \textbf{Case \subrtyp:} (4) becomes \subtyping{\bty[\rexpr']}{\bty[\rexpr]}.
                The conclusion of (1) then follows from the premise of \subrtyp, the inductive hypotheses applied to (3) and
                Assumption~\ref{assumption:model:transitive}.

                \item \textbf{Case \subunpack:} (3) becomes
                \typing{\varcx}{\env}{\loccx}{\dynenv}{\val}{\texists{\aa}{\bty[\aa]}{\expr'}}{\loccx}{}.
                and (4) becomes \subtyping{\texists{\aa}{\bty[\aa]}{\expr'}}{\bty[\expr]}.
                By inversion of (4) we have \subtyping[\varcx,\aa:\getsort{B},\expr']{\bty[\aa]}{\bty[\expr]}, and
                again by inversion we have \entailment{\varcx,\aa:\getsort{B},\expr'}{\aa = \expr}.
                By the inductive hypothesis applied to (3) we have \entailment{\varcx}{\expr'[\interp{\val}/\aa]} and
                \sortck{\interp{\val}}{\getsort{\bty}}.
                By Lemma~\ref{lemma:existential-indexed-value} applied to (3) we have
                (5) \typing{\varcx,\aa:\getsort{B},\expr'}{\env}{\loccx}{\dynenv}{\val}{\bty[\aa]}{\loccx}{}.
                Applying the inductive hypothesis to (5) we get \entailment{\varcx,\aa:\getsort{B},\expr'}{\aa = \interp{\val}}.
                Summarizing, we have
                (a) \entailment{\varcx,\aa:\getsort{B},\expr'}{\aa = \expr},
                (b) \entailment{\varcx}{\expr'[\interp{\val}/\aa]}, and
                (c) \entailment{\varcx,\aa:\getsort{B},\expr'}{\aa = \interp{\val}}.
                We can apply Assumption~\ref{assumption:model:substitution} with (a) and (b).
                To get \entailment{\varcx,\expr'[\interp{\val}/\aa]}{\interp{\val} = \expr} and then apply
                Assumption~\ref{assumption:model:cut} to get \entailment{\varcx}{\interp{\val}=\expr} which concludes
                this part of the proof.
            \end{itemize}
            \item $\typ = \texists{\aa}{\bty[\aa]}{\expr}$. By inversion of (4) we have two cases:

            \begin{itemize}
                \item \textbf{Case \subexists:} (4) becomes \subtyping{\bty[\expr']}{\texists{\aa}{\bty[\aa]}{\expr}}.
                By inversion of (4) we have (5) \entailment{\varcx}{\expr[\expr'/\aa]}. By applying the inductive
                hypothesis to (3) we have \sortck{\interp{\val}}{\getsort{\bty}} and
                (6) \entailment{\varcx}{\expr' = \interp{\val}}.
                We conclude this part of the proof by Assumption~\ref{assumption:model:congruence}.
                \item \textbf{Case \subunpack:} (3) becomes
                \typing{\varcx}{\env}{\loccx}{\dynenv}{\val}{\texists{\aa}{\bty[\aa]}{\expr'}}{\loccx}{}
                and (4) becomes \subtyping{\texists{\aa}{\bty[\aa]}{\expr'}}{\texists{\aa}{\bty[\aa]}{\expr}}.
                By inverting (4) twice we get \entailment{\varcx,\aa:\getsort{B},\expr'}{\expr}.
                Applying the inductive hypothesis to (3) we get \entailment{\varcx}{\expr'[\interp{\val}/\aa]}
                and \sortck{\interp{\val}}{\getsort{\bty}}.
                By using Assumption~\ref{assumption:model:substitution} we get \entailment{\varcx,\expr'[\interp{\val}/\aa]}{\expr[\interp{\val}/\aa]}.
                We conclude by using Assumption~\ref{assumption:model:cut}.
            \end{itemize}
        \end{itemize}
    \end{itemize}
\end{proof}

\begin{lemma}\label{lemma:existential-indexed-value}
    If \typing{\varcx}{\env}{\loccx}{\dynenv}{\val}{\texists{\aa}{\rtyp{\tcon}{\aa}}{\expr}}{\loccx}{} then
    \typing{\varcx,\aa:\getsort{B},\expr}{\env}{\loccx}{\dynenv}{\val}{\rtyp{\tcon}{\aa}}{\loccx}{}
\end{lemma}
\begin{proof}
    By applying \tsub and using \tunpack and Lemma~\ref{lemma:varcx-typing-weakening} to prove its premises.
\end{proof}

\begin{lemma}[Logical context weakening]\label{lemma:varcx-typing-weakening}
    If \typing{\varcx_1,        \varcx_2}{\env}{\loccx_i}{\dynenv}{\ee}{\typ}{\loccx_o}{} then
       \typing{\varcx_1,\varcx',\varcx_2}{\env}{\loccx_i}{\dynenv}{\ee}{\typ}{\loccx_o}{}.
\end{lemma}
\begin{proof}
    By induction in the typing derivation generalizing over $\varcx_2$.
    Most cases follow by applying the rule directly or by the inductive hypotheses.
    The interesting cases are:
    \begin{itemize}
        \item \textbf{Case \tassign,\tshrrebor,\tstrgmutrebor,\tsub} By applying the inductive hypotheses
        and Lemma~\ref{lemma:varcx-subtyping-weakening}.
        \item \textbf{Case \tcall:} Follows from assumption~\ref{assumption:model:weakening},
        the inductive hypothesss, and Lemma~\ref{lemma:varcx-subtyping-weakening}.
    \end{itemize}
\end{proof}

\begin{lemma}[Type substitution]\label{lemma:type-substitution}
Given \sortck[\varcx_1]{\expr}{\sort} and
          \typing{\varcx_1,\aa:\sort,\varcx_2}
              {\env}
              {\loccx_i}
              {\dynenv}
              {\ee}
              {\typ}
              {\loccx_o}
              {}
          then

          \typing{\varcx_1,\varcx_2[\expr/\aa]}
              {\env[\expr/\aa]}
              {\loccx_i[\expr/\aa]}
              {\dynenv[\expr/\aa]}
              {\ee[\expr/\aa]}
              {\typ[\expr/\aa]}
              {\loccx_o[\expr/\aa]}
              {}
\end{lemma}
\begin{proof}
\begingroup
    \newcommand\indelta{\ensuremath{\varcx_1,\aa:\sort, \varcx_2}}
    \newcommand\outdelta{\ensuremath{\varcx_1,\varcx_2[\expr/\aa]}}
    \newcommand\s{[\expr/\aa]}

    By induction on the typing derivation.

    \begin{itemize}
        \item \textbf{Case \tsub:} Inverting the rules we have:
        \begin{enumerate}
            \item \typing{\indelta}{\env}{\loccx_i}{\dynenv}{\ee}{\typ_1}{\loccx}{}
            \item \subtyping[\indelta]{\typ_1}{\typ}
            \item \loccxinc{\indelta}{}{}{\loccx}{\loccx_o}
        \end{enumerate}
        We apply the inductive hypothesis to (1) and Lemma~\ref{lemma:subtyping-substitution} to (2) and (3) to get
        \begin{enumerate}
            \item \typing{\outdelta}{\env\s}{\loccx_i\s}{\dynenv\s}{\ee\s}{\typ_1\s}{\loccx\s}{}
            \item \subtyping[\outdelta]{\typ_1\s}{\typ\s}
            \item \loccxinc{\outdelta}{}{}{\loccx\s}{\loccx_o\s}
        \end{enumerate}

        \item \textbf{Case \tlet:} By inversion of the rule:
        \begin{enumerate}
            \item \typing{\indelta}{\env}{\loccx_i}{\dynenv}{\ee_x}{\typ_x}{\loccx}{}
            \item \typing{\indelta}{\env,x:\typ_x}{\loccx}{\dynenv}{\ee_x}{\typ}{\loccx_o}{}
            \item $\xx\notin \dom{\env}$
        \end{enumerate}
        Applying inductive hypothesis we get
        \begin{enumerate}
            \item \typing{\outdelta}{\env\s}{\loccx_i\s}{\dynenv\s}{\ee_x\s}{\typ_x\s}{\loccx\s}{}
            \item \typing{\outdelta}{(\env,x:\typ_x)\s}{\loccx\s}{\dynenv\s}{\ee_x\s}{\typ\s}{\loccx_o\s}{}
        \end{enumerate}
        By definition we have $(\env,x:\typ_x)\s = \env\s,x: \typ_x\s$ and $\dom{\env} = \dom{\env\s}$,
        thus we conclude by applying \tlet.

        \item \textbf{Case \tnew:} By inversion of the rule:
        \begin{enumerate}
            \item \typing{\indelta,\lvar:\sloc}{\env, \xx:\tptr{\lvar}}{\loccx_i,\lvar\mapsto\uninit{1}}{\dynenv}{\ee}{\typ}{\loccx_o}{}
            \item \wf[\indelta]{\typ}
            \item \wf[\indelta]{\loccx_o}
            \item $\xx \notin \dom{\env}$
            \item $\lvar \notin \dom{\indelta}$
        \end{enumerate}
        Applying the inductive hypothesis and Lemma~\ref{lemma:wf-substitution} we have
        \begin{enumerate}
            \item \typing{\varcx_1,(\varcx_2,\lvar:\sloc)\s}{(\env, \xx:\tptr{\lvar})\s}{(\loccx_i,\lvar\mapsto\uninit{1})\s}{\dynenv\s}{\ee\s}{\typ\s}{\loccx_o\s}{}
            \item \wf[\outdelta]{\typ\s}
            \item \wf[\outdelta]{\loccx_o\s}
        \end{enumerate}
        By (5) we have $\lvar \neq \aa$, then by definition of substitution we have
        $$
          \typing{\outdelta,\lvar:\sloc}{\env\s, \xx:\tptr{\lvar}}{\loccx_i\s,\lvar\mapsto\uninit{1}}{\dynenv\s}{\ee\s}{\typ\s}{\loccx_o\s}{}
        $$
        We conclude by applying \tnew.

        \item \textbf{Case \tif:}
        Similarly, follows by applying the inductive hypothesis and definition of substitution.

        % \item \textbf{Case \tseq} By inductive hypotheses \ref{case:type-substitution:expr} and \ref{case:type-substitution:stmt}.

        \item \textbf{Case \tunpack} By inversion of the rule:
        \begin{enumerate}
            \item \typing{\indelta}{\env_1,x:\bty[\bb],\env_2}{\loccx_i}{\dynenv}{\ee}{\typ}{\loccx_o}{}
            \item \wf[\indelta]{\typ}
            \item \wf[\indelta]{\loccx_o}
            \item $\bb \notin \dom{\indelta}$
        \end{enumerate}
        Applying the inductive hypothesis and Lemma~\ref{lemma:wf-substitution} we hve
        \begin{enumerate}
            \item \typing{\varcx_1,(\varcx_2, \bb:\sort)\s}{(\env_1,x:\bty[\bb],\env_2)\s}{\loccx_i\s}{\dynenv\s}{\ee\s}{\typ\s}{\loccx_o\s}{}
            \item \wf[\outdelta]{\typ\s}
            \item \wf[\outdelta]{\loccx_o\s}
        \end{enumerate}
        Because of (4) then $\aa\neq\bb$ and consequently we have
        \typing{\outdelta, \bb:\sort}{(\env_1,x:\bty[\bb],\env_2)\s}{\loccx_i\s}{\dynenv\s}{\ee\s}{\typ\s}{\loccx_o\s}{}.
        We conclude by applying \tunpack.

        \item \textbf{Case \tcall} By inversion of the rule:
        By induction hypothesis, Assumption~\ref{assumption:model:substitution} and
        and lemmas~\ref{lemma:subtyping-substitution}, \ref{lemma:wf-substitution} and \ref{lemma:well-sortedness-substitution}.

        \item \textbf{Case \tfun} By inversion of the rule:
        \begin{enumerate}
           \item $\ff \not \in \dom{\env}$
           \item $\forall i. \xx_i \notin \dom{\env}$
           \item $\forall i. \bb_i \notin \dom{\indelta}$
           \item \typing{\indelta,\overline{\bb: \sort},\expr'}
                        {\env,
                            \overline{\xx : \typ},
                            \ff: \polysig{\overline{\tvar}}{{\overline{\bb: \sort}}}
                                        {{\expr'}}{\loccx_{i}}
                                        {\overline{\typ}}
                                        {{\typ}}
                                        {\loccx_{o}}
                            }
                        {\loccx_i}{\dynenv}
                        {\ee}
                        {\typ}{\loccx_o}
                        {}
        \end{enumerate}
        By applying the inductive hypothesis:

        \begin{enumerate}
            \setcounter{enumi}{3}
           \item \typing{\varcx_1,(\varcx_2,\overline{\bb: \sort},\expr')\s}
                        {(\env,
                            \overline{\xx : \typ},
                            \ff: \polysig{\overline{\tvar}}{{\overline{\bb: \sort}}}
                                        {{\expr'}}{\loccx_{i}}
                                        {\overline{\typ}}
                                        {{\typ}}
                                        {\loccx_{o}}
                        )\s}
                        {\loccx_i\s}{\dynenv\s}
                        {\ee\s}
                        {\typ\s}{\loccx_o\s}
                        {}
        \end{enumerate}
        By (3) we have $b_i \neq \aa$ for all $i$ and by definition of substitution we have:
        \begin{enumerate}
            \setcounter{enumi}{3}
           \item \typing{\varcx_1,\varcx_2\s,\bb: \sort,\expr'}
                        {\env\s,
                            \overline{\xx : \typ},
                            \ff: \polysig{}{{\overline{\bb: \sort}}}
                                        {{\expr'\s}}{\loccx_{i}\s}
                                        {\overline{\typ\s}}
                                        {{\typ\s}}
                                        {\loccx_{o}\s}
                        }
                        {\loccx_i\s}{\dynenv\s}
                        {\ee\s}
                        {\typ\s}{\loccx_o\s}
                        {}
        \end{enumerate}
        We conclude by applying \tfun.

        \item \textbf{Case \ttvar,\ttrue,\tfalse,\tconstint,\tumem,\ttptr:} Direct since they apply to expressions
            closed under \varcx.
        % \item \textbf{Case \tskip:} By applying rule \tskip.

        \item \textbf{Cases \tassignstrg, \tassign, \tstrgmutrebor, \tmutmutrebor, \tstrgrebor, \tderef and \tderefstrg}
            All cases follow directly by inductive hypothesis and Lemma~\ref{lemma:subtyping-substitution}
    \end{itemize}
\endgroup
\end{proof}

\begin{lemma}[Subtyping Substitution]\label{lemma:subtyping-substitution}
Given \sortck[\varcx_1]{\expr}{\sort}, then

\begin{enumerate}[label=\roman*]
    \item\label{case:subtyping-substitution:subtyping} If \subtyping[\varcx_1,\aa:\sort,\varcx_2]{\typ_1}{\typ_2} then
          \subtyping[\varcx_1,\varcx_2[\expr/\aa]]{\typ_1[\expr/\aa]}{\typ_2[\expr/\aa]}.
    \item\label{case:subtyping-substitution:loccxinc} If \loccxinc{\varcx_1,\aa:\sort,\varcx_2}{}{}{\loccx_1}{\loccx_2} then
          \loccxinc{\varcx_1,\varcx_2[\expr/\aa]}{}{}{\loccx_1[\expr/\aa]}{\loccx2[\expr/\aa]}.
\end{enumerate}
\end{lemma}
\begin{proof}
\begingroup
\newcommand\indelta{\varcx_1,\aa:\sort,\varcx_2}
\newcommand\outdelta{\varcx_1,\varcx_2[\expr/\aa]}
\newcommand\s{[\expr/\aa]}
    By mutual induction on the derivation trees:

    \textbf{Case \ref{case:subtyping-substitution:subtyping})}

    \begin{itemize}
        \item \textbf{Case \subptr and \submem:} By applying the rule since they apply to arbitrary context.
        \item \textbf{Case \subrtyp:} By inversion of the rule we have \entailment{\indelta}{\expr_1 = \expr_2}.
        Thus, by assumption~\ref{assumption:model:substitution} we know \entailment{\outdelta}{(\expr_1 = \expr_2)\s}.
        Therefore, by definition of substitution, \entailment{\outdelta}{\expr\s = \expr_\s}.
        Applying rule \subrtyp we have \subtyping[\outdelta]{\rtyp{\bty\s}{\expr_1\s}}{\rtyp{\bty\s}{\expr_2\s}}.
        By definition of substitution
        $$
        \subtyping[\outdelta]{\bty[\expr_1]\s}{\bty[\expr_2]\s}
        $$
        which concludes this part of the proof.

        \item \textbf{Case \subunpack:} By inversion of the rule we have
        $$
        \subtyping[\indelta,\bb:\getsort{\bty},\expr']{\bty[\bb]}{\typ}
        $$
        Applying, the inductive hypothesis we get
        $$
        \subtyping[\varcx_1,(\varcx_2, \bb:\getsort{\bty},\expr')\s]{\bty[\bb]\s}{\typ\s}
        $$
        By definition of substitution and since $\bb$ must be fresh:
        $$
        \subtyping[\varcx_1,\varcx_2\s, \bb:\getsort{\bty},\expr'\s]{\bty[\bb]\s}{\typ\s}
        $$
        Now we apply rule \subunpack to get
        $$
        \subtyping[\varcx_1,\varcx_2\s]{\texists{\bb}{\bty[\bb]}{\expr'\s}}{\typ\s}
        $$
        And by definition of substitution we have
        $$
        \subtyping[\varcx_1,\varcx_2\s]{(\texists{\bb}{\bty[\bb]}{\expr'})\s}{\typ\s}
        $$
        which is the desired goal.

        \item \textbf{Case \subexists:} By inversion of the rule we have \entailment{\indelta}{\expr_2[\expr_1/\bb]}
        Thus, by Assumption~\ref{assumption:model:substitution}, \entailment{\outdelta}{\expr_2[\expr_1/\bb]\s}.
        Since $\bb$ must be fresh then $\bb \notin \fv{\expr}$ and by Lemma~\ref{lemma:substitution-composition}
        we have \entailment{\outdelta}{\expr\s[\expr_1\s/\bb]}.
        Now, applying \subexists we get:
        $$
        \subtyping[\outdelta]{\bty[\expr_1\s]}{\texists{\bb}{\bty[\bb]}{\expr_2\s}}
        $$
        Finally, by definition of substitution we get
        $$
        \subtyping[\outdelta]{\bty[\expr_1]\s}{\texists{\bb}{\bty[\bb]}{\expr_2}\s}
        $$
        which concludes this part of the proof.

        \item \textbf{\subbormut and \subborshr:} By the inductive hypothesis

        \item \textbf{\subfun:} By inversion of the rule
        \begin{enumerate}
            \item \entailment{\indelta, \overline{\bb: \sort_\bb}}{\expr_2 \Rightarrow \expr_1}
            \item \loccxinc
                    {\indelta, \overline{\bb: \sort_\bb}}
                    {\elftcx}{\llftcx}
                    {\loccx_{2i}}
                    {\loccx_{1i}}
            \item $\forall i. \subtyping[\indelta, \overline{\bb: \sort_\bb}]{\typ_{2i}}{\typ_{1i}}$
            \item \loccxinc
                    {\indelta, \overline{\bb: \sort_\bb}}
                    {}{}
                    {\loccx_{1o}}
                    {\loccx_{2o}}
            \item \subtyping[\indelta, \overline{\bb: \sort_\bb}]{\typ_{1o}}{\typ_{2o}}
        \end{enumerate}
        Applying the inductive hypotheses and Assumption~\ref{assumption:model:substitution} get get:
        \begin{enumerate}
            \item \entailment{\varcx_1,(\varcx_2, \overline{\bb: \sort_\bb})\s}{(\expr_2 \Rightarrow \expr_1)\s}
            \item \loccxinc
                    {\varcx_1,(\varcx_2, \overline{\bb: \sort_\bb})\s}
                    {}{}
                    {\loccx_{2i}\s}
                    {\loccx_{1i}\s}
            \item $\forall i. \subtyping[\varcx_1,(\varcx_2, \overline{\bb: \sort_\bb})\s]{\typ_{2i}\s}{\typ_{1i}\s}$
            \item \loccxinc
                    {\varcx_1,(\varcx_2, \overline{\bb: \sort_\bb})\s}
                    {}{}
                    {\loccx_{1o}\s}
                    {\loccx_{2o}\s}
            \item \subtyping[\varcx_1, (\varcx_2, \overline{\bb: \sort_\bb})\s]{\typ_{1o}\s}{\typ_{2o}\s}
        \end{enumerate}
        Since $\overline{\bb}$ need to be fresh we get
        \begin{enumerate}
            \item \entailment{\varcx_1,\varcx_2\s, \overline{\bb: \sort_\bb}}{(\expr_2 \Rightarrow \expr_1)\s}
            \item \loccxinc
                    {\varcx_1,\varcx_2\s, \overline{\bb: \sort_\bb}}
                    {}{}
                    {\loccx_{2i}\s}
                    {\loccx_{1i}\s}
            \item $\forall i. \subtyping[\varcx_1,\varcx_2\s, \overline{\bb: \sort_\bb}]{\typ_{2i}\s}{\typ_{1i}\s}$
            \item \loccxinc
                    {\varcx_1,\varcx_2\s, \overline{\bb: \sort_\bb}}
                    {}{}
                    {\loccx_{1o}\s}
                    {\loccx_{2o}\s}
            \item \subtyping[\varcx_1, \varcx_2\s, \overline{\bb: \sort_\bb}]{\typ_{1o}\s}{\typ_{2o}\s}
        \end{enumerate}
        We conclude by applying \subfun.
    \end{itemize}

    \textbf{Case \ref{case:subtyping-substitution:loccxinc})}

    \begin{itemize}
        \item \textbf{Case \loccxinctrans:} By inductive hypothesis \ref{case:subtyping-substitution:loccxinc}.
        \item \textbf{Case \loccxincperm:} Direct since if $\loccx'$ is a permutation of $\loccx$ then
        $\loccx'\s$  is also a permutation of $\loccx\s$.
        \item \textbf{Case \loccxincweaken:} By Lemma~\ref{lemma:substitution-concat}.
        \item \textbf{Case \loccxincframe:} By the inductive hypothesis \ref{case:subtyping-substitution:loccxinc}.
        and Lemma~\ref{lemma:substitution-concat}.
        \item \textbf{Case \loccxincsub:} By the inductive hypothesis \ref{case:subtyping-substitution:subtyping}.
    \end{itemize}
\endgroup
\end{proof}

\begingroup
\newcommand\indelta{\varcx_1,\aa:\sort,\varcx_2}
\newcommand\outdelta{\varcx_1,\varcx_2[\expr/\aa]}
\newcommand\s{[\expr/\aa]}

\begin{lemma}[Well-formedness Substitution]\label{lemma:wf-substitution}
Given \sortck[\varcx_1]{\expr}{\sort}, then

\begin{enumerate}[label=\roman*]
    \item If \wf[\indelta]{\typ} then \wf[\outdelta]{\typ\s}
    \item If \wf[\indelta]{\loccx} then \wf[\outdelta]{\loccx\s}
    \item If \wf[\indelta]{\dynenv} then \wf[\outdelta]{\dynenv\s}
\end{enumerate}
\end{lemma}
\begin{proof}
    Each one by induction on the derivation tree.
\end{proof}

\begin{lemma}[Well-sortedness Substitution]\label{lemma:well-sortedness-substitution}
If \sortck[\varcx_1]{\expr}{\sort}, \sortck[\indelta]{\expr'}{\sort'} and \wfvarcx{\varcx_1,\varcx_2}
then \sortck[\outdelta]{\expr'\s}{\sort'}
\end{lemma}
\begin{proof}
    By induction on the derivation tree applying Lemma~\ref{lemma:well-sortedness:weakening} and
    the assumption \sortck[\varcx_1]{\expr}{\sort} on the variable case.
\end{proof}

\endgroup

\begin{lemma}[Well-sortedness Weakening]\label{lemma:well-sortedness:weakening}
If \sortck[\varcx_1]{\expr}{\sort} and \wfvarcx{\varcx_1, \varcx_2} then \sortck[\varcx_2]{\expr}{\sort}.
\end{lemma}
\begin{proof}
    By induction on the derivation tree noting that if $\aa:\sort \in \varcx_1$ and $\wfvarcx{\varcx_1, \varcx_2}$ then
    $\aa:\sort \in \varcx_1, \varcx_2$.
\end{proof}

\begin{lemma}[Substitution composition]\label{lemma:substitution-composition}
    If $\aa \notin \fv{\expr_\bb}$ then $(\expr[\expr_a/\aa])[\expr_\bb/\bb] = (\expr[\expr_b/\bb])[\expr_a[\expr_\bb/\bb]/\aa]$
\end{lemma}
\begin{proof}
    By induction on the structure of $\expr$.
    The interesting case is the variable case.
    Let $\expr = c$ for some variable $c$.
    We have three cases
    \begin{itemize}
        \item $c \neq \aa \wedge c \neq \bb$: By applying the definition of substitution we get $c$ in both sides of the equality.
        \item $c = \aa$: By applying the definition of substitution on the left side of the equality we get
        $\expr_a[\expr_\bb/\bb]$.
        Applying, the definition of substitution on the right side once we get $\aa[\expr_a[\expr_\bb/\bb]/\aa]$.
        Applying it a second time we get $\expr_\aa[\expr_\bb/\bb]$.
        \item $c = \bb$: On the left side we have
        $$
        (\bb[\expr_a/\aa])[\expr_\bb/\bb] = \bb[\expr_\bb/\bb] = \expr_\bb
        $$
        On the right side we have
        $$
        (\bb[\expr_\bb/\bb])[\expr_a[\expr_\bb/\bb]/\aa] = \expr_\bb[\expr_a[\expr_\bb]/\aa]
        $$
        By the assumption $\aa \notin \fv{\expr_\bb}$ we get
        $$
        \expr_\bb[\expr_a[\expr_\bb]/\aa] = \expr_\bb
        $$
        which concludes the proof.
    \end{itemize}
\end{proof}

\begin{lemma}[Substitution Concatenation]\label{lemma:substitution-concat}
    $(\loccx_1,\loccx_2)[\expr/\aa] = \loccx_1[\expr/\aa], \loccx_2[\expr/\aa]$
\end{lemma}
\begin{proof}
    By induction on the structure of $\loccx_2$ applying the definition of substitution.
\end{proof}

\begin{lemma}[Canonical Forms Booleans]\label{lemma:canonical:bool}
  If \typing{\varcx}{\env}{\loccx_i}{\dynenv}{\val}{\typ}{\loccx_o}{} and $\typ = \tbool<\expr>$
  or $\typ = \texists{\aa}{\tbool<\aa>}{\expr'}$
  then $\val = \ctrue$ or $\val = \cfalse$.
\end{lemma}
\begin{proof}
  By induction on the typing derivation.
  The following cases apply:
  \begin{itemize}
    \item \textbf{\ttrue:} Direct since the rules only applies if $\val=\ctrue$.
    \item \textbf{\tfalse:} Direct since the rules only applies if $\val=\cfalse$.
    \item \textbf{\tsub:} By inversion of the subtyping judgment on the premise of the rule either
    \subrtyp, \subunpack or \subexists applies.
    In all cases we conclude by using the inductive hypothesis choosing either the indexed or existential case.
  \end{itemize}
\end{proof}

\begin{lemma}[Canonical Forms Ints]\label{lemma:canonical:int}
  If \typing{\varcx}{\env}{\loccx_i}{\dynenv}{\val}{\typ}{\loccx_o}{} and
  $\typ = \tint<n>$ or $\typ = \texists{\aa}{\tint<\aa>}{\expr}$
  then $\val = z$ for some $z\in\mathbb{Z}$.
\end{lemma}
\begin{proof}
  By induction on the typing derivation.
  The following cases apply:
  \begin{itemize}
    \item \textbf{\tconstint:} Direct since the rules only applies if $\val=z$.
    \item \textbf{\tsub:} By inversion of the subtyping judgment on the premise of the rule either
    \subrtyp, \subunpack or \subexists applies.
    In all cases we conclude by using the inductive hypothesis choosing either the indexed or existential case.
  \end{itemize}
\end{proof}

\begin{lemma}[Canonical Forms Pointers]\label{lemma:canonical:ptr}
\quad
\begin{enumerate}
    \item If \typing{\varcx}{\env}{\loccx_i}{\dynenv}{\val}{\tptr{\loc}}{\loccx_o}{} then $\val=\vptr{\cloc}{\ptrtag}$.
    \item If \typing{\varcx}{\env}{\loccx_i}{\dynenv}{\val}{\tref{\bormode}{\typ}}{\loccx_o}{} then $\val=\vptr{\cloc}{\ptrtag}$.
\end{enumerate}
\end{lemma}
\begin{proof}
    Both by induction on the typing derivation.
    The following cases apply
    \begin{itemize}
        \item \textbf{Case \ttptr:} Direct by the form of the rule.
        \item \textbf{Case \tsub:} By inversion of the subtyping premise in the rule \tsub either
        \subptr, \subborshr or \subbormut apply.
        In all cases we conclude by applying the inductive hypothesis.
    \end{itemize}
\end{proof}

\begin{lemma}[Canonical Forms Vectors]\label{lemma:canonical:vec}
  If \typing{\varcx}{\env}{\loccx_i}{\dynenv}{\val}{\typ}{\loccx_o}{} and if $\typ = \tvec<m>$ or $\typ = \texists{\aa}{\tvec<\aa>}{\expr}$
  then $\val = \vvec{n}{\val'}$.
\end{lemma}
\begin{proof}
  By induction on the typing derivation
  The following cases apply:
  \begin{itemize}
    \item \textbf{Case \tvecvec:} Direct since the rule only applies if $\val=\vvec{m}{\val'}$.
    \item \textbf{Case \tsub:} By inversion of the subtyping judgment on the premise of \tsub
    either \subrtyp, \subunpack or \subexists apply.
    In all cases we conclude by using the inductive hypothesis choosing either the indexed or existential case.
  \end{itemize}
\end{proof}

\begin{lemma}[Canonical Forms Functions]\label{lemma:canonical:fun}
  If \typing{\varcx}{\env}{\loccx_i}{\dynenv}{\val}
                {\polysig{}
                        {\overline{\aa: \sort}}
                        {\expr}
                        {\loccx}
                        {\overline{\xx : \typ}}{\typ}{\loccx_{fi}}
                }
                {\loccx_o}{},
   then either
  \begin{enumerate}
    \item $\val = \vrec{\ff}{\overline{\aa}}{\overline{\xx}}{{e}}$,
    \item $\val = \vecnew$,
    \item $\val = \vecpush$, or
    \item $\val = \vecindexmut$.
  \end{enumerate}
\end{lemma}
\begin{proof}
  By induction on the typing derivation.
  The following cases apply:
  \begin{itemize}
    \item \textbf{Case \tfun:} In this case (1) holds.
    \item \textbf{Case \tvecnew} In this case (2) holds.
    \item \textbf{Case \tvecpush} In this case (3) holds.
    \item \textbf{Case \tvecindexmut} In this case (4) holds.
    \item \textbf{Case \tsub:} By inversion of the subtyping judgment in the premise of the rule
    \tsub we have that only \subfun applies.
    We conclude by applying the inductive hypothesis.
  \end{itemize}
\end{proof}

\clearpage
\subsection{Lemmata about memory events}
\begin{lemma}[Allocation event]\label{lemma:event:alloc}
If
\begin{itemize}
  \item \statetyping[\varcx][\loccx][\dynenv]{\hp}{\sbstate_i} and
  \item \transnew{\sbstate_i}{\sbstate_o}
\end{itemize}
then

\statetyping[\varcx][\loccx,\mapstoowned{\cloc}{\uninit{1}}][\dynenv,\mapstoowned{(\cloc, \ptrtag)}{\tptr{\cloc}}]{\hp\hbind{\cloc}{\poison}}{\sbstate_o}
\end{lemma}
\begin{proof}
    Since \transnew{\sbstate_i}{\sbstate_o} we know by inversion of \osdealloc that $\cloc\notin\dom{\sbstate_i\dotstacks}$.
    Then, by definition of \statetyping[\varcx][\loccx][\dynenv]{\hp}{\sbstate_i}, we have that $\cloc\notin\dom{\hp}$,
    consequently the update does not invalidate any of the other locations.
    We also have by \tumem that \valtyping{\varcx}{\emptyset}{\emptyset}{\dynenv}{\poison}{\uninit{1}}.
    It remains to show that
    \stacktyping[\varcx][\dynenv,(\cloc,\ptrtag)\mapsto\tptr{\cloc}]{\shr}{\cloc}{(\unique, \ptrtag, \bot)}{\uninit{1}}
    which follows directly by the definition of well-typed stacks.
\end{proof}

\begin{lemma}[Strong-Reborrow event]\label{lemma:event:strg-rebor}
If
\begin{itemize}
    \item \statetyping[\varcx][\loccx][\dynenv]{\hp}{\sbstate_i},
    \item $\dynenv(\cloc, \ptrtag) = \tptr{\cloc}$ and
    \item \transreborrow{\sbstate_i}{\cloc}{\ptrtag}{\ptrtag'}{\SbRef{\mut}}{\sbstate_o}
\end{itemize}
then

\statetyping[\varcx][\loccx][\dynenv,\mapstoowned{(\cloc,\ptrtag')}{\tptr{\cloc}}]{\hp}{\sbstate_o}
\end{lemma}
\begin{proof}
    Since \transreborrow{\sbstate_i}{\cloc}{\ptrtag}{\ptrtag'}{\SbRef{\mut}}{\sbstate_o}
    we know that $\sbstate_o\dotstacks(\cloc)$ must contain $(\unique, \ptrtag', \_)$ at the top
    followed by $(\unique, \ptrtag, \_)$.
    Since \statetyping[\varcx][\loccx][\dynenv]{\hp}{\sbstate_i} and $\dynenv(\cloc,\ptrtag)=\tptr{\cloc}$,
    then \hpstrg must have been used to derive the prefix of the stack was well-typed, thus \hpstrg also holds
    if we add $(\unique, \ptrtag', \_)$ to the top of the stack.
\end{proof}

\begin{lemma}[Weaken-Reborrow event]\label{lemma:event:weaken-rebor}
If
\begin{itemize}
    \item \subtyping{\loccx(\cloc)}{\typ},
    \item $\dynenv(\cloc, \ptrtag) = \tptr{\cloc}$,
    \item \statetyping[\varcx][\loccx][\dynenv]{\hp}{\sbstate_i} and
    \item \transreborrow{\sbstate_i}{\cloc}{\ptrtag}{\ptrtag'}{\SbRef{\mut}}{\sbstate_o}
\end{itemize}
then

$\statetyping[\varcx][\loccx[\cloc\mapsto\typ]][\dynenv,\mapstoowned{(\cloc,\ptrtag')}{\tref{\mut}{\typ}}]{\hp}{\sbstate_o}$
\end{lemma}
\begin{proof}
    Similar to Lemma~\ref{lemma:event:strg-rebor} we know that $\sbstate_o\dotstacks(\cloc)$ must
    contain $(\unique, \ptrtag', \_)$ at the top followed by $(\unique, \ptrtag, \_)$.
    We can apply \hptracked to show the heaplet is well-typed after the update applying
    \hpmut to show the stack is well typed.
    Let $\dynenv' = \dynenv,\mapstoowned{(\cloc,\ptrtag')}{\tref{\mut}{\typ}}  $
    It suffices to show \valtyping{\varcx}{\emptyset}{\emptyset}{\dynenv'}{\hp(\cloc)}{\typ}.
    Since $\cloc \in \loccx$ then \hptracked must have been applied to prove well-typedness of the
    initial state, therefore we have \valtyping{\varcx}{\emptyset}{\emptyset}{\dynenv}{\hp(\cloc)}{\loccx(\cloc)}.
    By Lemma~\ref{lemma:weakening} we have
    \valtyping{\varcx}{\emptyset}{\emptyset}{\dynenv'}{\hp(\cloc)}{\loccx(\cloc)} and by subsumption
    \valtyping{\varcx}{\emptyset}{\emptyset}{\dynenv'}{\hp(\cloc)}{\typ}.
\end{proof}

\begin{lemma}[Mut-Reborrow event]\label{lemma:event:mut-rebor}
If
\begin{itemize}
    \item $\dynenv(\cloc, \ptrtag) = \tref{\mut}{\typ}$
    \item \statetyping[\varcx][\loccx][\dynenv]{\hp}{\sbstate_i} and
    \item \transreborrow{\sbstate_i}{\cloc}{\ptrtag}{\ptrtag'}{\SbRef{\mut}}{\sbstate_o}
\end{itemize}
then

\statetyping[\varcx][\loccx][\dynenv,\mapstoowned{(\cloc,\ptrtag')}{\tref{\mut}{\typ}}]{\hp}{\sbstate_o}
\end{lemma}
\begin{proof}
    Since \transreborrow{\sbstate_i}{\cloc}{\ptrtag}{\ptrtag'}{\SbRef{\mut}}{\sbstate_o} we have
    that $\sbstate_o\dotstacks(\cloc)$ must contain $(\unique, \ptrtag',\_)$ at the top.
    We also know the prefix of the stack must be well-typed.
    We conclude by applying \hpmut to show the stack updated with the new item is well-typed.
\end{proof}

\begin{lemma}[Shared-Reborrow event]\label{lemma:event:shr-rebor}
If
\begin{itemize}
    \item $\dynenv(\cloc, \ptrtag) = \tref{\bormode}{\typ}$
    \item \statetyping[\varcx][\loccx][\dynenv]{\hp}{\sbstate_i} and
    \item \transreborrow{\sbstate_i}{\cloc}{\ptrtag}{\ptrtag'}{\SbRef{\shr}}{\sbstate_o}
\end{itemize}
then

\statetyping[\varcx][\loccx][\dynenv,\mapstoowned{(\cloc,\ptrtag')}{\tref{\shr}{\typ}}]{\hp}{\sbstate_o}
\end{lemma}
\begin{proof}
    By well-typedness of the input stack either \hpmut or \hpshr was applied.
    In both cases we know $\subtyping{\typ}{\typ'}$ for some $\typ'$.
    We also know the retag transition only remove items from the stack, thus the prefix of the
    output stack must also be well-typed.
    We conclude by applying \hpshr to prove the output stack is well-typed after the update.
\end{proof}

\begin{lemma}[Read event]\label{lemma:event:read}
If
\begin{itemize}
    \item $\statetyping[\varcx][\loccx][\dynenv]{\hp}{\sbstate_i}$,
    \item $\dynenv(\cloc, \ptrtag) = \tref{\bormode}{\typ}$ and
    \item \transread{\sbstate_i}{\cloc}{\ptrtag}{\sbstate_o}
\end{itemize}
then
\begin{itemize}
    \item $\valtyping{\varcx}{\emptyset}{\loccx}{\dynenv}{\hp(\cloc)}{\typ}$ and
    \item $\statetyping[\varcx][\loccx][\dynenv]{\hp}{\sbstate_o}$.
\end{itemize}
\end{lemma}
\begin{proof}
    Since \transread{\sbstate_i}{\cloc}{\ptrtag}{\sbstate_o} the stack must have a granting
    item with tag $\ptrtag$.
    Because the initial stack is well-typed then either one of \hpshr or \hpmut must have been
    used for the granting item.
    In both cases we know \subtyping{\typ'}{\typ} for some \typ'.
    In both cases we know \valtyping{\varcx}{\emptyset}{\loccx}{\dynenv}{\hp(\cloc)}{\typ'}
    because either \hptracked or \hpuntracked must apply.
    The by subsumption we know \valtyping{\varcx}{\emptyset}{\loccx}{\dynenv}{\hp(\cloc)}{\typ} which
    is the first part of the conclusion.
    The second part follows from the fact that the read access transition can only change
    \unique permissions into \disabled, and thus we can apply \hpdisabled to prove the output
    stack is well-typed.
\end{proof}

\begin{lemma}[Strong read event]\label{lemma:event:strg-read}
If
\begin{itemize}
    \item $\cloc \in \dom{\loccx}$
    \item $\statetyping[\varcx][\loccx][\dynenv]{\hp}{\sbstate_i}$,
    \item \transread{\sbstate_i}{\cloc}{\ptrtag}{\sbstate_o}
\end{itemize}
then
\begin{itemize}
    \item $\valtyping{\varcx}{\emptyset}{\loccx}{\dynenv}{\hp(\cloc)}{\loccx(\cloc)}$ and
    \item $\statetyping[\varcx][\loccx][\dynenv]{\hp}{\sbstate_o}$.
\end{itemize}
\end{lemma}
\begin{proof}
    The first part of the conclusion follows directly by the definition of well-formed heaps since
    \hptracked must apply.
    The second part follows from the fact that the read access transition can only change
    \unique permissions into \disabled, and thus we can apply \hpdisabled to prove the output
    stack is well-typed.
\end{proof}

\begin{lemma}[Weak write event]\label{lemma:event:weak-write}
If
\begin{itemize}
    \item \statetyping{\hp}{\sbstate_i},
    \item \dynenv(\cloc, \ptrtag) = \tref{\mut}{\typ},
    \item \valtyping{\varcx}{\emptyset}{\loccx}{\dynenv}{\val}{\typ}, and
    \item \transwrite{\sbstate_i}{\cloc}{\ptrtag}{\sbstate_o}.
\end{itemize}
then

\statetyping{\hp\hbind{\cloc}{\val}}{\sbstate_o}
\end{lemma}
\begin{proof}
    After the update $\sbstate_o\dotstacks(\cloc)$ must contain $(\unique,\ptrtag, \_)$ at the top.
    Because the stack was well-typed before the update by inversion of \hpmut
    we have (1) \subtyping{\typ}{\loccx(\cloc)}.
    By (1) and subsumption we have \valtyping{\varcx}{\emptyset}{\loccx}{\dynenv}{\val}{\loccx(\cloc)},
    thus we can stil use \hptracked to prove the heaplet is well-typed after the update.
    We conclude by noting that the output stack must also be well-typed because items
    are only popped from it.
\end{proof}

\begin{lemma}[Strong write event]\label{lemma:event:strg-write}
If
\begin{itemize}
    \item \statetyping{\hp}{\sbstate_i},
    \item \dynenv(\cloc, \ptrtag) = \tptr{\cloc},
    \item \valtyping{\varcx}{\emptyset}{\loccx}{\dynenv}{\val}{\typ}
    \item \transwrite{\sbstate_i}{\cloc}{\ptrtag}{\sbstate_o} and
\end{itemize}
then

\begin{itemize}
    \item \statetyping[\varcx][\loccx[\cloc\mapsto\typ]]{\hp\hbind{\cloc}{\val}}{\sbstate_o}
\end{itemize}
\end{lemma}
\begin{proof}
    After the transition, $\sbstate_o\dotstacks(\cloc)$ must contain $(\unique, \ptrtag, \_)$ at
    the top and because $\dynenv(\cloc,\ptrtag) = \tptr{\cloc}$, the output stack only contains tags
    that are mapped to pointers in \dynenv.
    Therefore, there is nothing else to prove to show the output stack is well-typed.
    Finally, the heap is well-typed because we are updating \loccx to point to the new type \typ.
\end{proof}

\subsubsection{Lemmata about Vector Memory Events}

\begin{lemma}[Vec push empty]\label{lemma:vec:push-empty}
Let
\begin{itemize}
    \item $\hp_i=\hp\hbind{\cloc}{\vvec{0}{\val'}}$ and
    \item $\hp_o=\hp\hbind{\cloc}{\vvec{1}{\vptr{\cloc'}{\ptrtag'}}}\hbind{\cloc'}{\val}$.
\end{itemize}
If
\begin{itemize}
    \item $\dynenv(\cloc, \ptrtag) = \tptr{\cloc}$
    \item \valtyping{\varcx}{\emptyset}{\emptyset}{\dynenv}{\val}{\typ},
    \item \statetyping[\varcx][\loccx][\dynenv]{\hp_i}{\sbstate_i}, and
    \item \transwrite{\sbstate_i}{\cloc}{\ptrtag}{\sbstate},
    \item \transalloc{\sbstate}{\cloc'}{\ptrtag'}{1}{\sbstate_o},
\end{itemize}
then

\statetyping
    [\varcx]
    [\loccx[\cloc \mapsto \rtyp{\tvec}{1}]]
    [\dynenv,(\cloc', \ptrtag') \mapsto \tref{\mut}{\typ}]
    {\hp_o}
    {\sbstate_o} and
\end{lemma}
\begin{proof}
    Let $\dynenv_o=\dynenv,(\cloc', \ptrtag') \mapsto \tref{\mut}{\typ}$.
    We can apply \tvecvec to show
    \typing{\varcx}{\emptyset}{\emptyset}{\dynenv_o}{\vvec{1}{\vptr{\cloc'}{\ptrtag'}}}{\rtyp{\tvec}{1}}{\emptyset}{}.
    Since \val has type \typ then the output stack will be well-typed in $\dynenv_o$.
    We conclude by using the same argument in Lemma~\ref{lemma:event:strg-write} to prove we can
    update the type of \cloc in \loccx.
\end{proof}

\begin{lemma}[Vec push]\label{lemma:vec:push}
Let
\begin{itemize}
    \item $\hp_i=\hp\hbind{\cloc}{\vvec{n}{\vptr{\cloc'}{\ptrtag'}}}\hbindn{n}{\cloc'}{\overline{\val}}$,
    \item $\hp_o=\hp\hbind{\cloc}{\vvec{n+1}{\vptr{\cloc''}{\ptrtag''}}}\hbindn{n+1}{\cloc''}{\overline{\val} \append [\val]}$, and
    \item $\dynenv_o=(\dynenv_i - (\cloc', \_))[(\cloc'' + i, \ptrtag') \mapsto \tref{\mut}{\typ} | i \in [0, n]]$.
\end{itemize}
If
\begin{itemize}
    \item \valtyping{\varcx}{\emptyset}{\emptyset}{\dynenv_i}{\val}{\typ},
    \item \transwrite{\sbstate_i}{\cloc}{\ptrtag}{\sbstate},
    \item \transdealloc{\sbstate}{\cloc'}{\ptrtag'}{n}{\sbstate'},
    \item \transalloc{\sbstate'}{\cloc''}{\ptrtag''}{n+1}{\sbstate_o},
    \item \statetyping[\varcx][\loccx][\dynenv_i]{\hp_i}{\sbstate_i}, and
    \item $\dynenv(\cloc, \ptrtag) = \tptr{\cloc}$
\end{itemize}
then

\statetyping
    [\varcx]
    [\loccx[\cloc \mapsto \rtyp{\tvec}{n + 1}]]
    [\dynenv_o]
    {\hp_o}
    {\sbstate_o} and
\end{lemma}
\begin{proof}
    By well-typedness of the input state we know
    \valtyping{\varcx}{\emptyset}{\emptyset}{\dynenv_i}{\vvec{n}{\vptr{\cloc'}{\ptrtag'}}}{\rtyp{\tvec}{n}}.
    Then, by inversion of \tvecvec we know $\dynenv_i(\cloc' + i, \ptrtag') = \tref{\mut}{\typ}$ for $i \in [0, n)$
    which together with well-typedness of the input state implies
    \valtyping{\varcx}{\emptyset}{\emptyset}{\dynenv_i}{\hp_i(\cloc + i)}{\typ}.
    Thus, since the new value \val also has type \typ, after the update all the relocated values have type \typ.
    We can then apply \tvecvec to prove \vvec{n+1}{\vptr{\cloc''}{\ptrtag''}} has type \rtyp{\tvec}{n+1} under $\dynenv_o$, and
    conclude using the same argument in Lemma~\ref{lemma:event:strg-write} to prove we can update the type of \cloc in \loccx.
\end{proof}

\begin{lemma}[Vec index mut]\label{lemma:vec:indexmut}
If
\begin{itemize}
    \item $\dynenv(\cloc, \ptrtag) = \tref{\mut}{\rtyp{\tvec}{n}}$,
    \item $\hp(\cloc) = \vvec{n}{\vptr{\cloc'}{\ptrtag'}}$,
    \item \transread{\sbstate_i}{\cloc}{\ptrtag}{\sbstate}, and
    \item \transreborrow{\sbstate}{\cloc' + i}{\ptrtag'}{\ptrtag''}{\mut}{\sbstate_o}
    \item \statetyping{\hp}{\sbstate_i}
\end{itemize}
then

\statetyping
    [\varcx]
    [\loccx]
    [\dynenv,(\cloc' + i, \ptrtag'') \mapsto \tref{\mut}{\typ}]
    {\hp}
    {\sbstate_o} and
\end{lemma}
\begin{proof}
    By Lemma~\ref{lemma:event:read} we have
    \valtyping{\varcx}{\emptyset}{\emptyset}{\dynenv}{\vvec{n}{\vptr{\cloc'}{\ptrtag'}}}{\rtyp{\tvec}{n}}.
    By inversion of \tvecvec we have $\dynenv(\cloc' + i , \ptrtag') = \tref{\mut}{\typ}$ for $i \in [0, n)$.
    We conclude by applying Lemma~\ref{lemma:event:mut-rebor}.
\end{proof}

\clearpage
\section{Vectors}
\subsection{Syntax}
\begin{figure}
\[
\begin{array}{rrcll}

    \syntaxcat{Values} &
        \val & ::=  & \dots \\
            && \mid & \vvec{n}{\val} \\
            && \mid & \vecpush \\
            && \mid & \vecnew  \\
            && \mid & \vecindexmut \\

    \syntaxcat{Base Types} &
        \tcon & ::= & \dots \mid \tvec     & \textit{integers, booleans, or user-defined} \\

\end{array}
\]
\caption{Extension of Syntax for Vectors}
\end{figure}

\subsection{Declarative judgments}
\begin{figure}
\begin{judgment}{Value typing}{\valtyping{\varcx}{\env}{\emptyset}{\dynenv}{\val}{\typ}}

    \inferrule[\tvecnew]
    {}
    {
        \valtyping{\varcx}{\env}{\emptyset}{\dynenv}{\vecnew}
        {\kw{fn}() \rightarrow \tvec}
    }

    \inferrule[\tvecpush]
    {}
    {
        \valtyping
        {\varcx}{\env}{\emptyset}{\dynenv}{\vecpush}
        {\polysig{}
            {\lvar:\sloc}{\ctrue}
            {[\mapstoowned{\lvar}{\rtyp{\tvec}{n}}]}
            {\tptr{\lvar}}
            {\uninit{1}}{[\mapstoowned{\lvar}{\rtyp{\tvec}{n + 1}}]}
        }
    }

    \inferrule[\tvecindexmut]
    {}
    {
        \valtyping
        {\varcx}{\env}{\emptyset}{\dynenv}{\vecindexmut}
        {
            \polysig
            {}
            {\aa:\sint,\bb:\sint}
            {0 \leq \bb < \aa}
            {\emptyset}
            {\tref{\mut}{\rtyp{\tvec}{\aa}}, \rtyp{\tint}{\bb}}
            {\tref{\mut}{\typ}}
            {\emptyset}
        }
    }

    \inferrule[\tvecvec]
    {
        n \geq 0 \\
        n > 0 \implies \val = \vptr{\cloc}{\ptrtag} \wedge \forall i \in [0, n).~\dynenv(\cloc + i, \ptrtag) = \tref{\mut}{\typ}
    }
    {
        \valtyping
        {\varcx}{\env}{\emptyset}{\dynenv}{\vvec{n}{\val}}
        {
            \rtyp{\tvec}{n}
        }
    }
\end{judgment}
\caption{Typing for Vectors}
\end{figure}

\subsection{Operational semantics}

\begin{judgment}{Operational Semantics}{\eval{\hp}{\sbstate}{\ee}{\hp}{\sbstate}{\rexpr}}
    \inferrule[\opvecnew]
    {
    }
    {
        \eval
          {\hp}{\sbstate}
          {\fcall{\vecnew}{}{}{}}
          {\hp}{\sbstate}
          {\vvec{0}{\poison}}
    }

    \inferrule[\opvecpush]
    {
        \transwrite{\sbstate_i}{\cloc}{\ptrtag}{\sbstate} \\\\
        \transdealloc{\sbstate}{\cloc'}{\ptrtag'}{n}{\sbstate'} \\\\
        \transalloc{\sbstate'}{\cloc''}{\ptrtag''}{n+1}{\sbstate_o} \\\\
        [\cloc'', \cloc'' + n] \mathrel{\#} \dom{\hp} \\\\
        \hp_i = \hp\hbind{\cloc}{\vvec{n}{\vptr{\cloc'}{\ptrtag'}}}\hbindn{n}{\cloc'}{\overline{\val}} \\\\
        \hp_o = \hp\hbind{\cloc}{\vvec{n+1}{\vptr{\cloc''}{\ptrtag''}}}\hbindn{n+1}{\cloc''}{\overline{\val} \append [\val]}
    }
    {
        \eval
          {\hp_i}{\sbstate_i}
          {\fcall{\vecpush}{}{\cloc}{\vptr{\cloc}{\ptrtag}, \val}}
          {\hp_o}{\sbstate_o}
          {\poison}
    }

    \inferrule[\opvecpushempty]
    {
        \transwrite{\sbstate_i}{\cloc}{\ptrtag}{\sbstate} \\\\
        \transalloc{\sbstate}{\cloc'}{\ptrtag'}{1}{\sbstate_o} \\\\
        \cloc' \notin \dom{\hp} \\\\
        \hp_i = \hp\hbind{\cloc}{\vvec{0}{\val'}} \\\\
        \hp_o = \hp\hbind{\cloc}{\vvec{1}{\vptr{\cloc'}{\ptrtag'}}}\hbind{\cloc'}{\val}
    }
    {
        \eval
          {\hp_i}{\sbstate_i}
          {\fcall{\vecpush}{}{\cloc}{\vptr{\cloc}{\ptrtag}, \val}}
          {\hp_o}{\sbstate_o}
          {\poison}
    }

    \inferrule[\opvecindexmut]
    {
        \cloc + i \in \dom{\hp} \\\\
        \transread{\sbstate_i}{\cloc}{\ptrtag}{\sbstate} \\\\
        \transreborrow{\sbstate}{\cloc' + i}{\ptrtag'}{\ptrtag''}{\mut}{\sbstate_o} \\\\
        \hp = \hp'\hbind{\cloc}{\vvec{n}{\vptr{\cloc'}{\ptrtag'}}}
    }
    {
        \eval
          {\hp}{\sbstate_i}
          {\fcall{\vecindexmut}{}{}{\vptr{\cloc}{\ptrtag}, i}}
          {\hp}{\sbstate_o}
          {\vptr{\cloc' + i}{\ptrtag''}}
    }
\end{judgment}

% \begin{judgment}{Subtyping}{\subtyping{\typ}{\typ}}
%     \inferrule
%         {}
%         {
%             \subtyping{}\tvec
%         }
% \end{judgment}

\subsection{Preservation}

\preservation*
\begin{proof}
    We add the following cases to the proof of \textbf{Rule \tcall}.

\end{proof}

\progress*
\begin{proof}
    We need to modify the proof of case \tfun by applying the extended cannonical forms lemma for
    functions (\ref{lemma:canonical:fun}) adding the following cases:
\end{proof}
